# Supplementary material for: Preference Modeling with Context-Dependent Salient Features
Source: arXiv:2002.09615 source file (2020-06-27)
Supplement: Supplementary file 1 [file all_synthetic_exp.tex]

The goal is to understand how the selection function $\tau$ effects the parameters $b^*$, $R$, $\eta, \beta,$ and $\lambda$ from Theorem \ref{thm:sampleComplexity} and hence $m_1$, $m_2$, (number of samples) and $B_m$ (upper bound on error) as well as the weak, moderate, and strong intransitivity rates, and the pairwise inconsistency rate. 

We consider five selection functions:
\begin{enumerate}
    \item Given $k \in [d]$, let the ``top $k$" selection function be the function that selects the top $k$ coordinates with the highest sample variance.
    \item Given $k \in [d]$, let the ``random exactly $k$`` selection function be the function that selects exactly $k$ coordinates for each pair of items uniformly at random.
    \item Given $p \in [0,1]$, let the ``random" selection function be the function that selects each coordinate independently with probability $p$ for each pair of items.
    \item RASV with threshold $k \in [0,1]$.
    \item RISV with threshold $k \in [0,1]$.
\end{enumerate}

When deciding how to sample $U$ and $w^*$, there are two considerations to keep in mind.

First, we need to control how large $\langle w^*, U_i^{\tau(i,j)} - U_j^{\tau(i,j)} \rangle$, i.e. $b^*$ becomes. The larger $b^*$ is, the more samples it will take to estimate $w^*$ according to Theorem \ref{thm:sampleComplexity}. Equivalently, we do not want the pairwise probabilities to be very close to 0 or 1 since controlling $b^*$ controls the range of the pairwise probabilities. The logistic function is very flat for large $b^*$, so intuitively it makes sense that more samples are required to estimate $w^*$ well in this regime.  

Second, we want to sample $U$ and $w^*$, so that for a given selection function, we can fairly compare the sample complexity across different $k$'s or $p$'s. 

It is not clear what ``fair" should mean, but for a moment, let us say that a fair comparison is when $\|U_i^{\tau(i,j)}\|$ is about the same for any $(i,j)$ regardless of $k$ or $p$. When all the features are used in each pairwise comparison, sampling each coordinate of $U$ and $w^*$ from $\sim N(0, \frac{1}{\sqrt{d}})$ is reasonable since $\mathbb{E} \|U_i^{\tau(i,j)}\|_2^2 =  \mathbb{E} \|U_i\|_2^2 = 1$, so $b^*$ will not grow as $d$ grows. The difficulty is that for a \textit{fixed} $U$ and $w^*$ but \textit{varying} $k$ or $p$, it is no longer the case that $\mathbb{E} \|U_i^{\tau(i,j)}\|_2^2 = 1$. For instance, $U_i^{\tau(i,j)}$ is $k$ sparse when $\tau$ is the top $k$ selection function, so $\mathbb{E} \|U_i^{\tau(i,j)}\|_2^2 = \frac{k}{d} < 1$.

For the experiments, we sample each coordinate of $U$ and $w^*$ from $\sim N(0, \frac{1}{\sqrt{d}})$ and then consider 4 different ways to further process $U$:

\begin{enumerate}
    \item As is: no further processing on $U$.
    \item Same b: For a given selection function and $k$ or $p$, compute $b^*$, then divide $U$ by $b^*$, so that $b^*$ is always 1.
    \item Scaled: For the ``top $k$" and ``random exactly $k$" selection functions and the ``random" selection function with $p = \frac{k}{n}$, multiply $U$ by $\frac{\sqrt{d}}{\sqrt{k}}$, so that $\mathbb{E} \|U_i^{\tau(i,j)}\|_2^2 = 1$ for top $k$ and random exactly $k$. Note that if $p = \frac{k}{n}$, then $U^{\tau(i,j)}$ on average is $k$ sparse. Furthermore, for ``top $k$" and ``random exactly $k$", some calculations show $\mathbb{E} \langle w, U_i^{\tau(i,j)} - U_j^{\tau(i,j)} \rangle = 0$ and $\mathrm{var}(\langle w, U_i^{\tau(i,j)} - U_j^{\tau(i,j)}\rangle) = \mathbb{E} \langle w, U_i^{\tau(i,j)} - U_j^{\tau(i,j)} \rangle^2 = \frac{k}{kd}= \frac{1}{d}$. 
    \item Normalized: Normalize each column of $U$. 
\end{enumerate}

In the experiments, the ambient dimension $d = 10$ and the number of items $n = 100$. The $x$-axis represents $k$ where for the random selection function $p = \frac{k}{d}$. We repeat the following 10 times for each selection function: sample $U$ and $w^*$, pre-process $U$, and use this $U$ while varying $k$. The bars represent the standard error.

Figures \ref{fig:param,top_k} - \ref{fig:param,risv} show the parameters in Theorem \ref{thm:sampleComplexity}, Figures \ref{fig:samp,topk} - \ref{fig:samp,risv} show $m_1$, $m_2$, and the bound from \ref{thm:sampleComplexity}, and finally Figures \ref{fig:sst, top k} - \ref{fig:sst, risv}  show the intransitivity and pairwise inconsistency rates.

To be clear, for Figures \ref{fig:samp,topk} - \ref{fig:samp,risv} the upper bound (i.e. plot on the left) does not include the number of samples in it, i.e. the plot shows \[ \frac{4(1 + \exp(b^*))^2}{\exp(b^*)\lambda}  \sqrt{\frac{3\beta^2\log{(2d^2)}d + 4\sqrt{d}\beta \log{(2d^2)}}{6}}\] without the $m$ term. Therefore, to ensure $\| w - w^*\|\leq 1$, the number of samples you need will be squared whatever number is on the $y$-axis in the plot.

\subsection{Parameters}

\begin{figure}
\centering

   \includegraphics[width=1\linewidth]{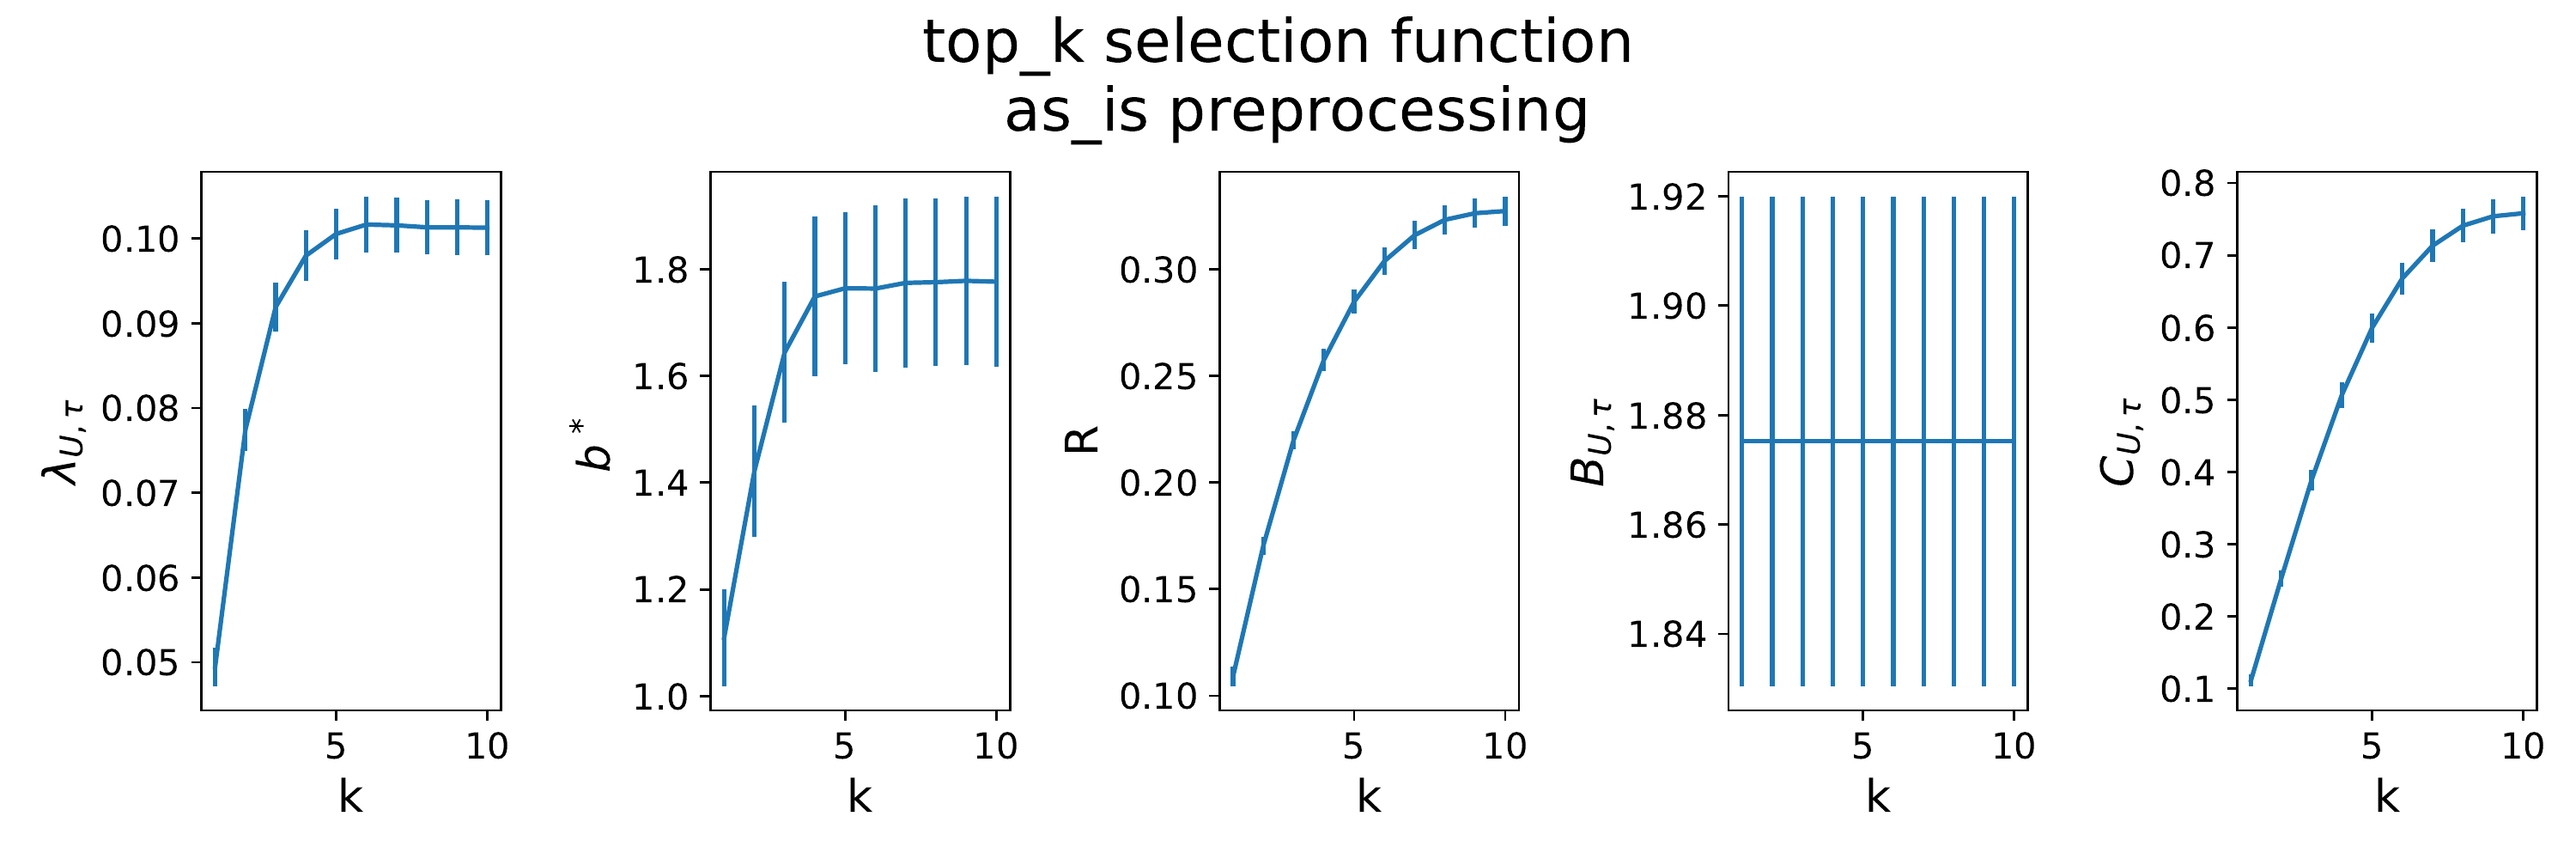}

 \includegraphics[width=1\linewidth]{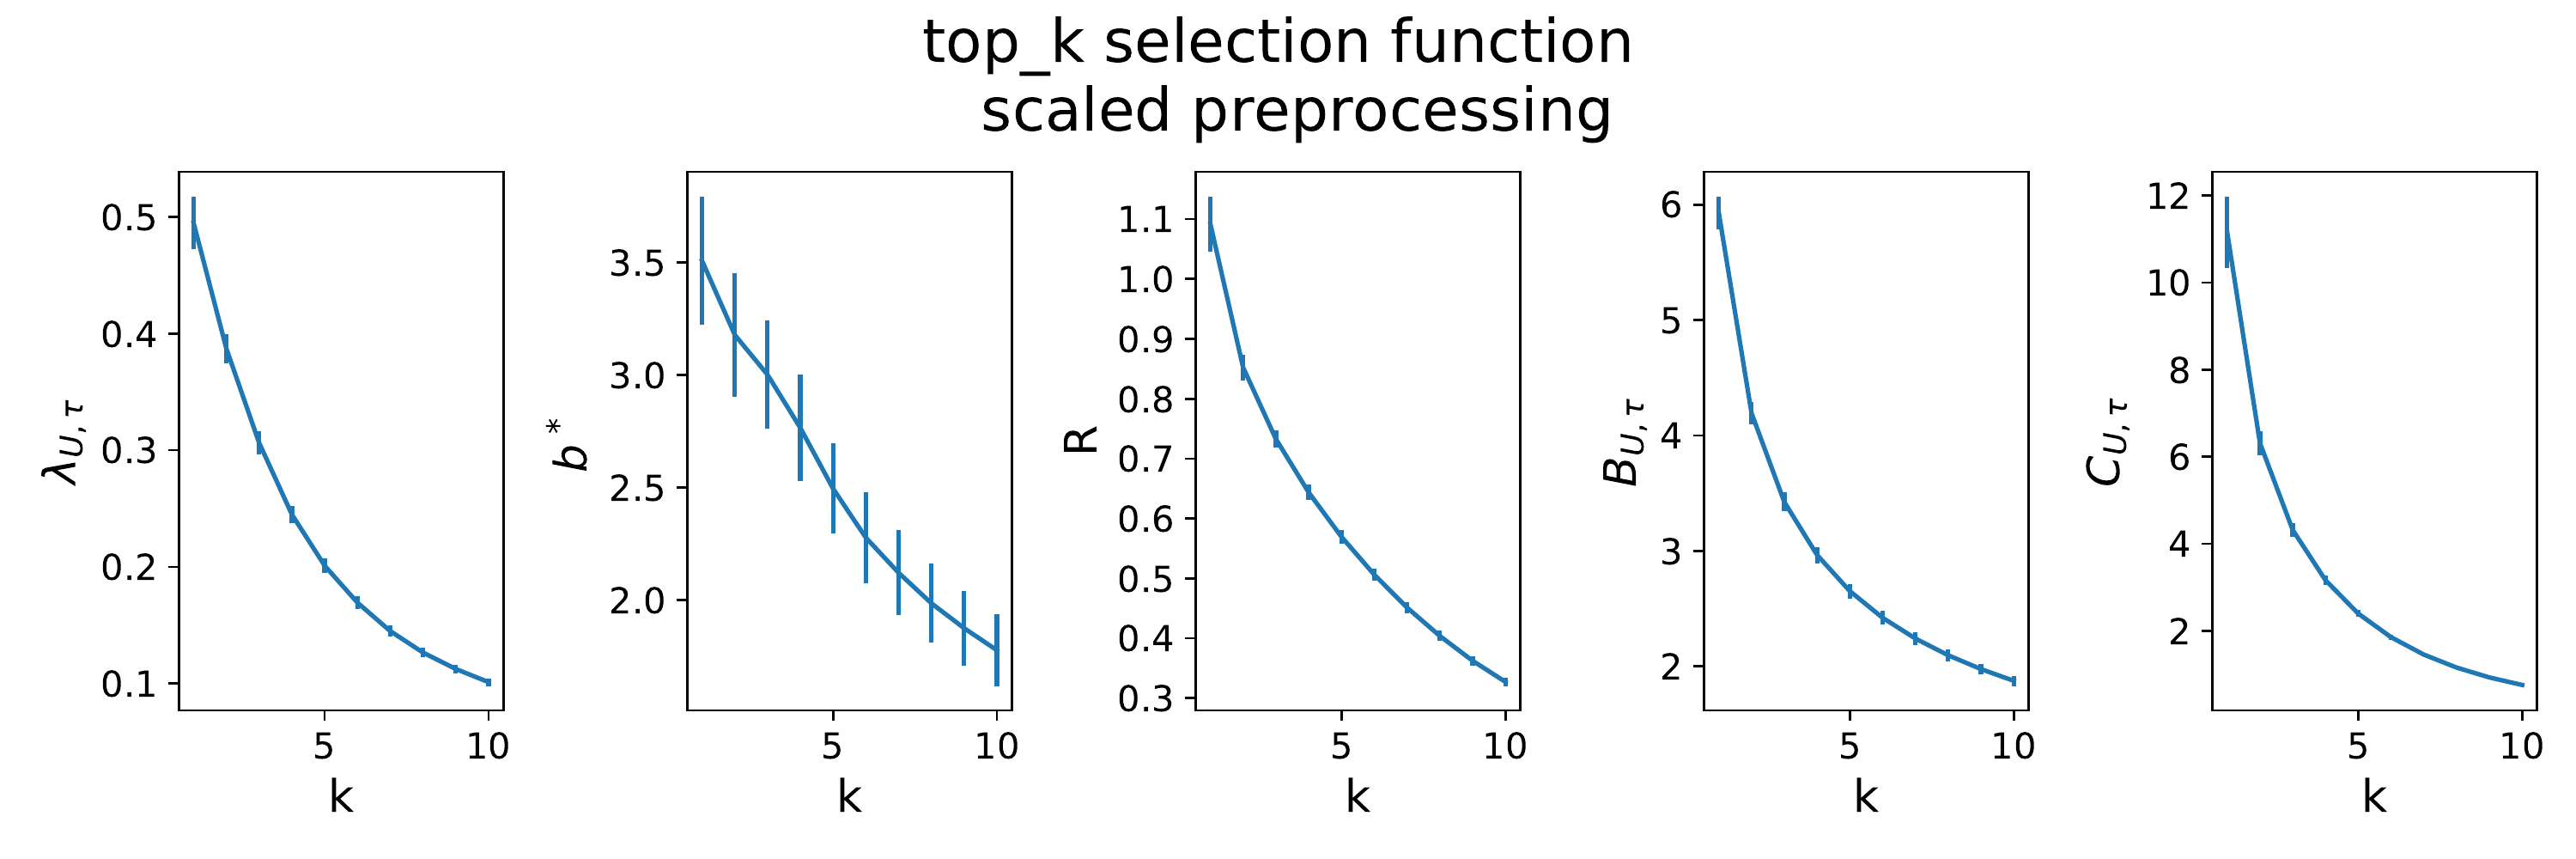}

    \includegraphics[width=1\linewidth]{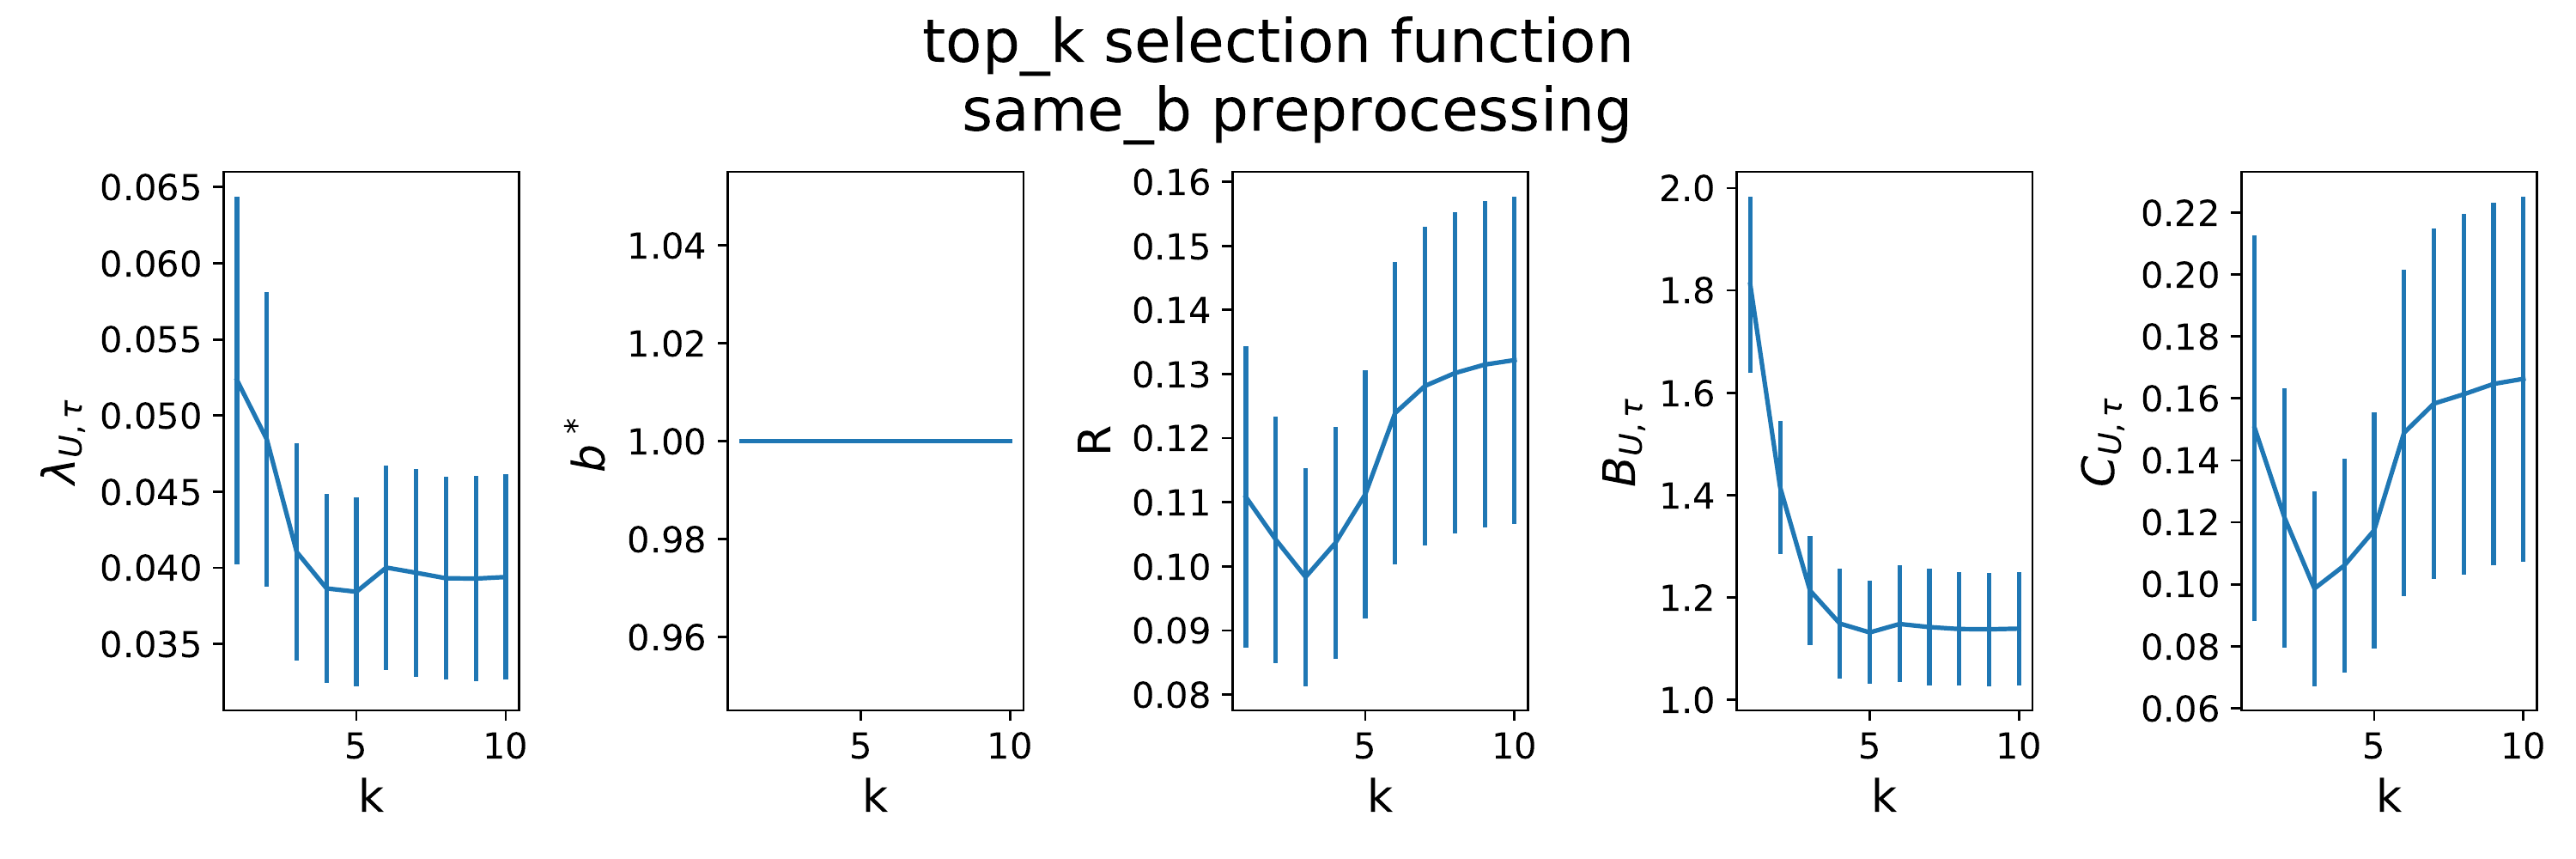}
   
 \includegraphics[width=1\linewidth]{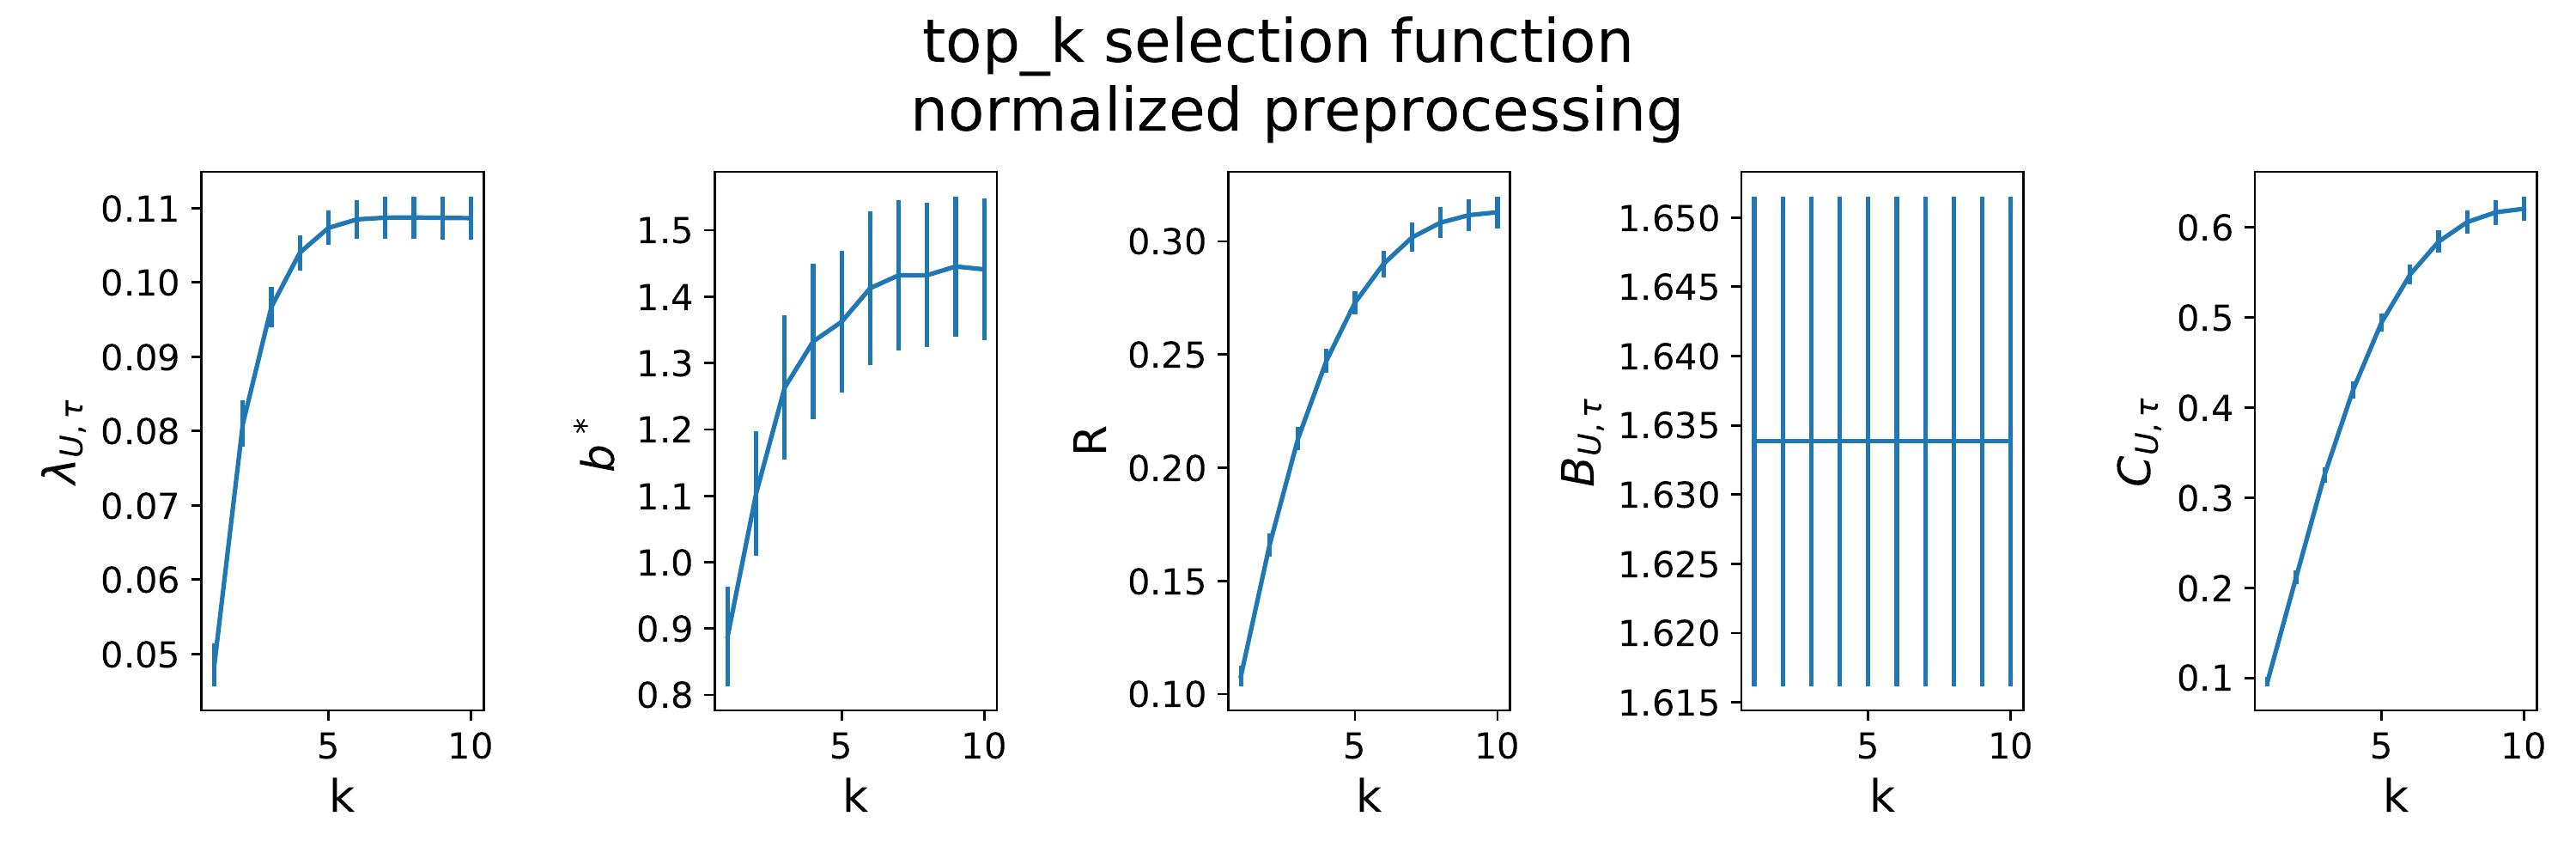}
\caption{Parameters for ``top $k$"}
\label{fig:param,top_k}
\end{figure}

\begin{figure}
\centering

   \includegraphics[width=1\linewidth]{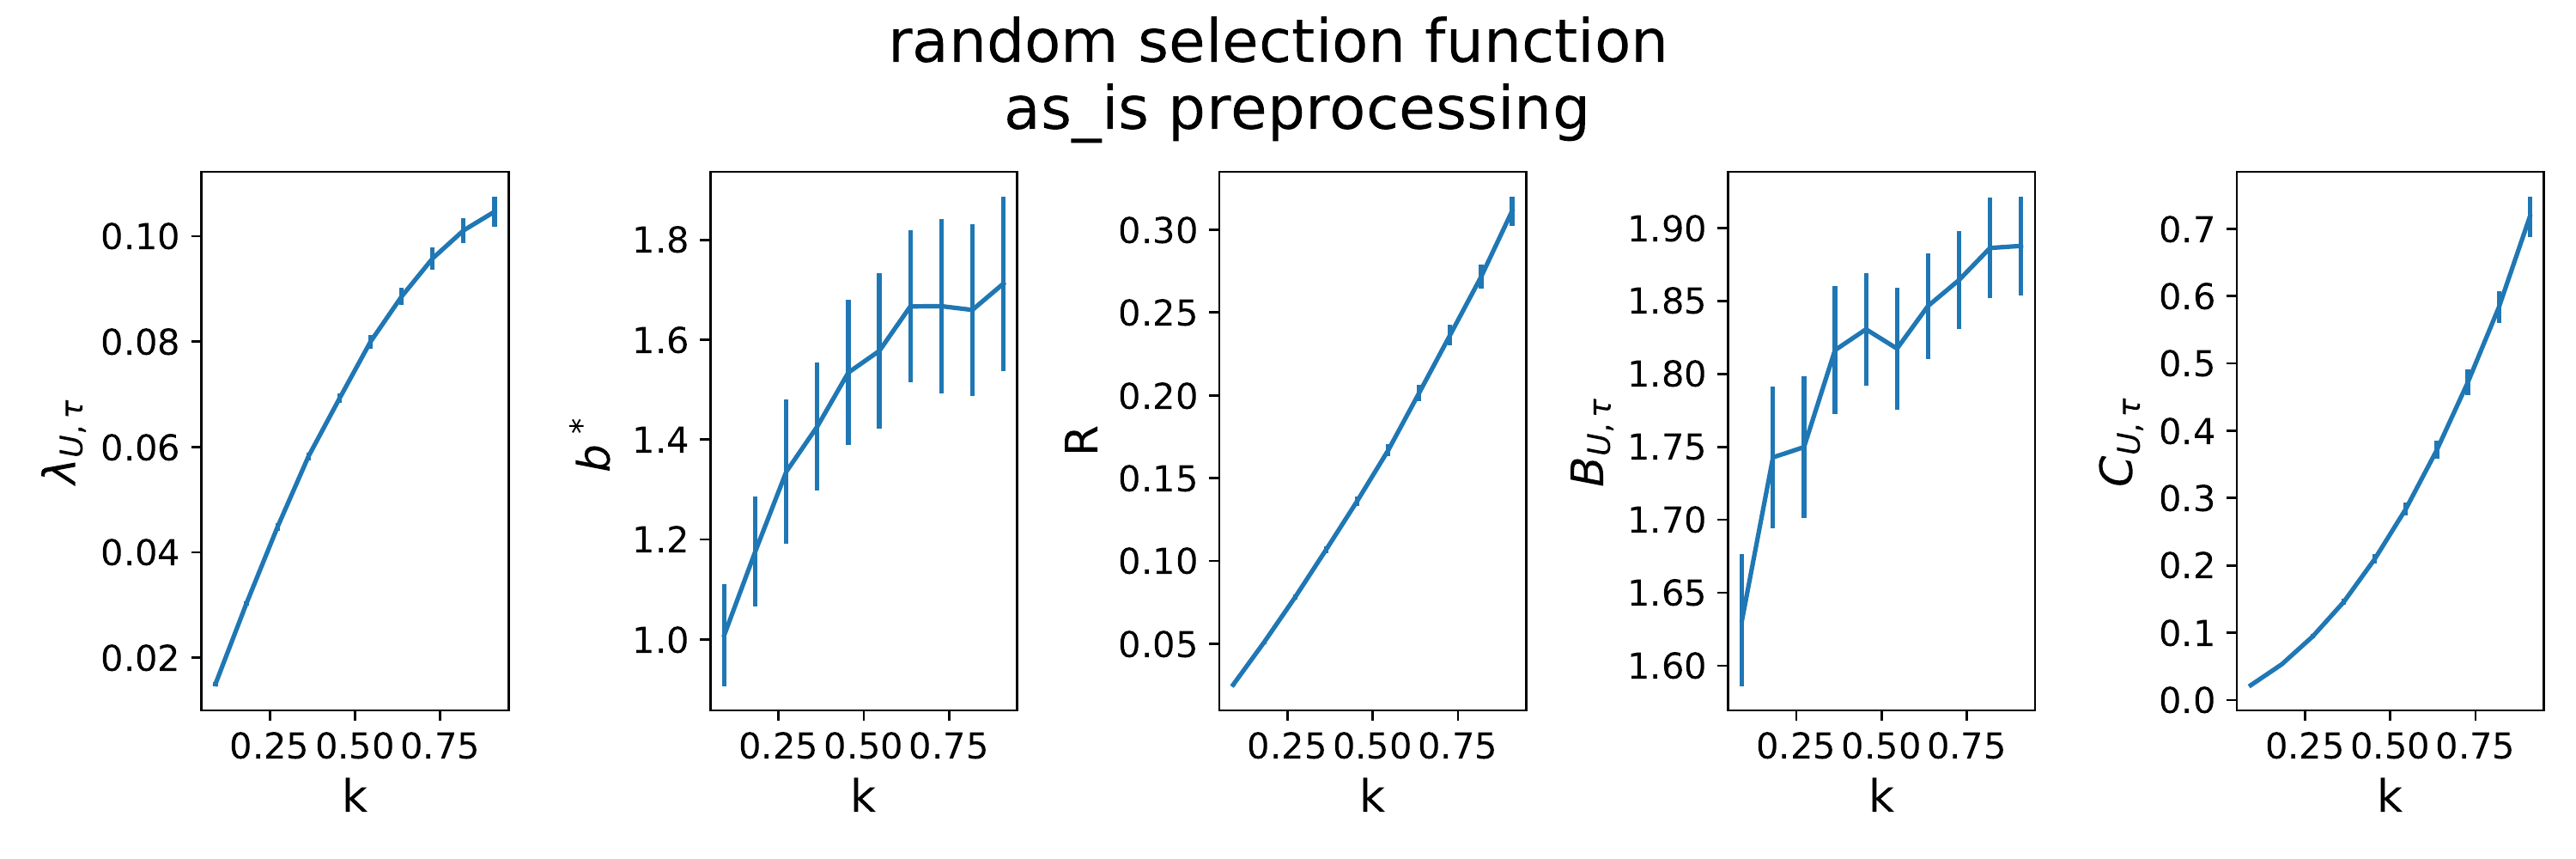}

 \includegraphics[width=1\linewidth]{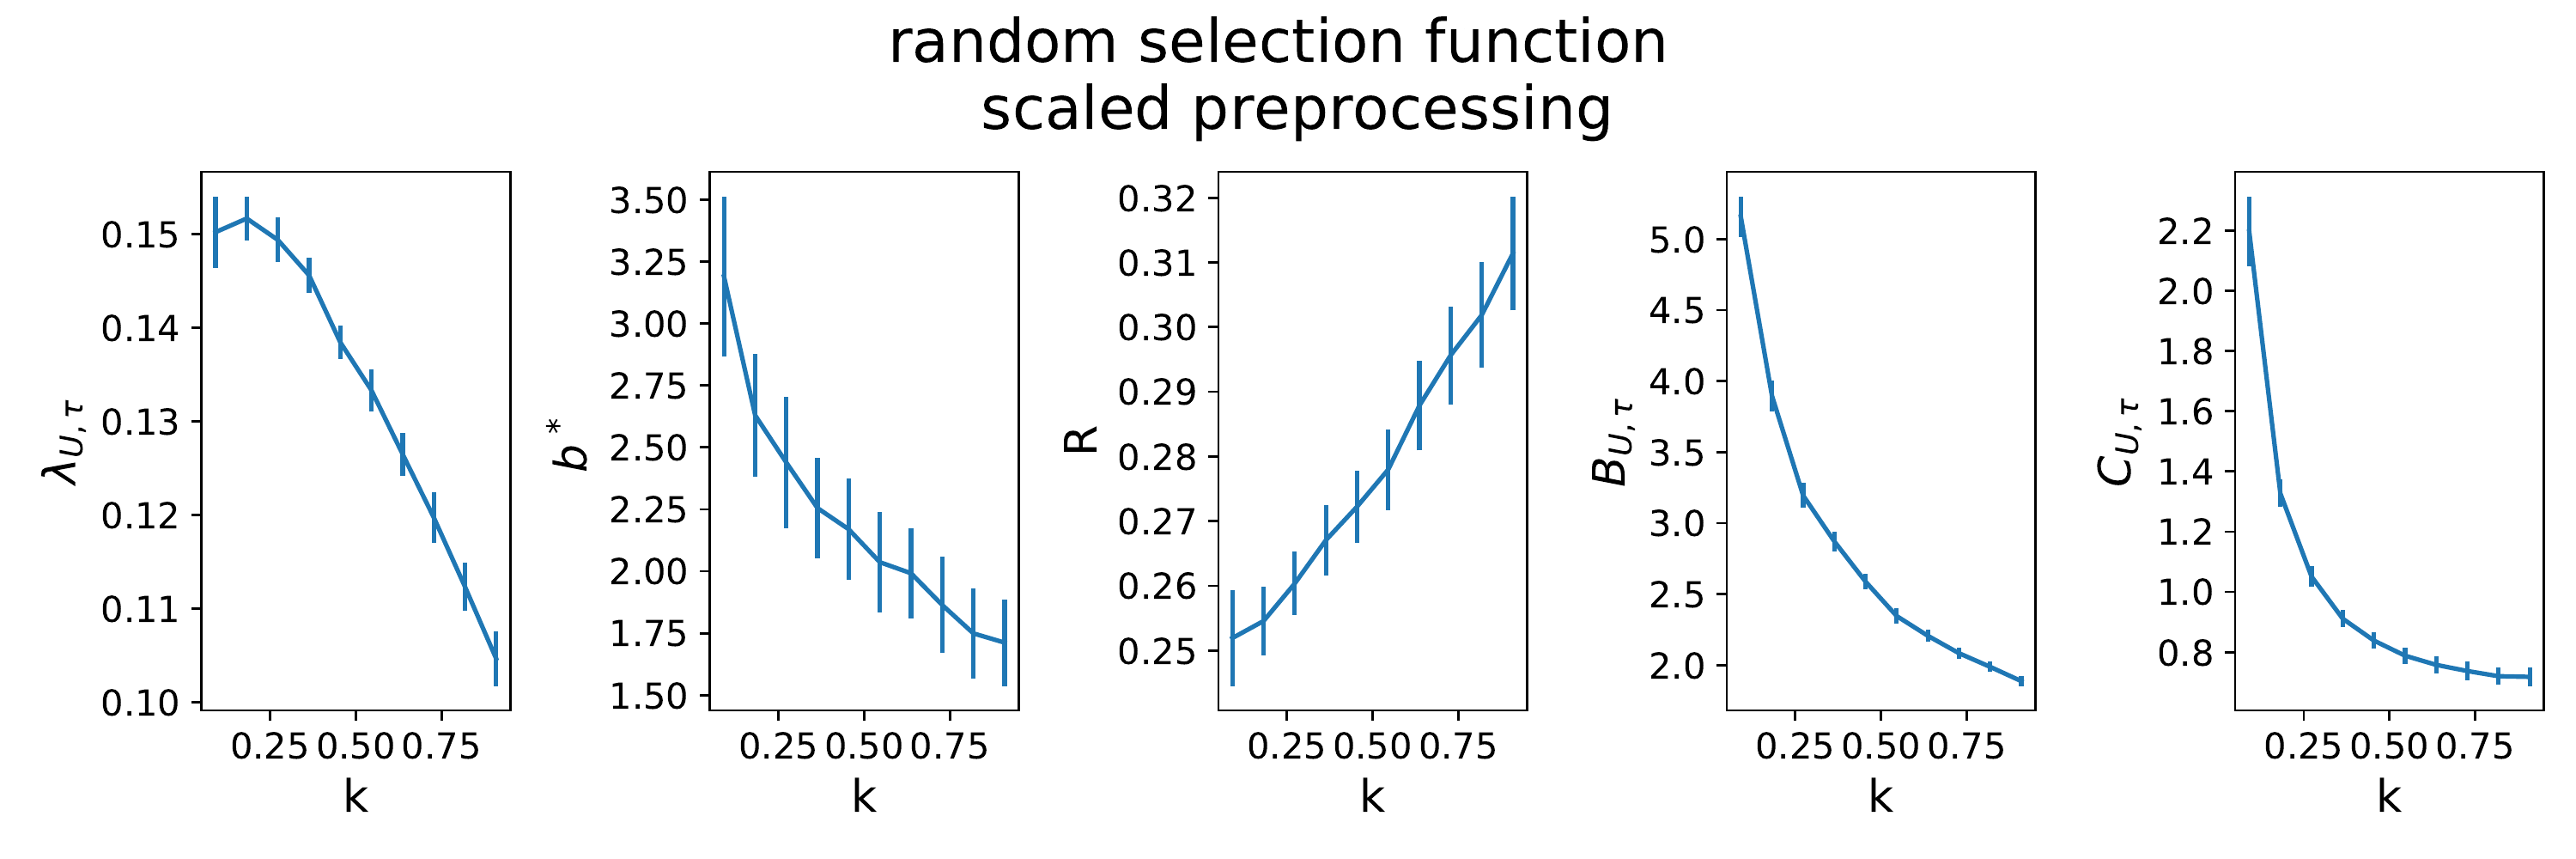}

    \includegraphics[width=1\linewidth]{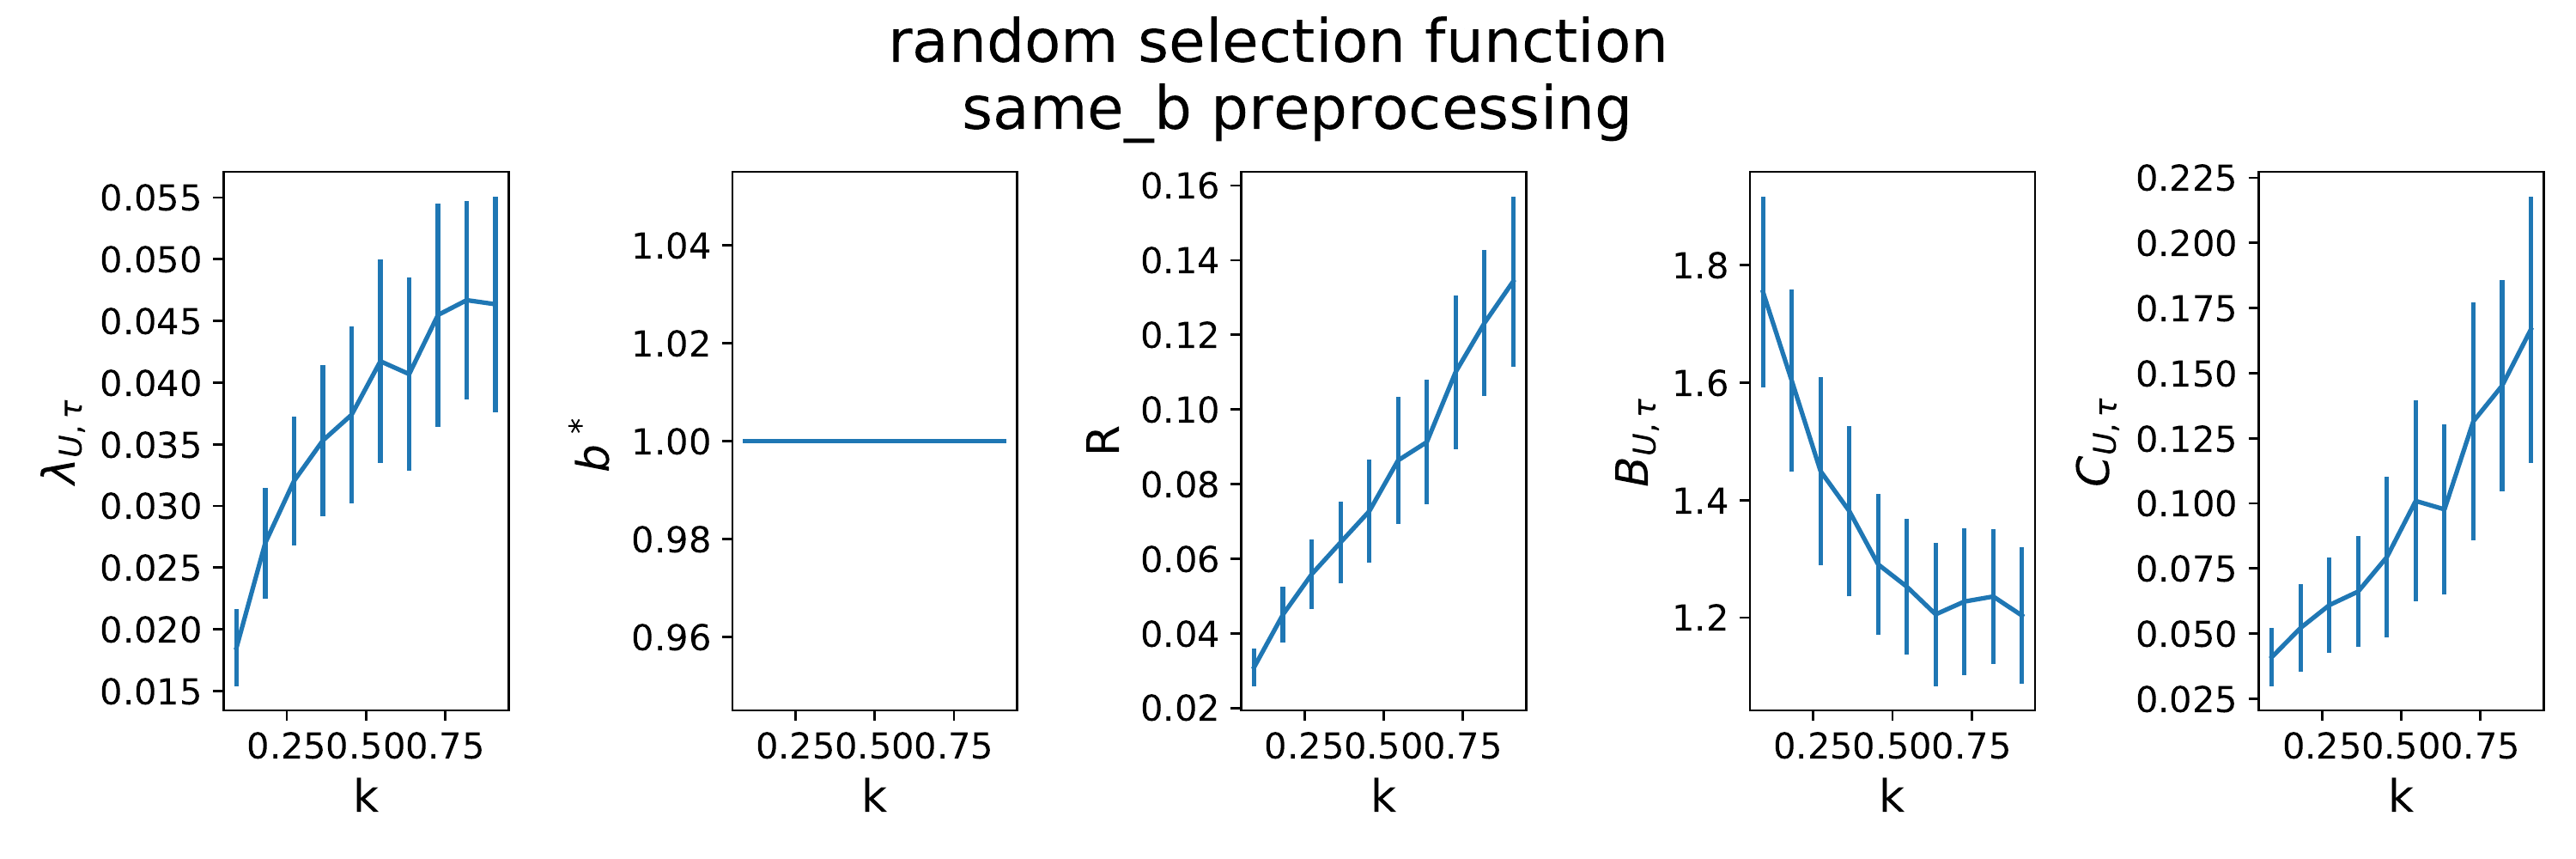}
   
 \includegraphics[width=1\linewidth]{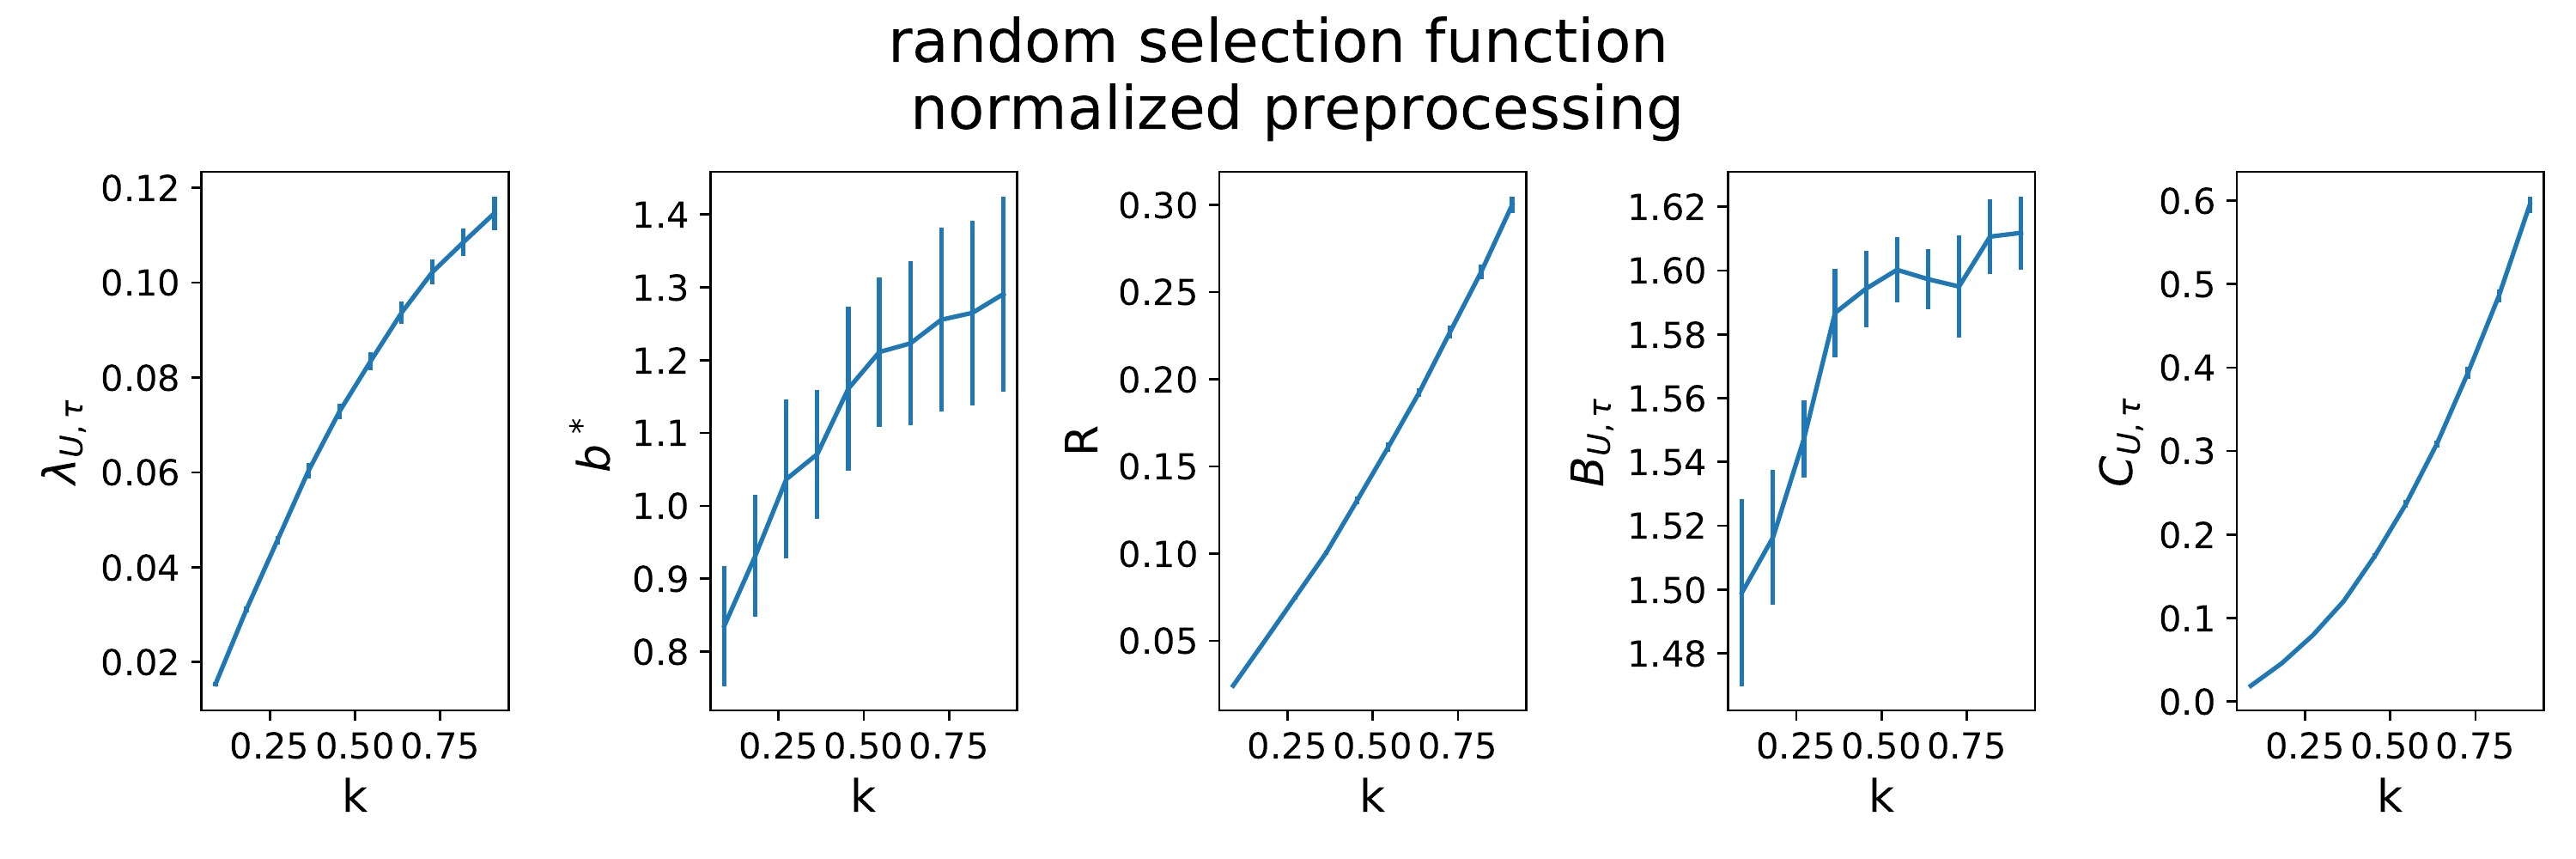}
 \caption{Parameters for ``random"}
\label{fig:param,random}
\end{figure}

\begin{figure}
\centering

   \includegraphics[width=1\linewidth]{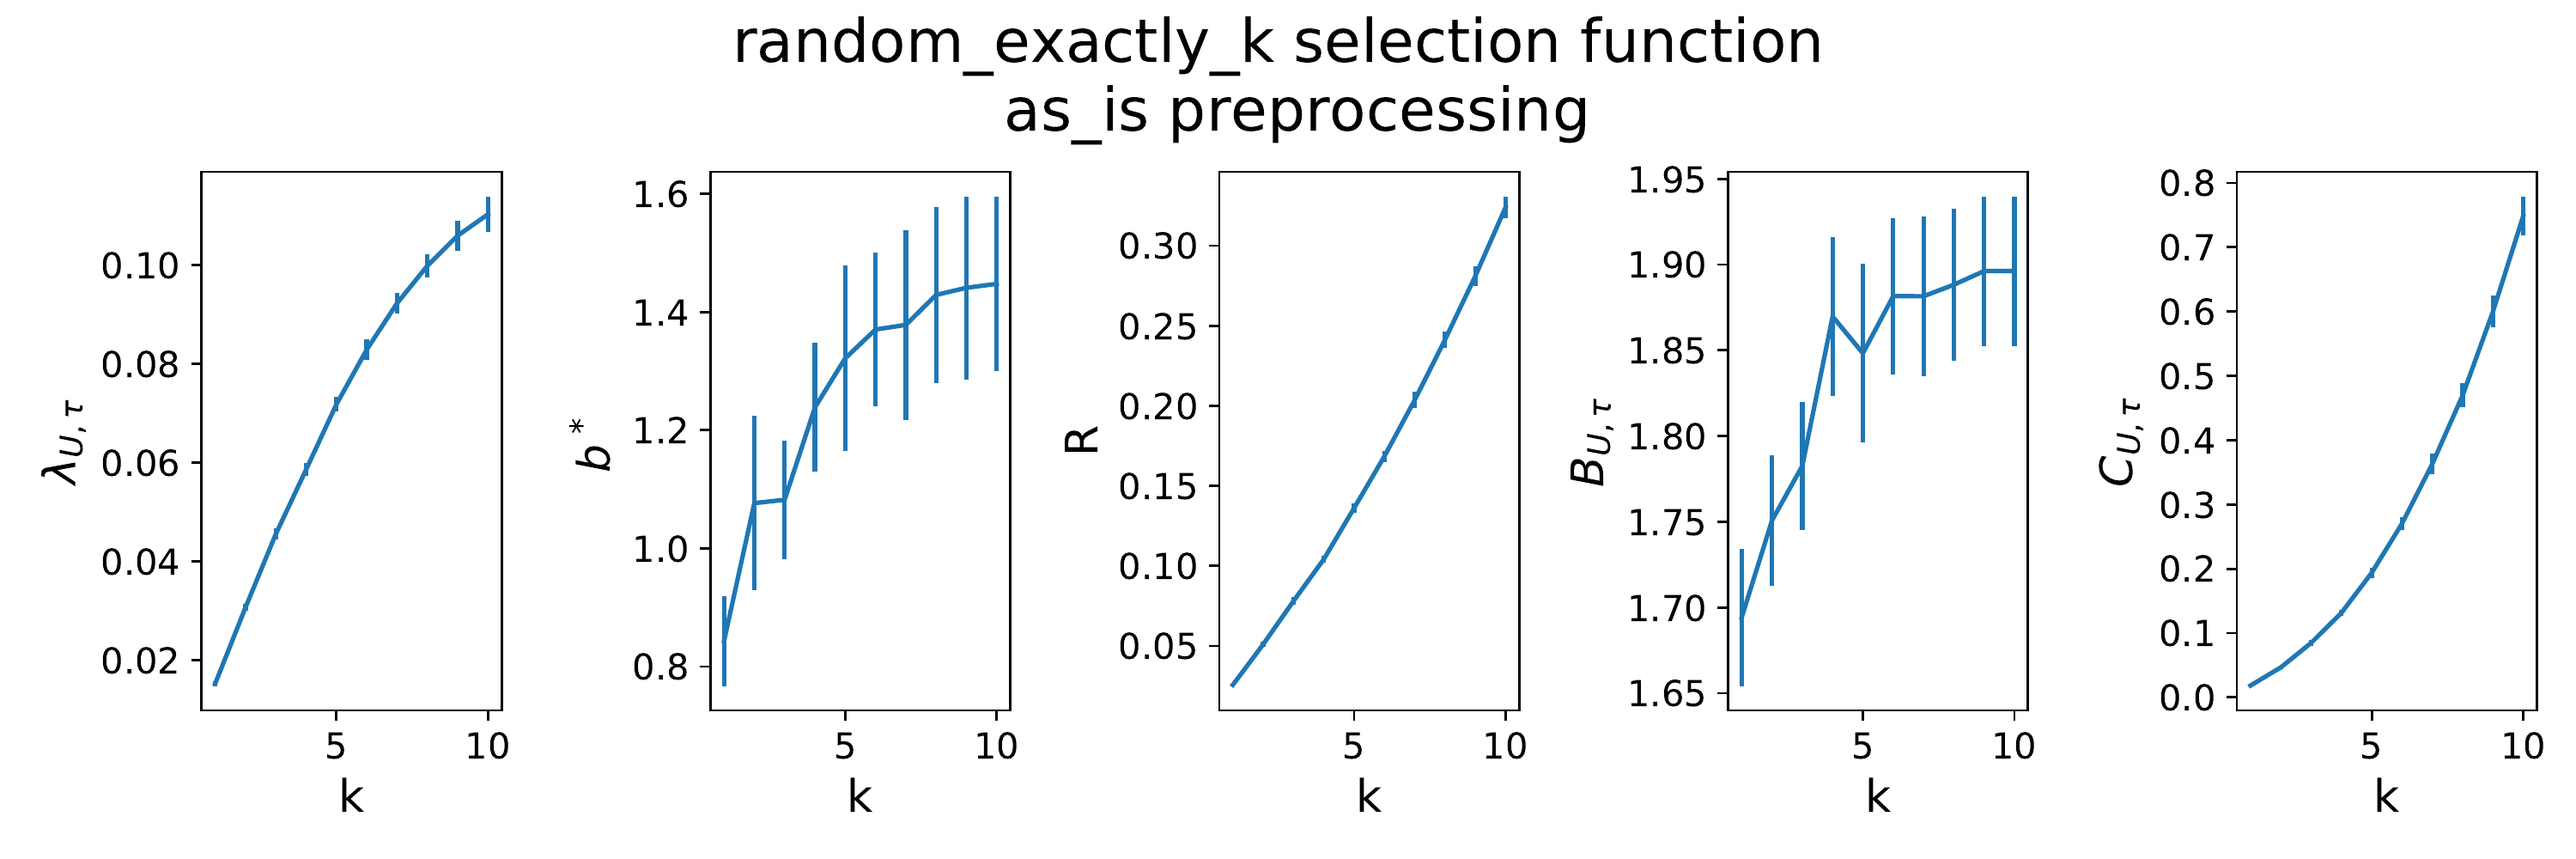}

 \includegraphics[width=1\linewidth]{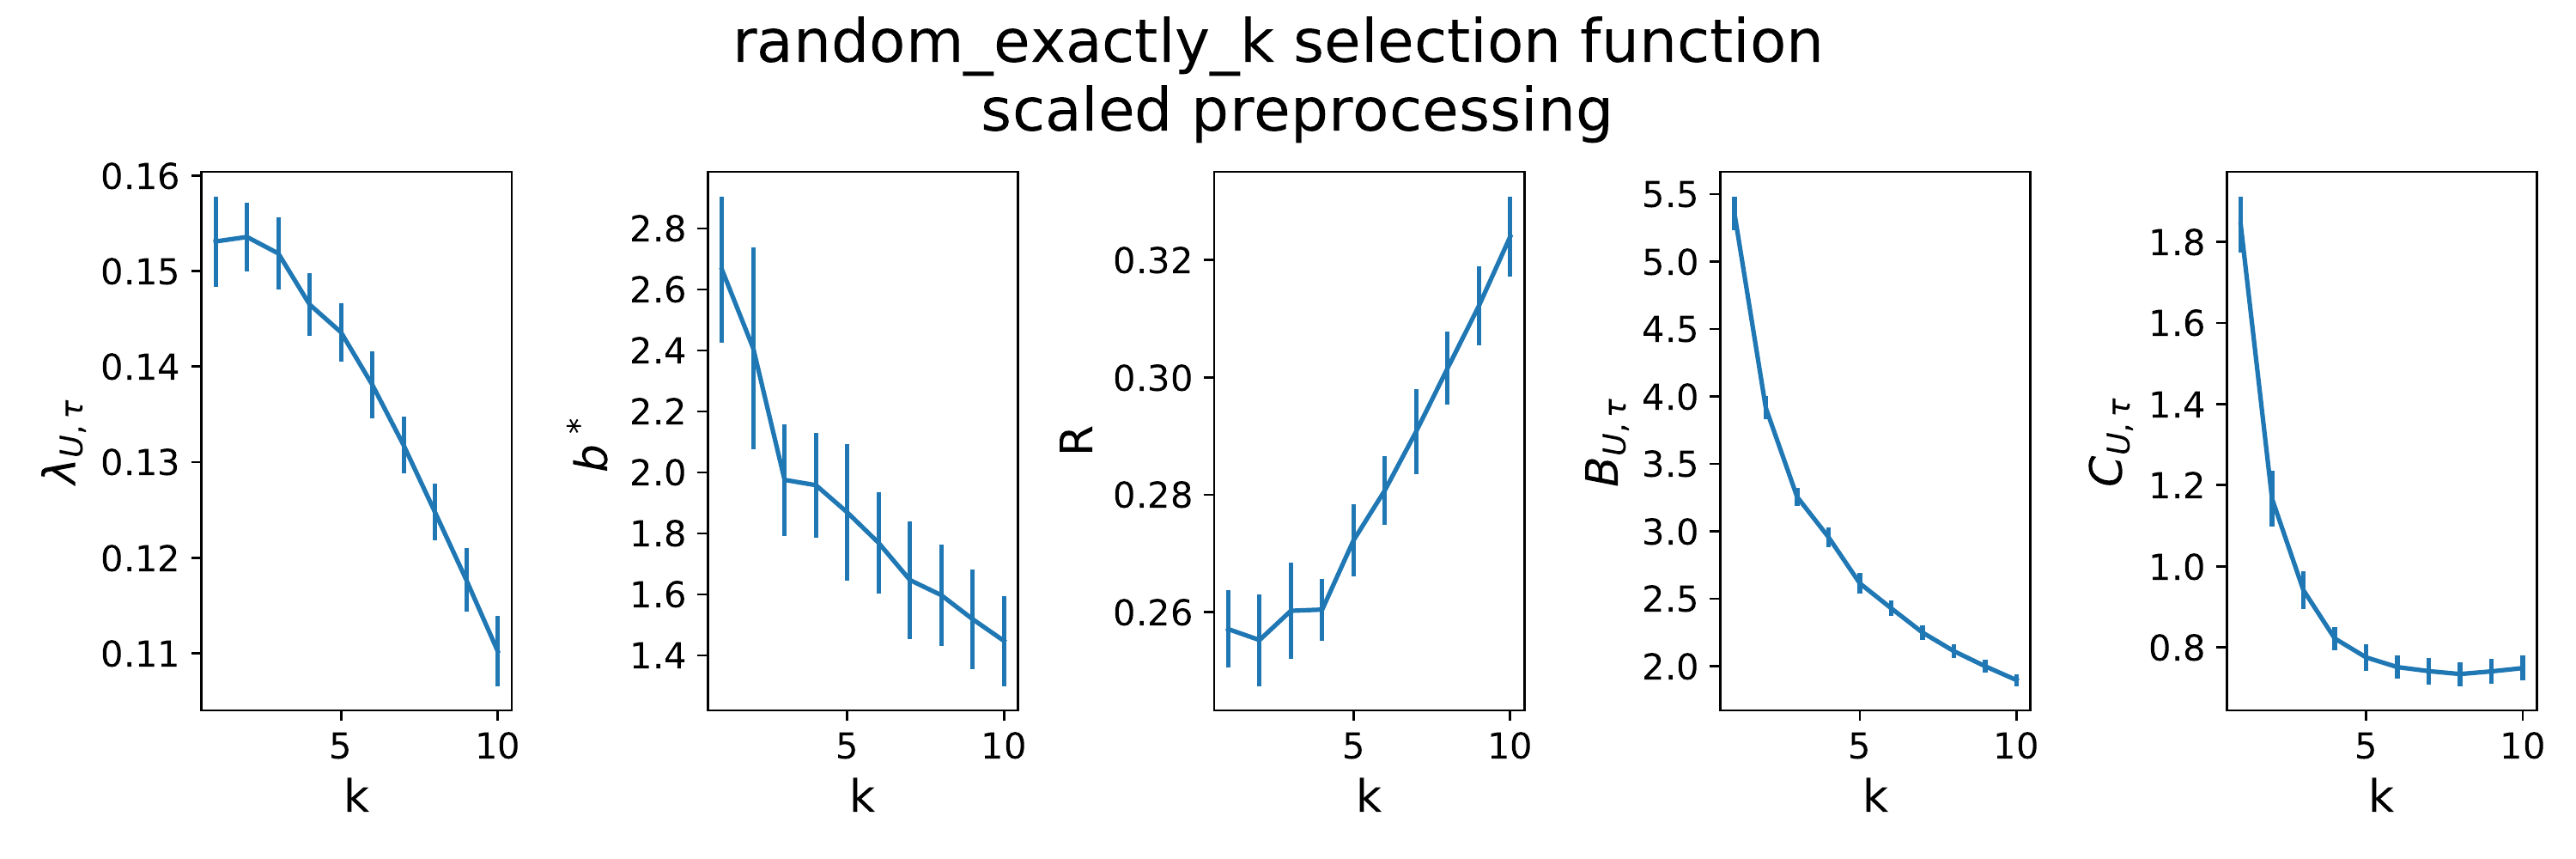}

    \includegraphics[width=1\linewidth]{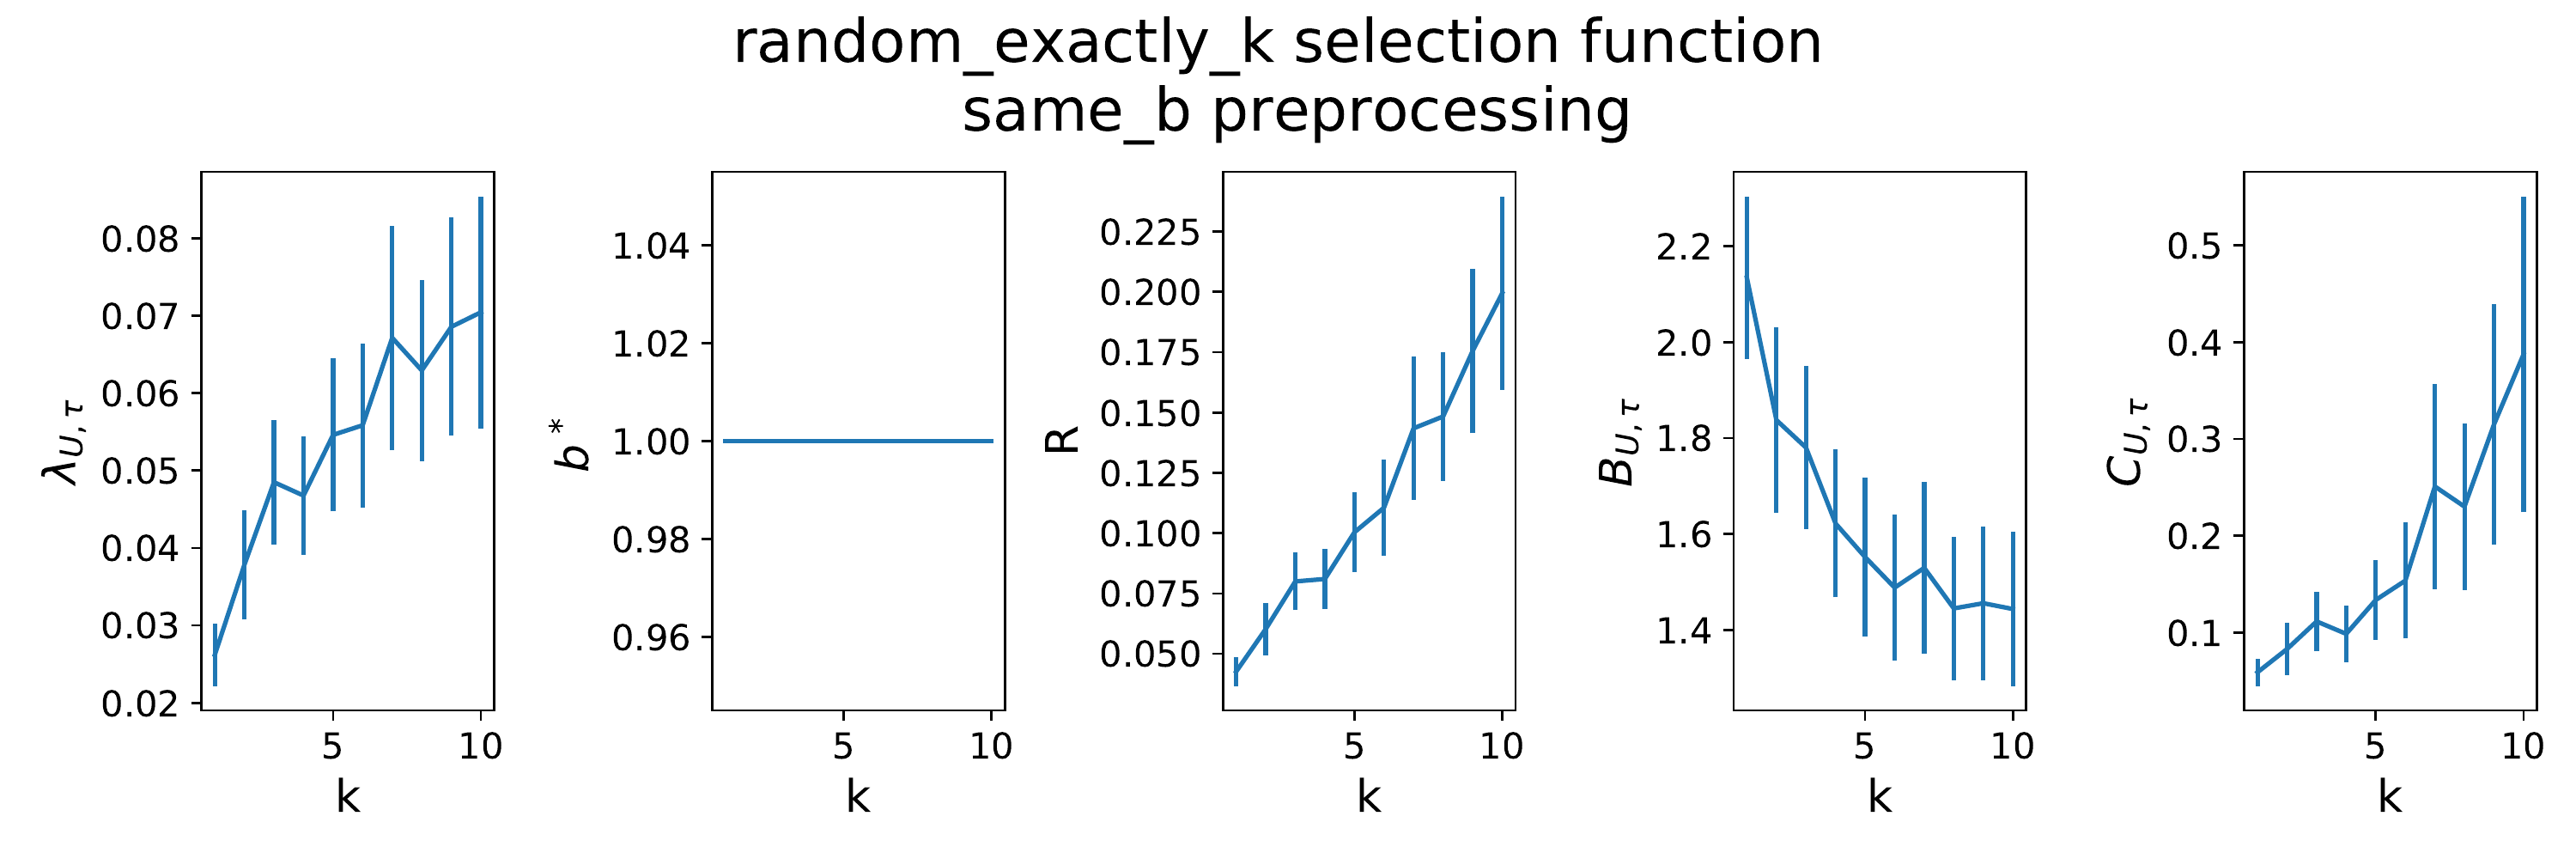}
   
 \includegraphics[width=1\linewidth]{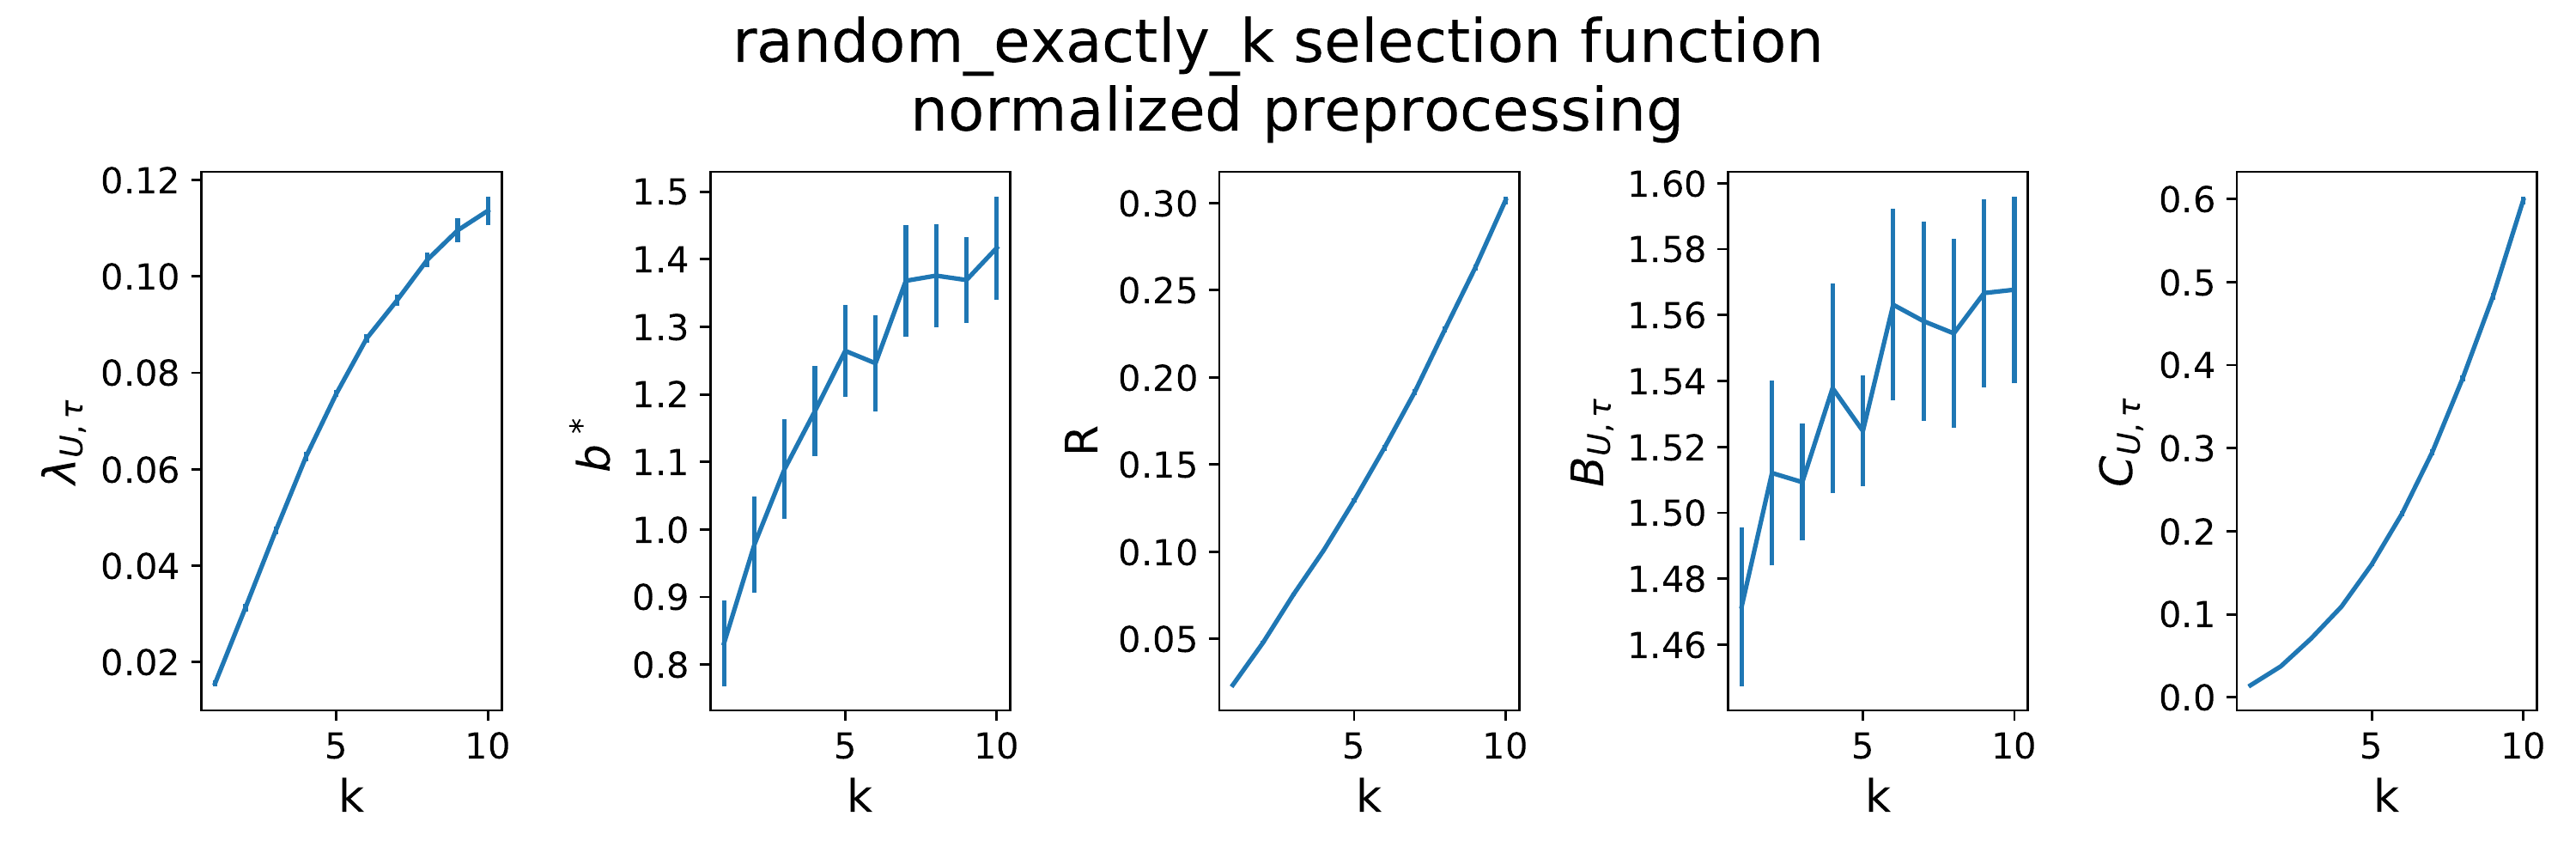}
  \caption{Parameters for ``random exactly $k$"}
\label{fig:param,random_exactly_k}
\end{figure}

\begin{figure}
\centering

   \includegraphics[width=1\linewidth]{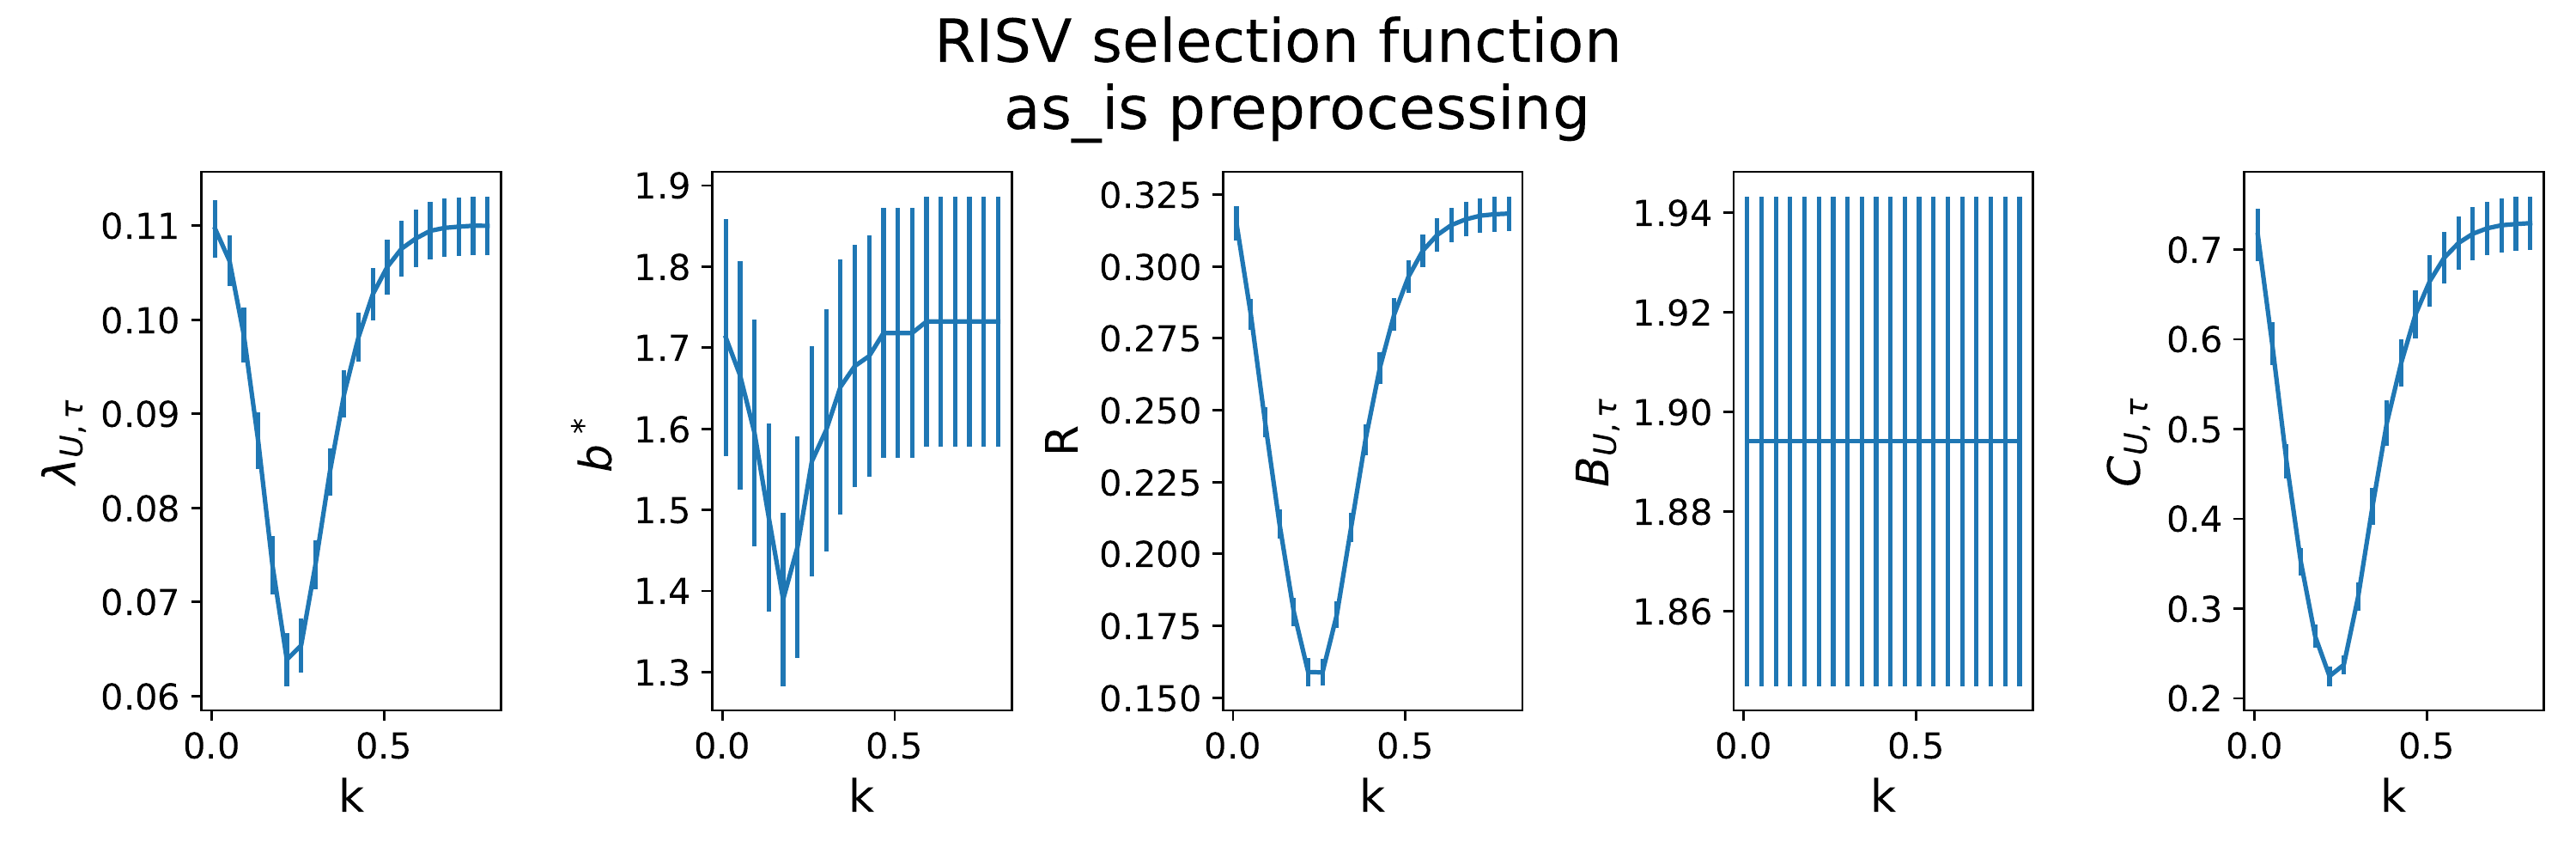}

    \includegraphics[width=1\linewidth]{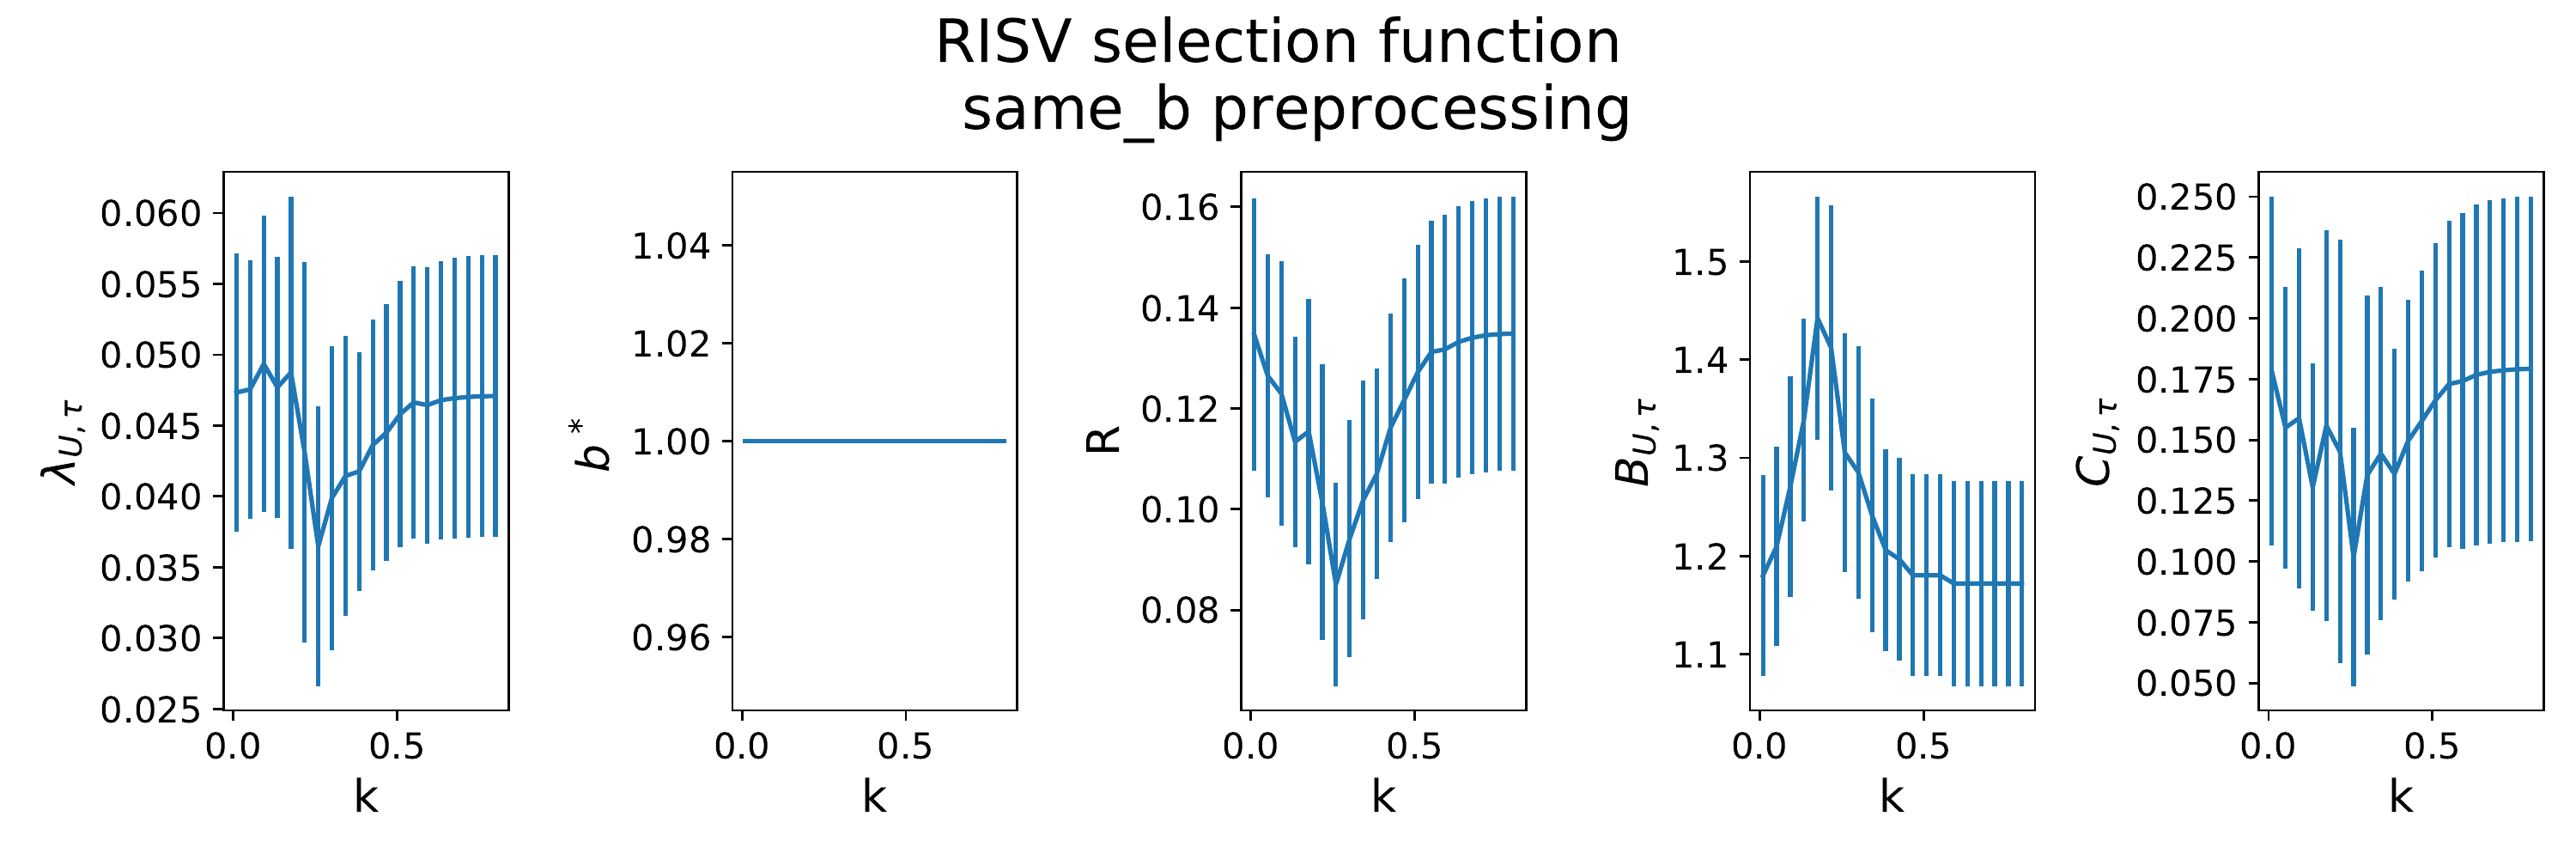}
   
 \includegraphics[width=1\linewidth]{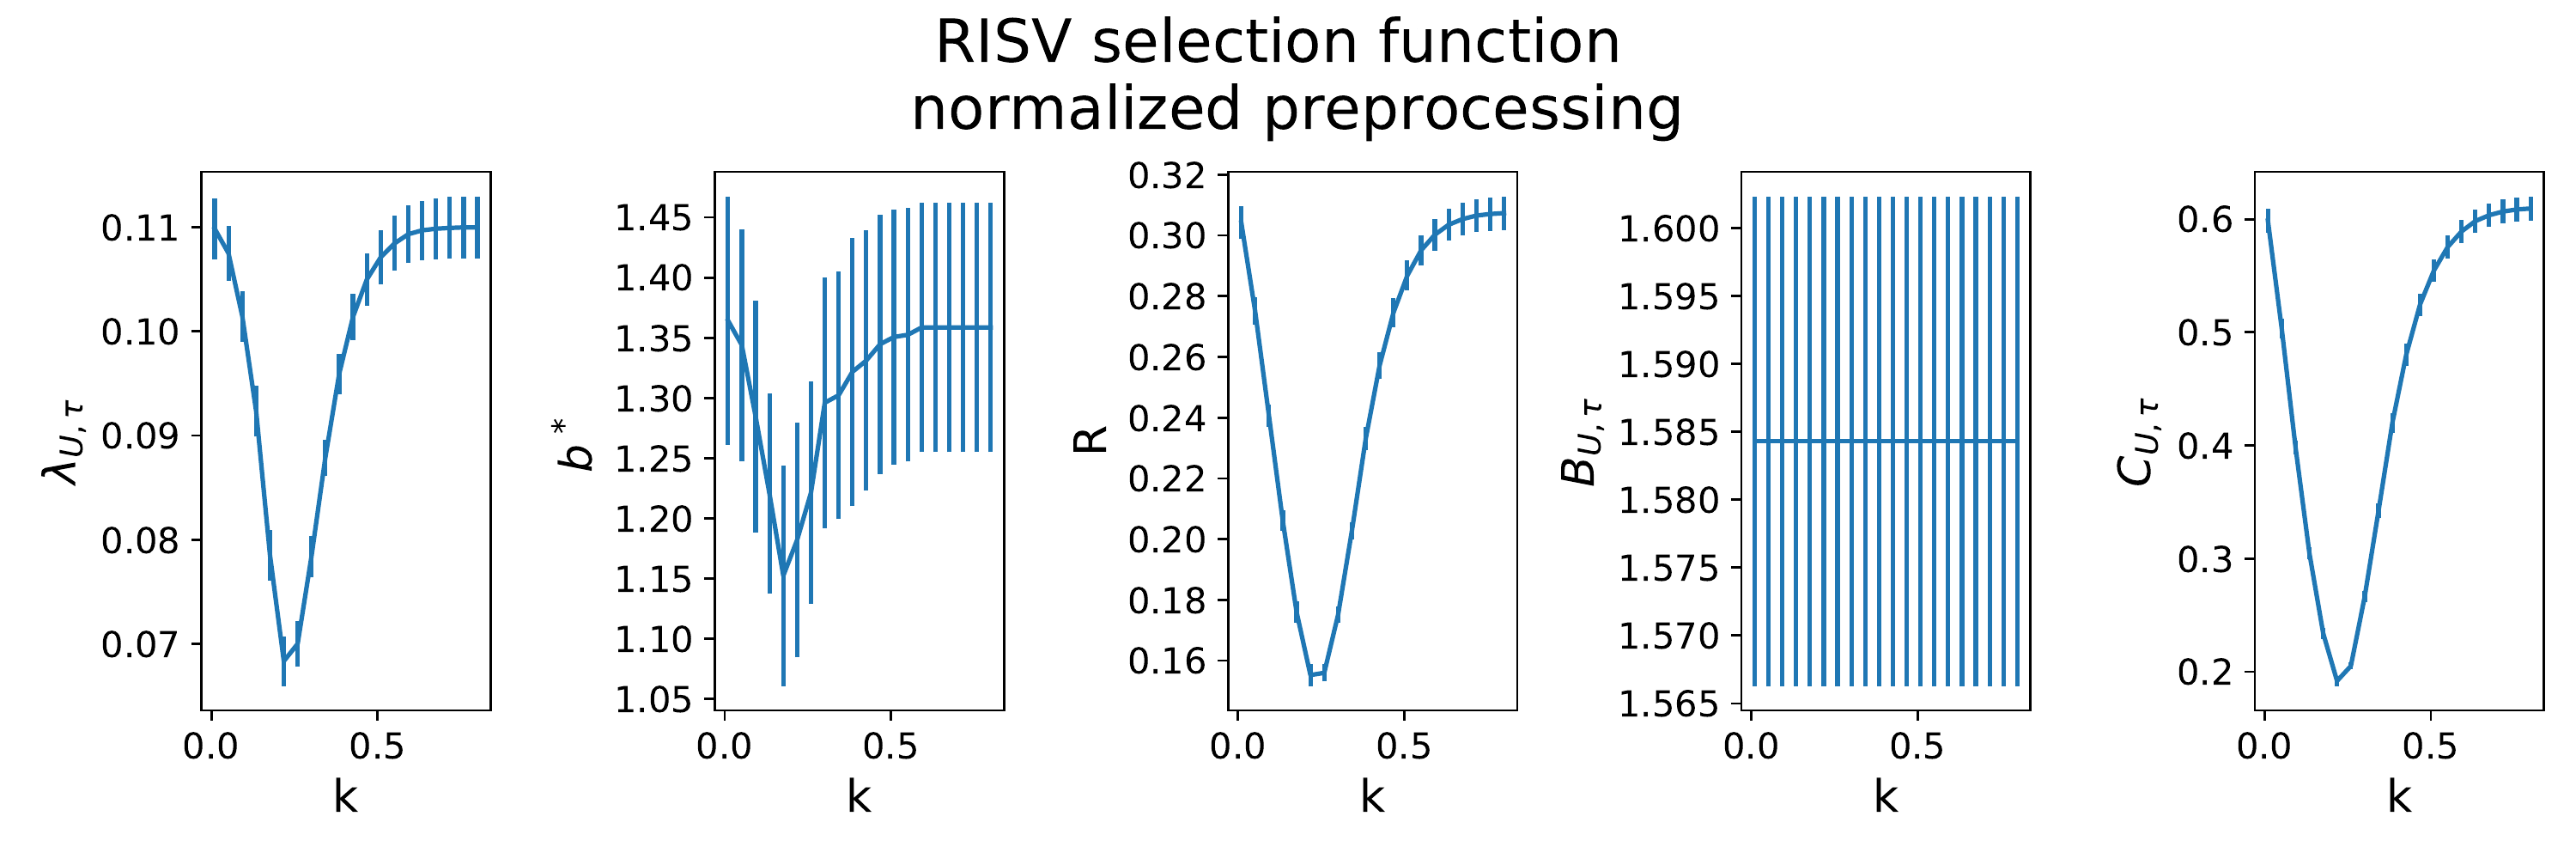}
   \caption{Parameters for RISV}
\label{fig:param,risv}
\end{figure}

\begin{figure}
\centering

   \includegraphics[width=1\linewidth]{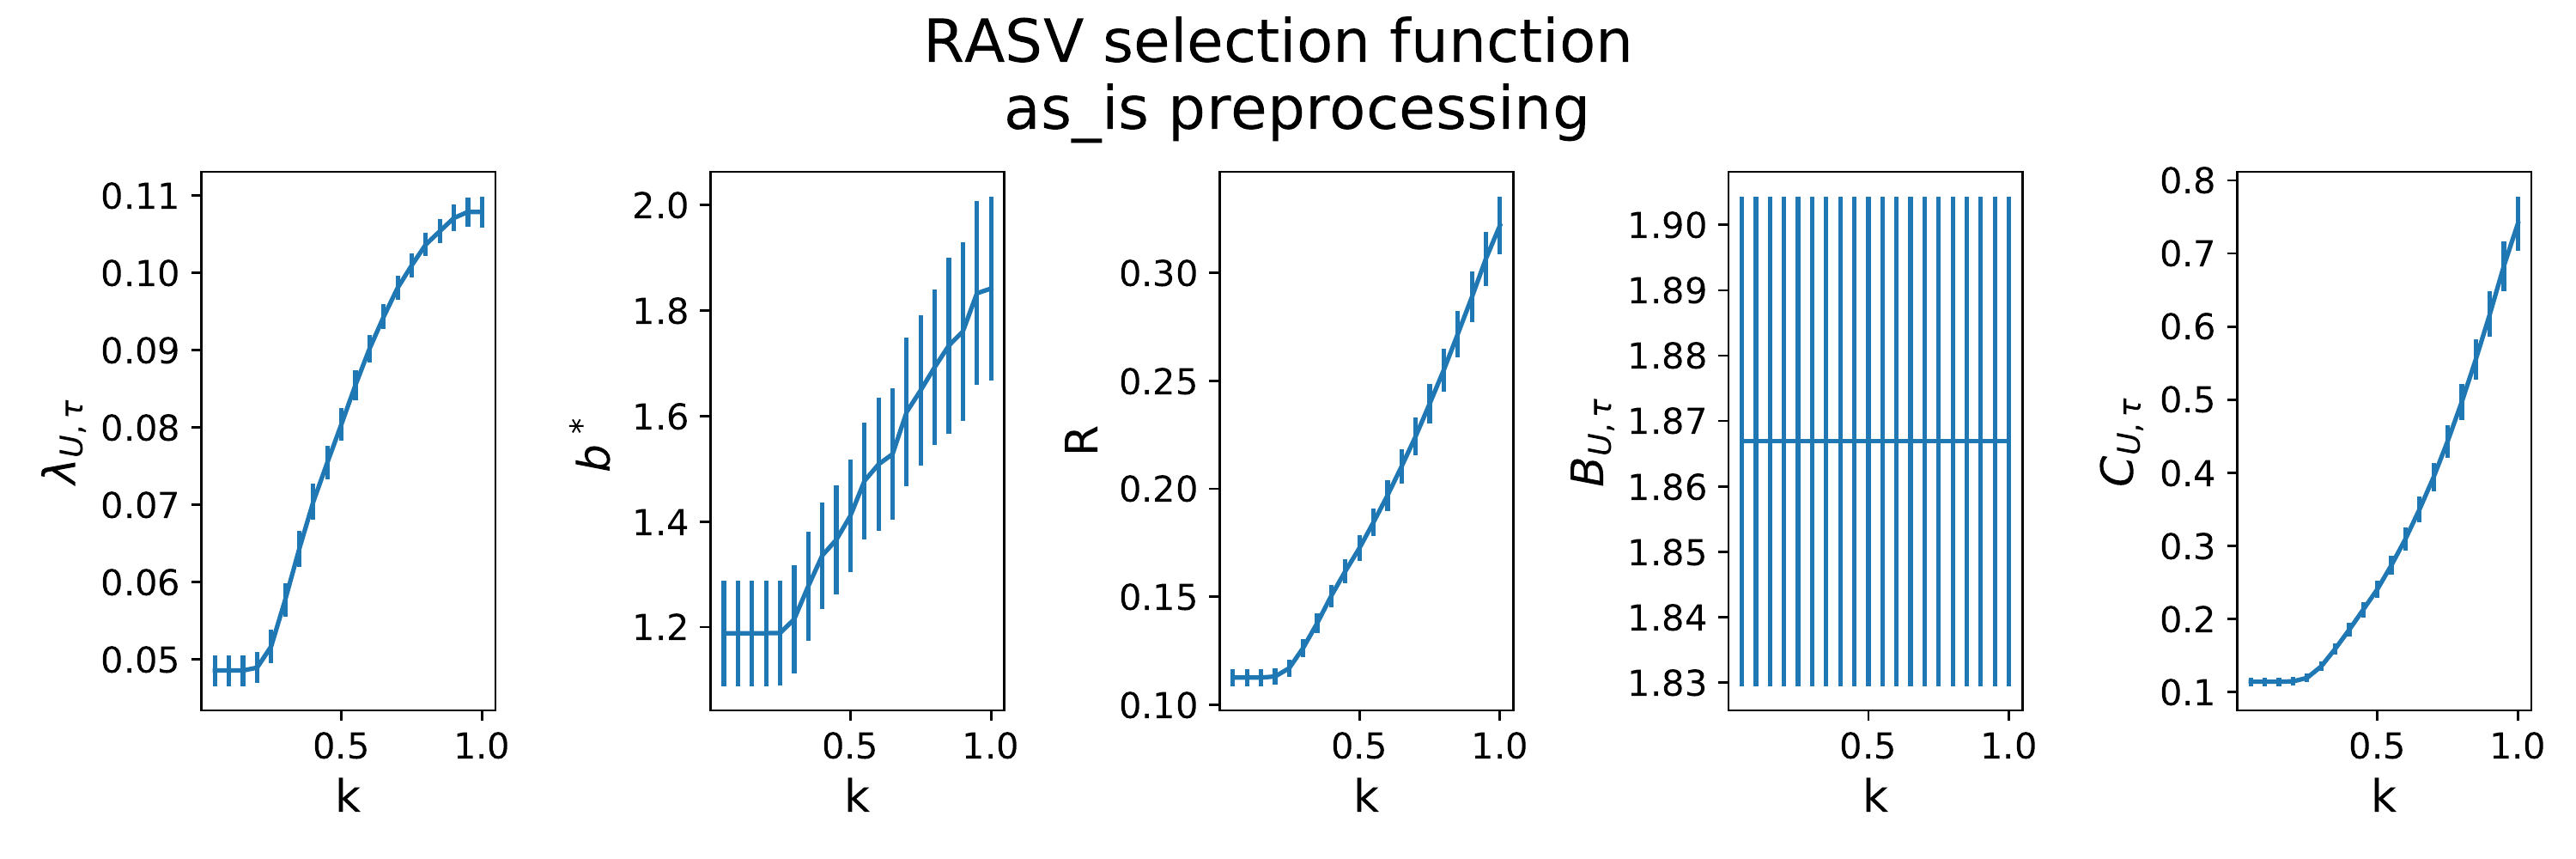}

    \includegraphics[width=1\linewidth]{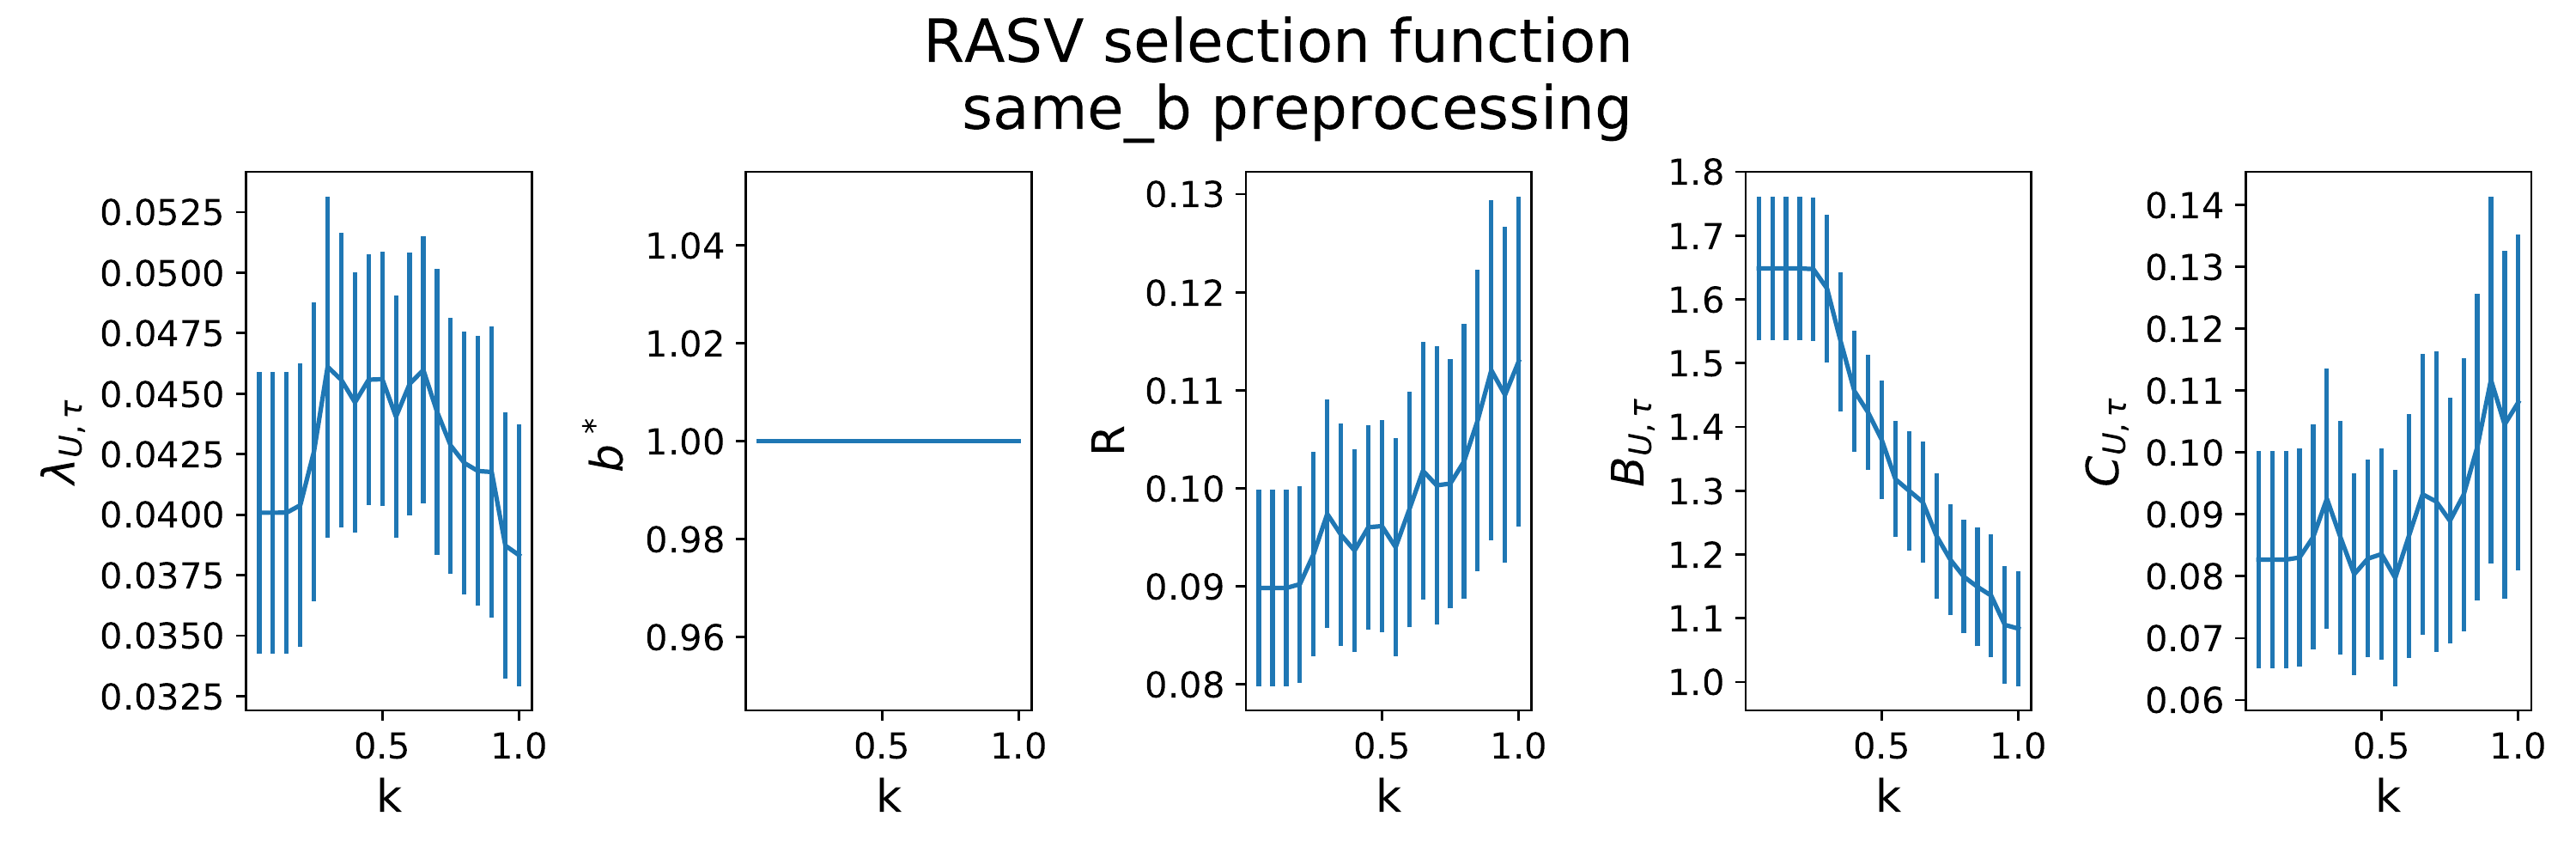}
   
 \includegraphics[width=1\linewidth]{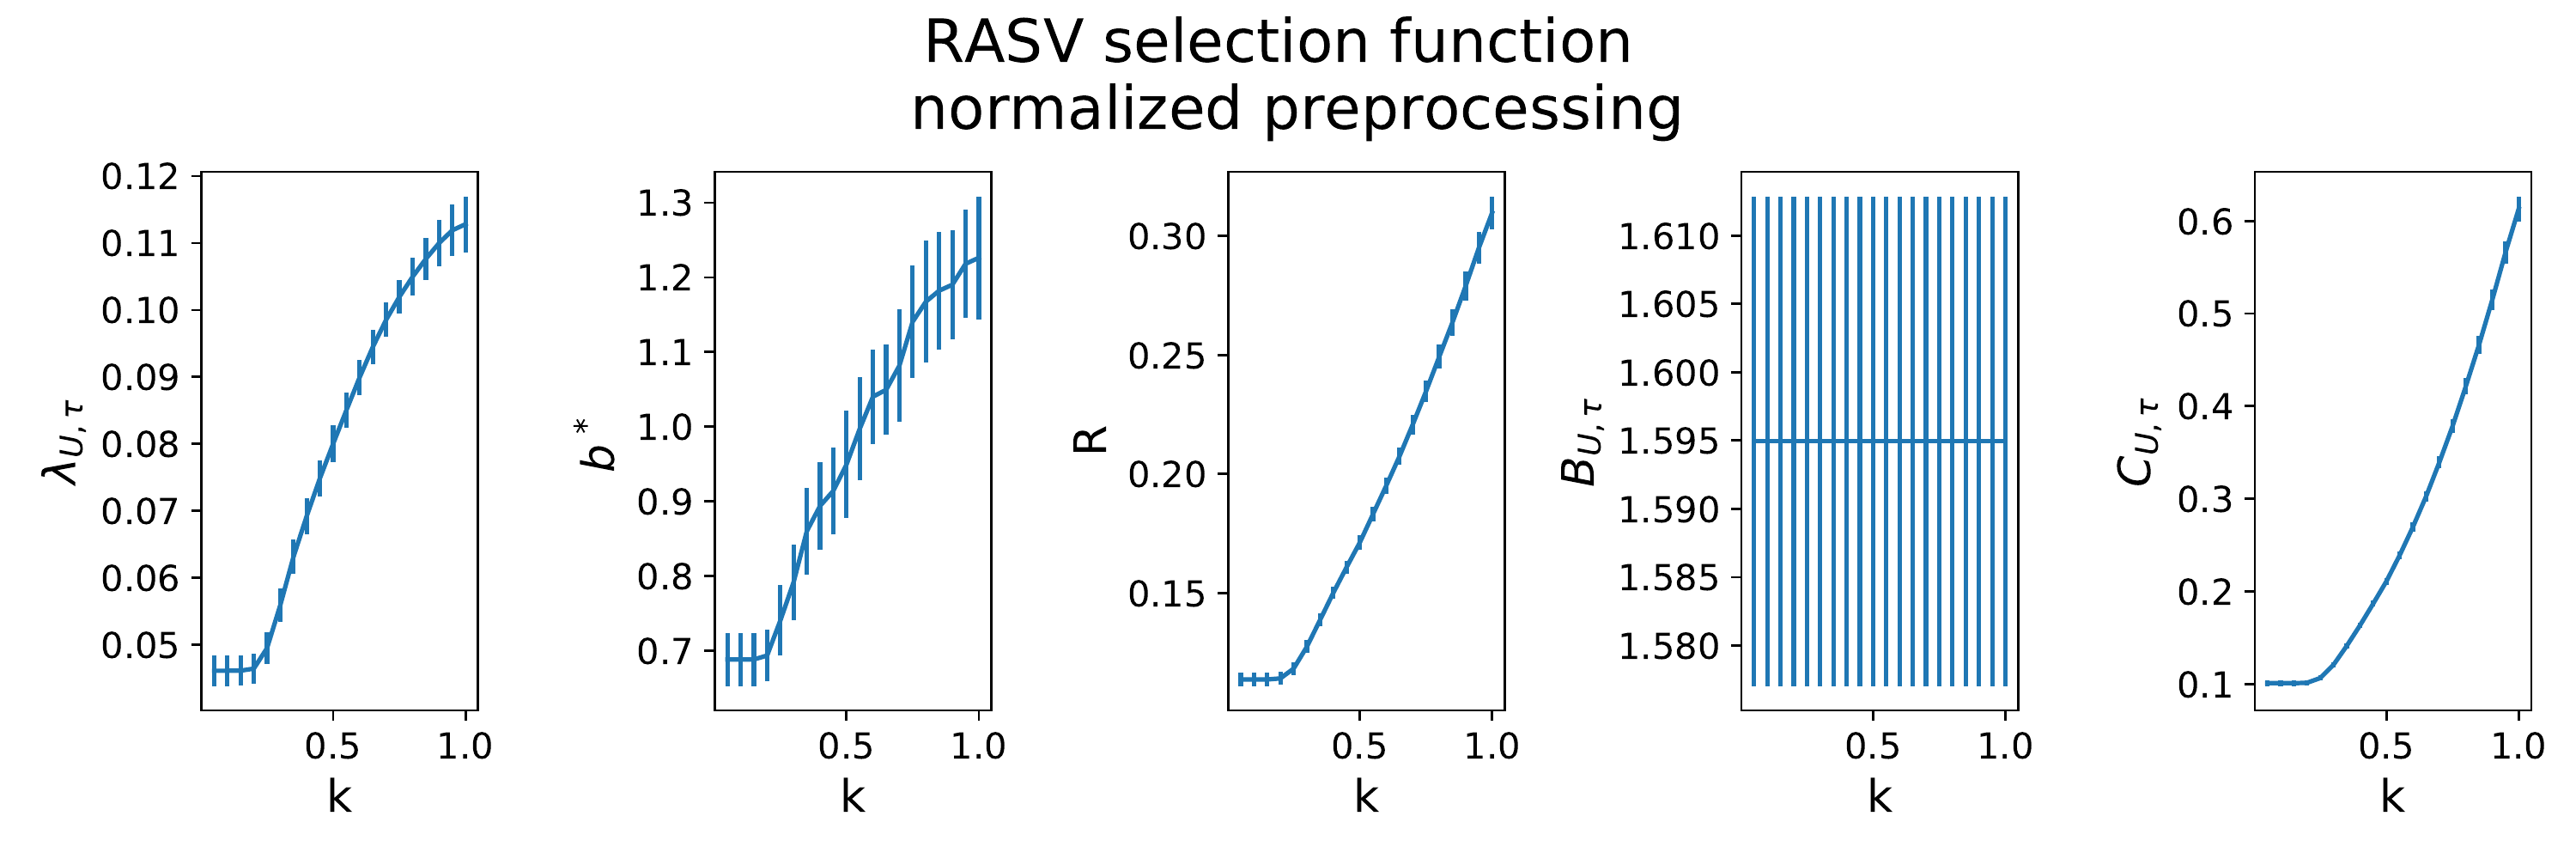}
    \caption{Parameters for RASV}
\label{fig:param,rasv}
\end{figure}

\subsection{Number of samples and bound}
\begin{figure}
\centering

   \includegraphics[width=1\linewidth]{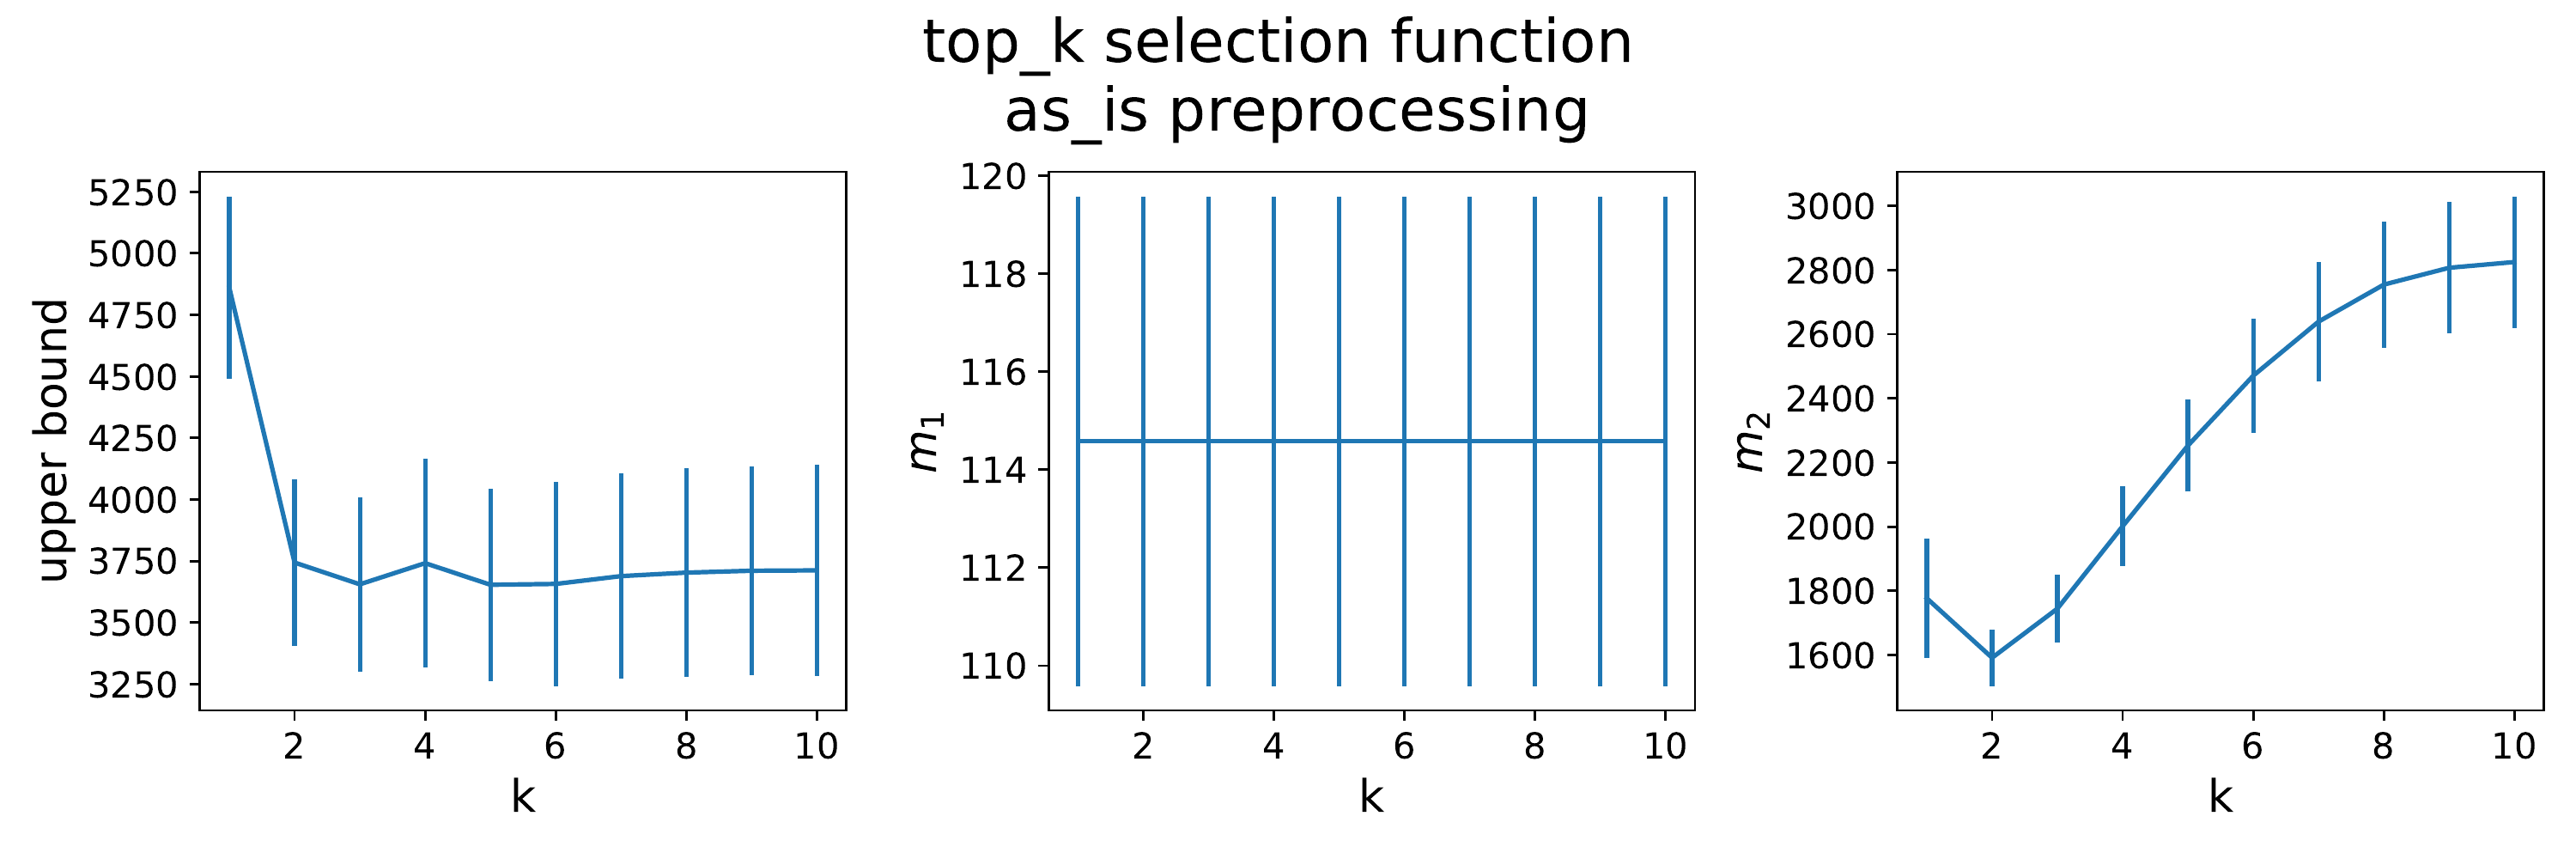}

 \includegraphics[width=1\linewidth]{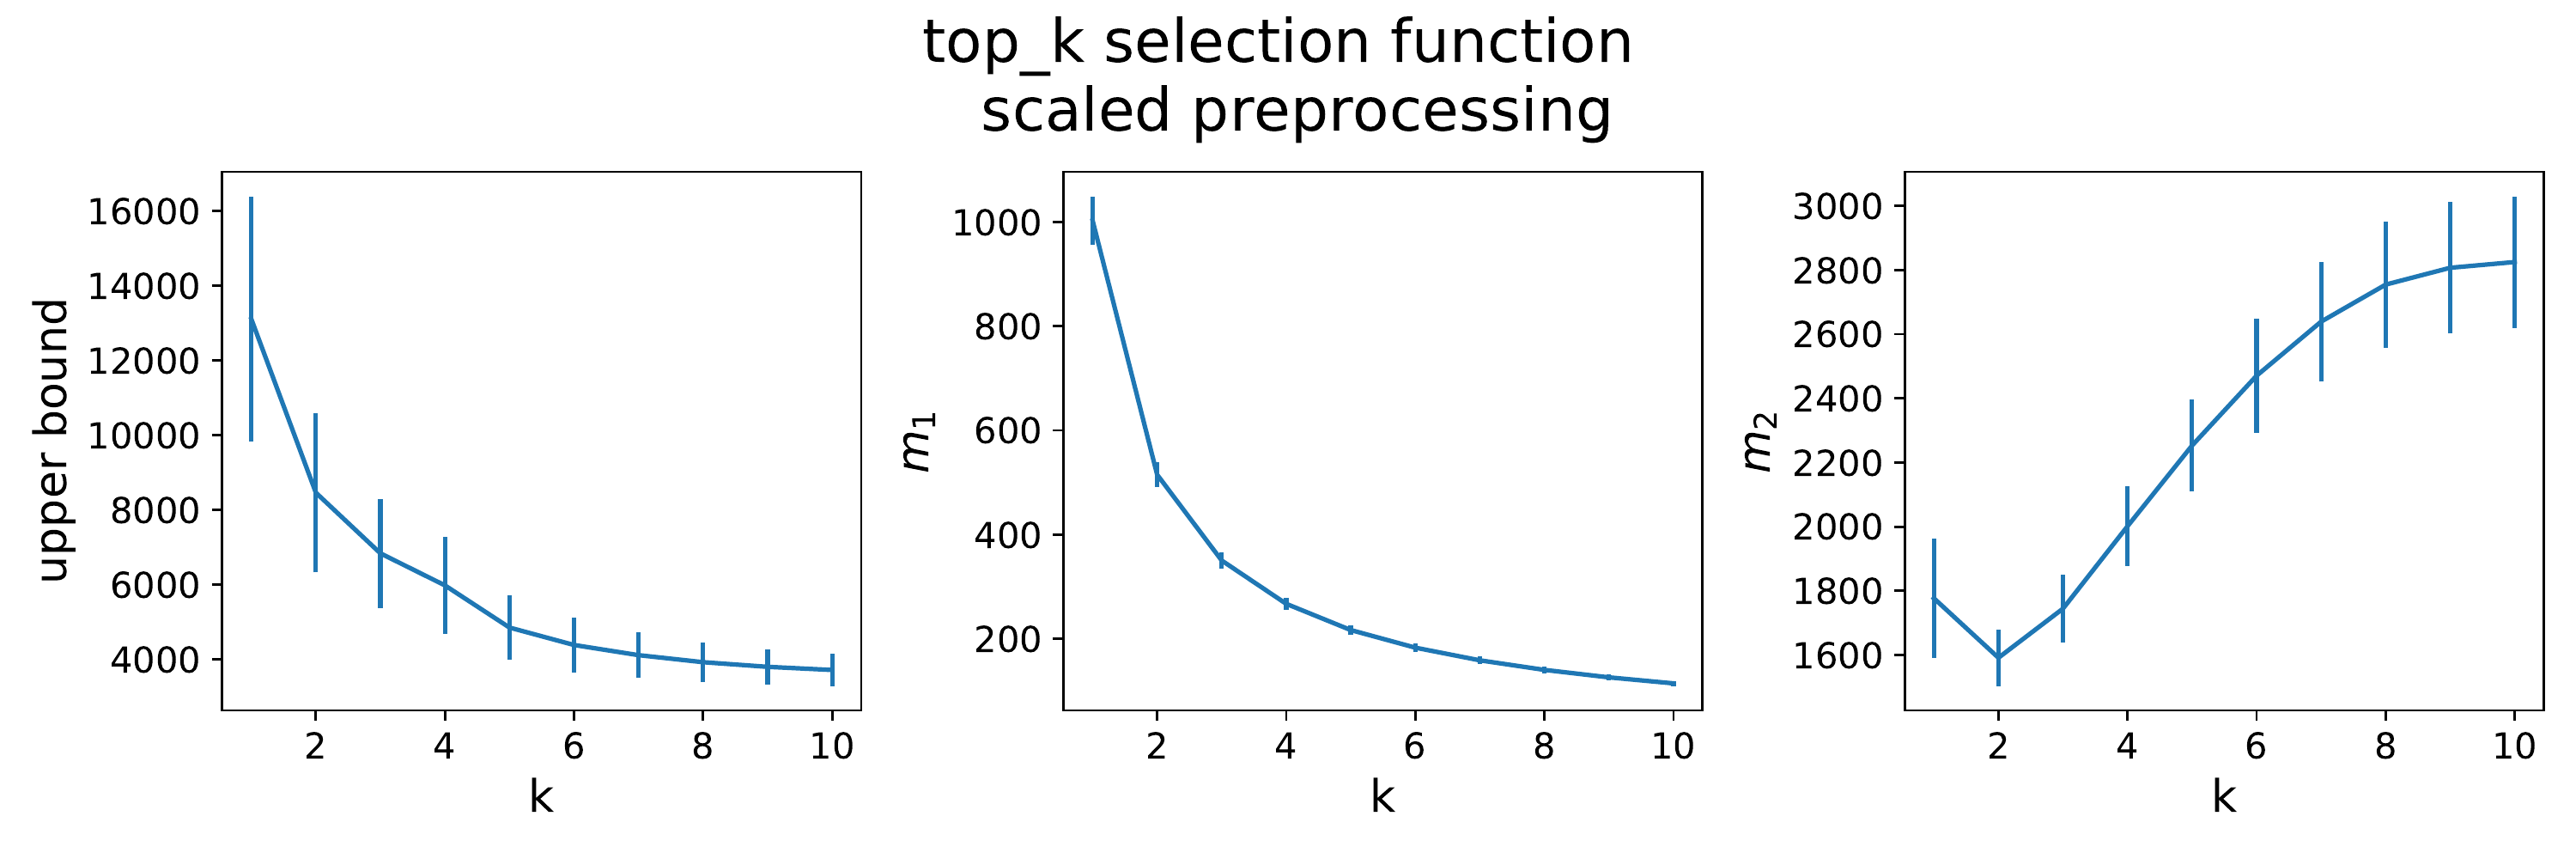}

    \includegraphics[width=1\linewidth]{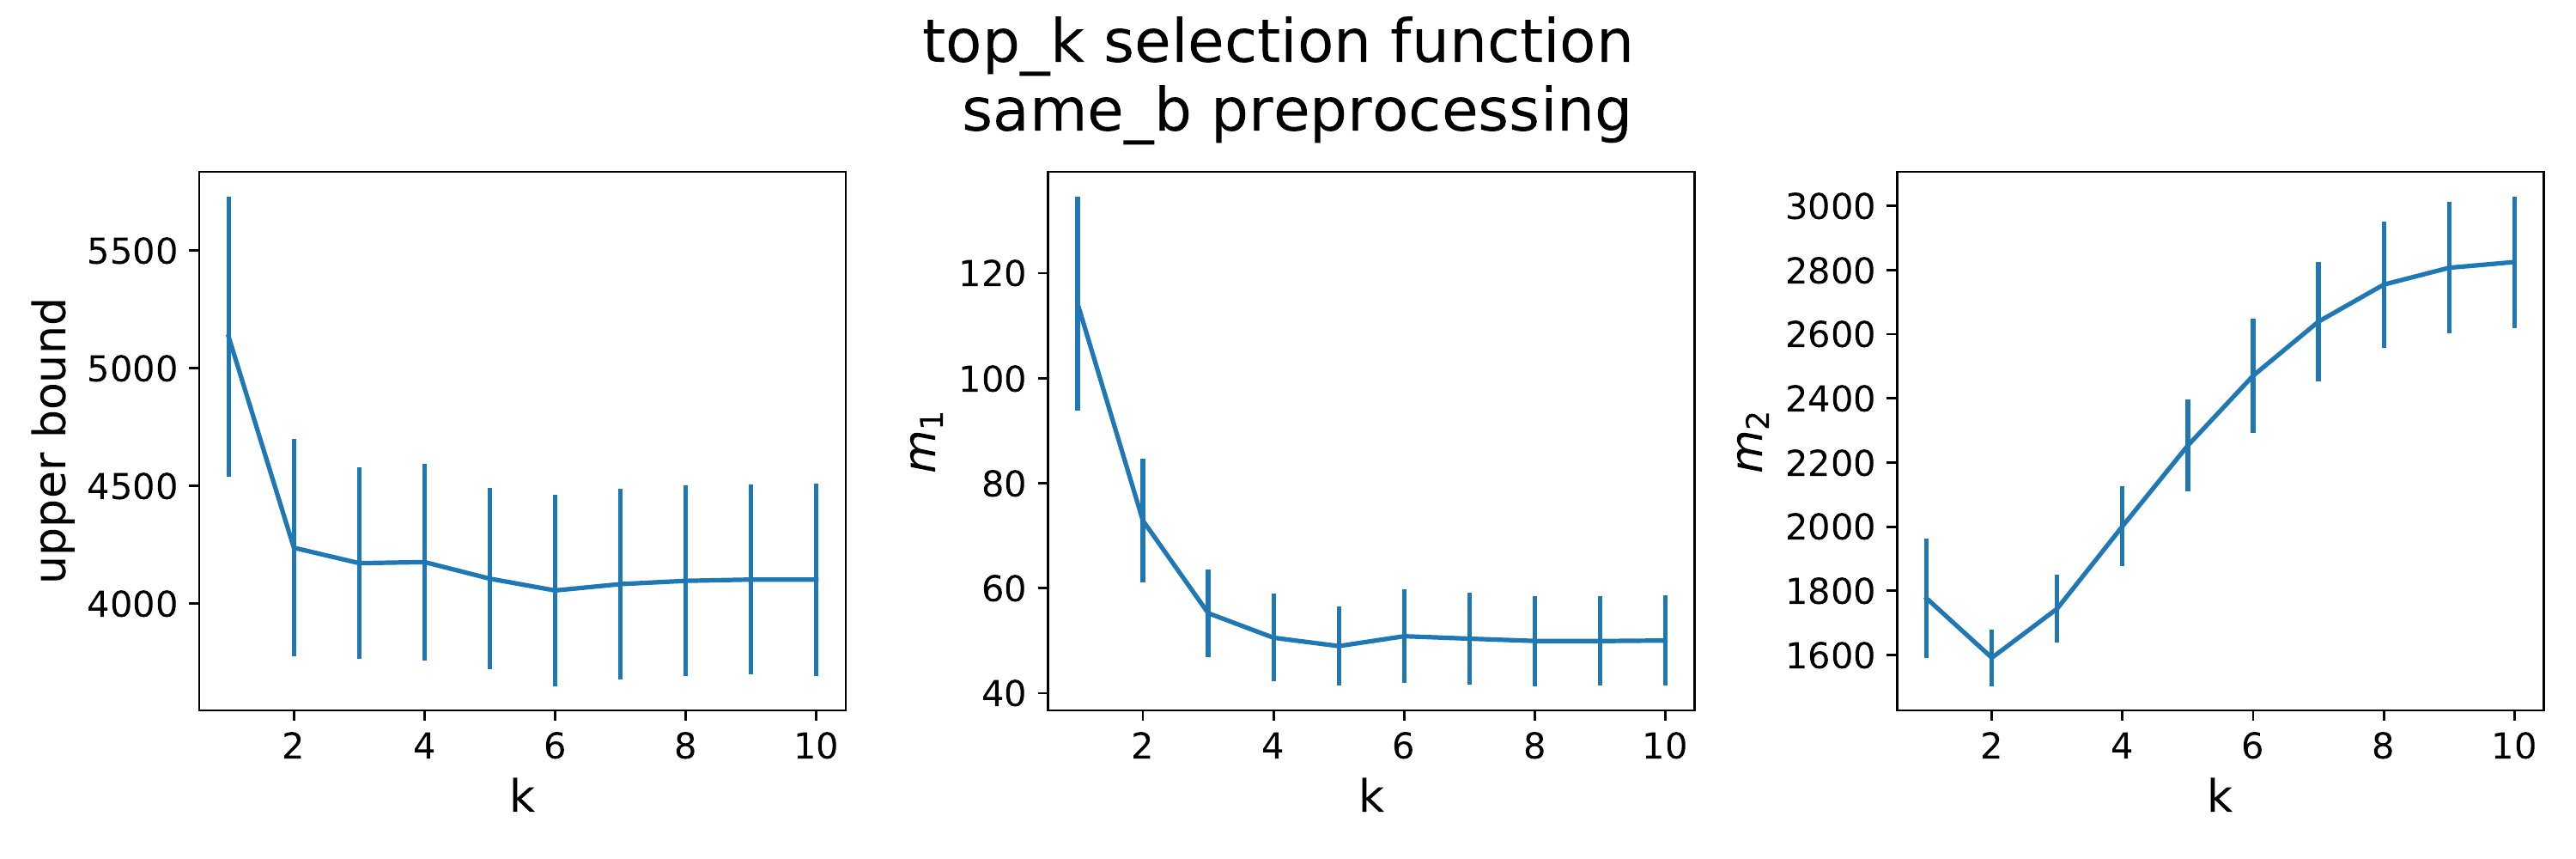}
   
 \includegraphics[width=1\linewidth]{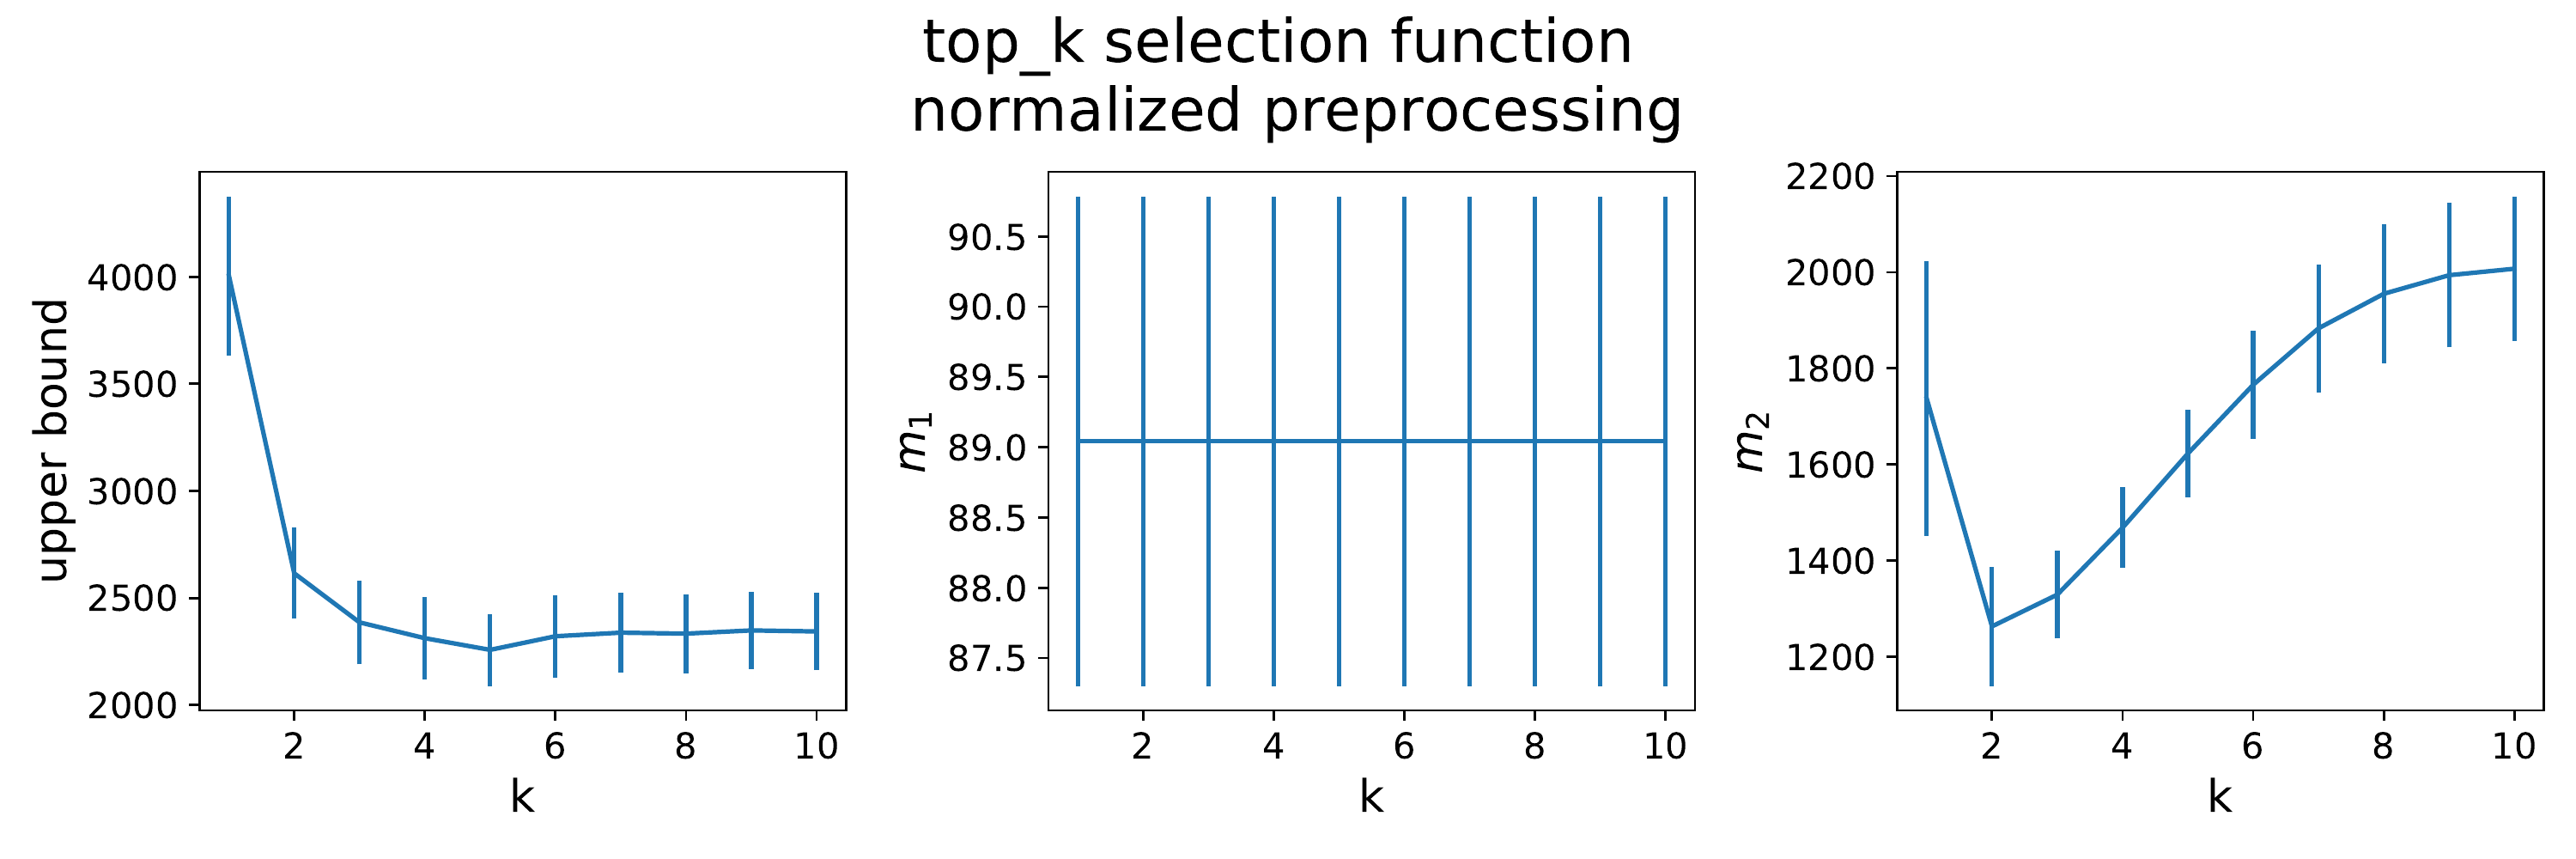}

\caption{Number of samples and bound for ``top $k$"}
\label{fig:samp,topk}
\end{figure}

\begin{figure}
\centering

   \includegraphics[width=1\linewidth]{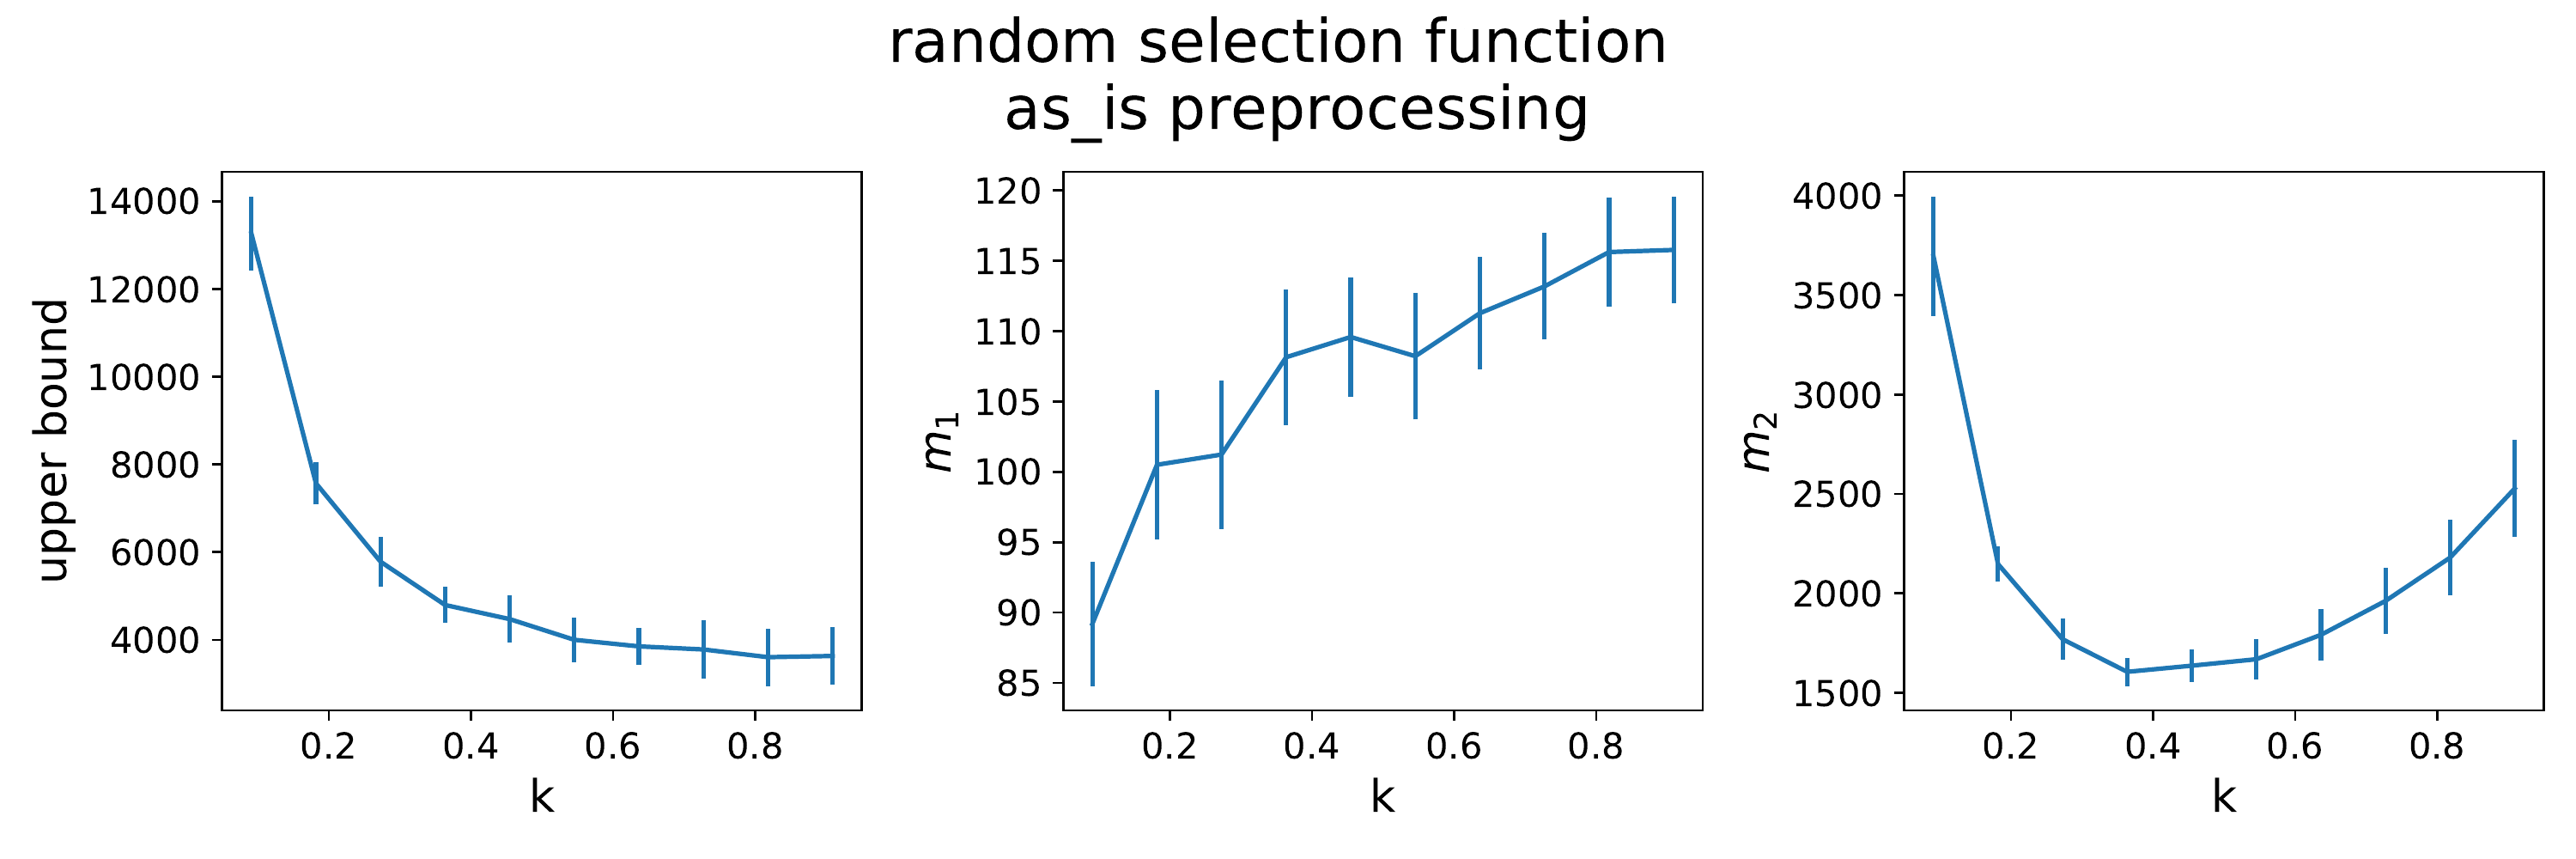}

 \includegraphics[width=1\linewidth]{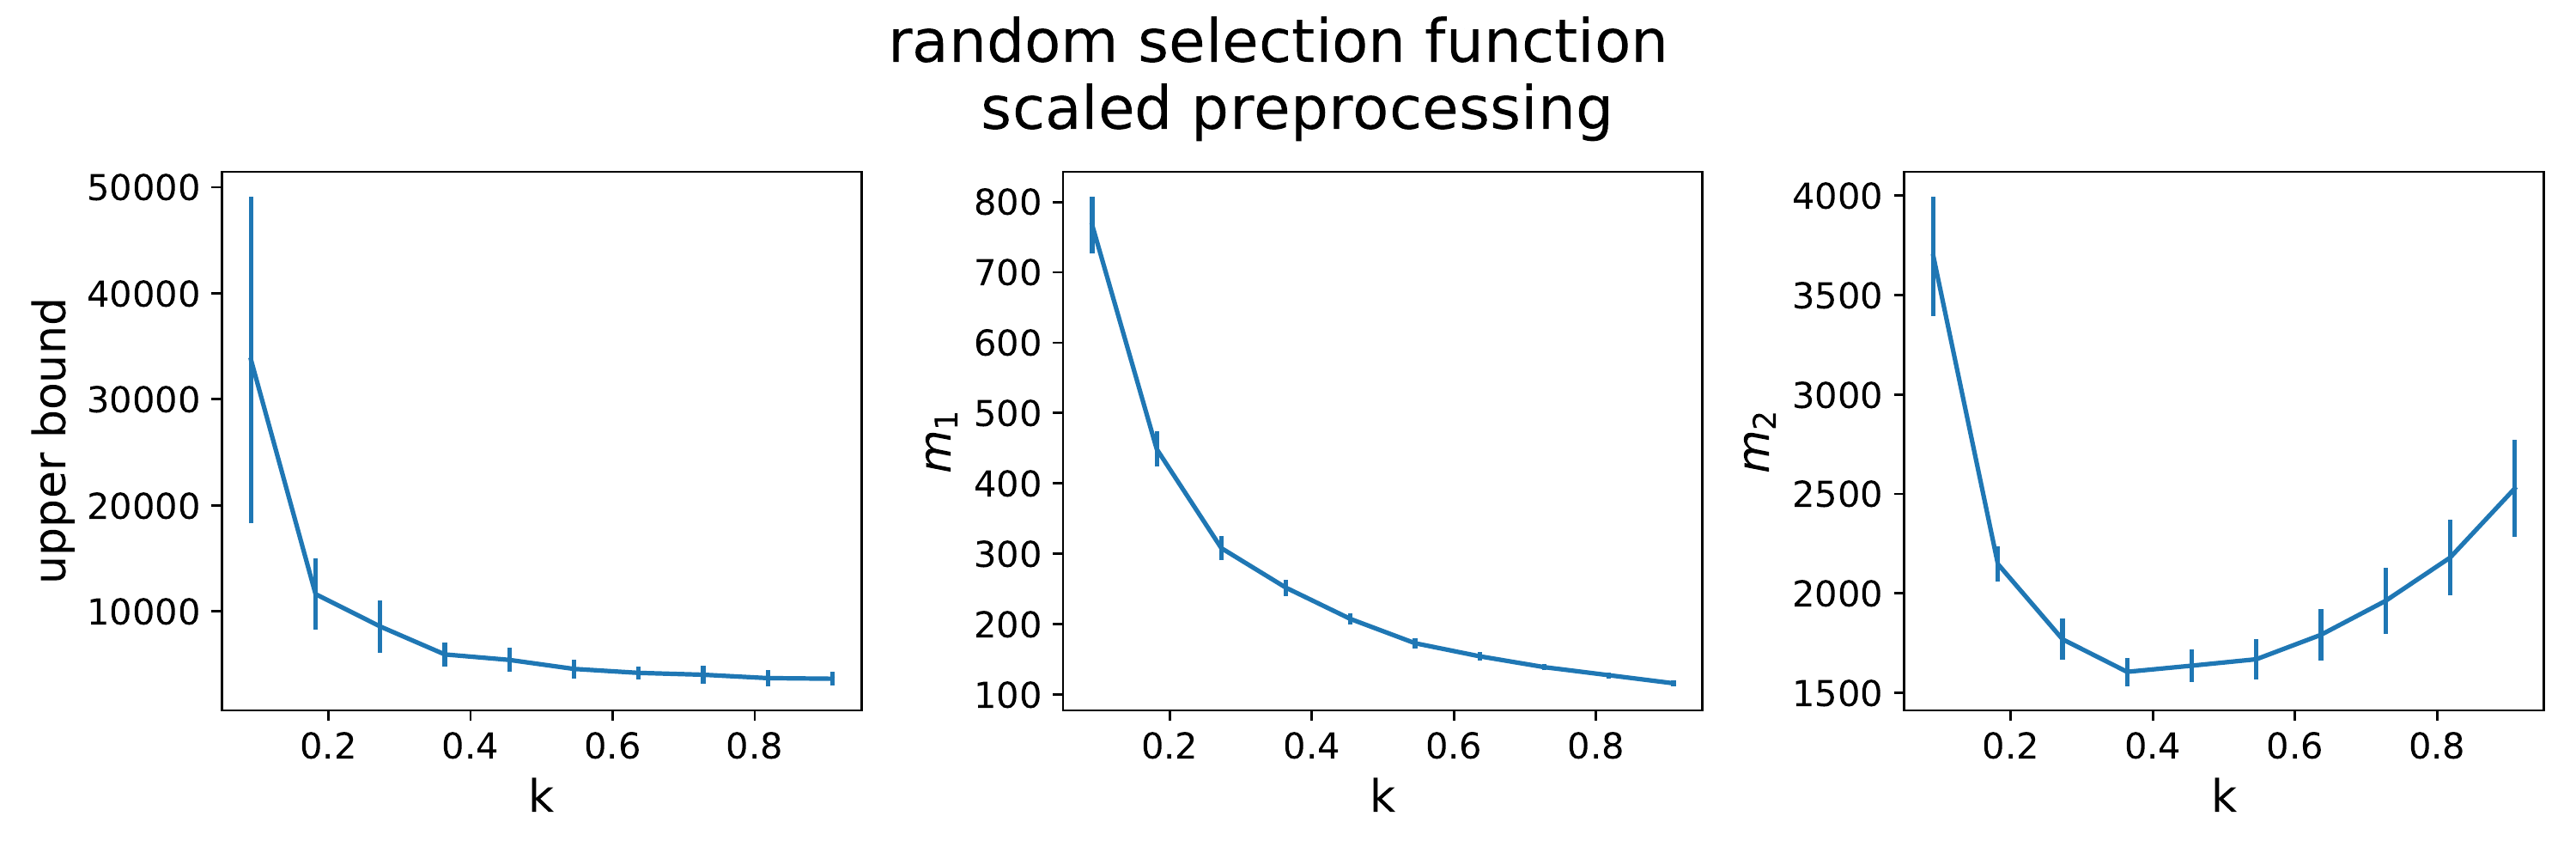}

    \includegraphics[width=1\linewidth]{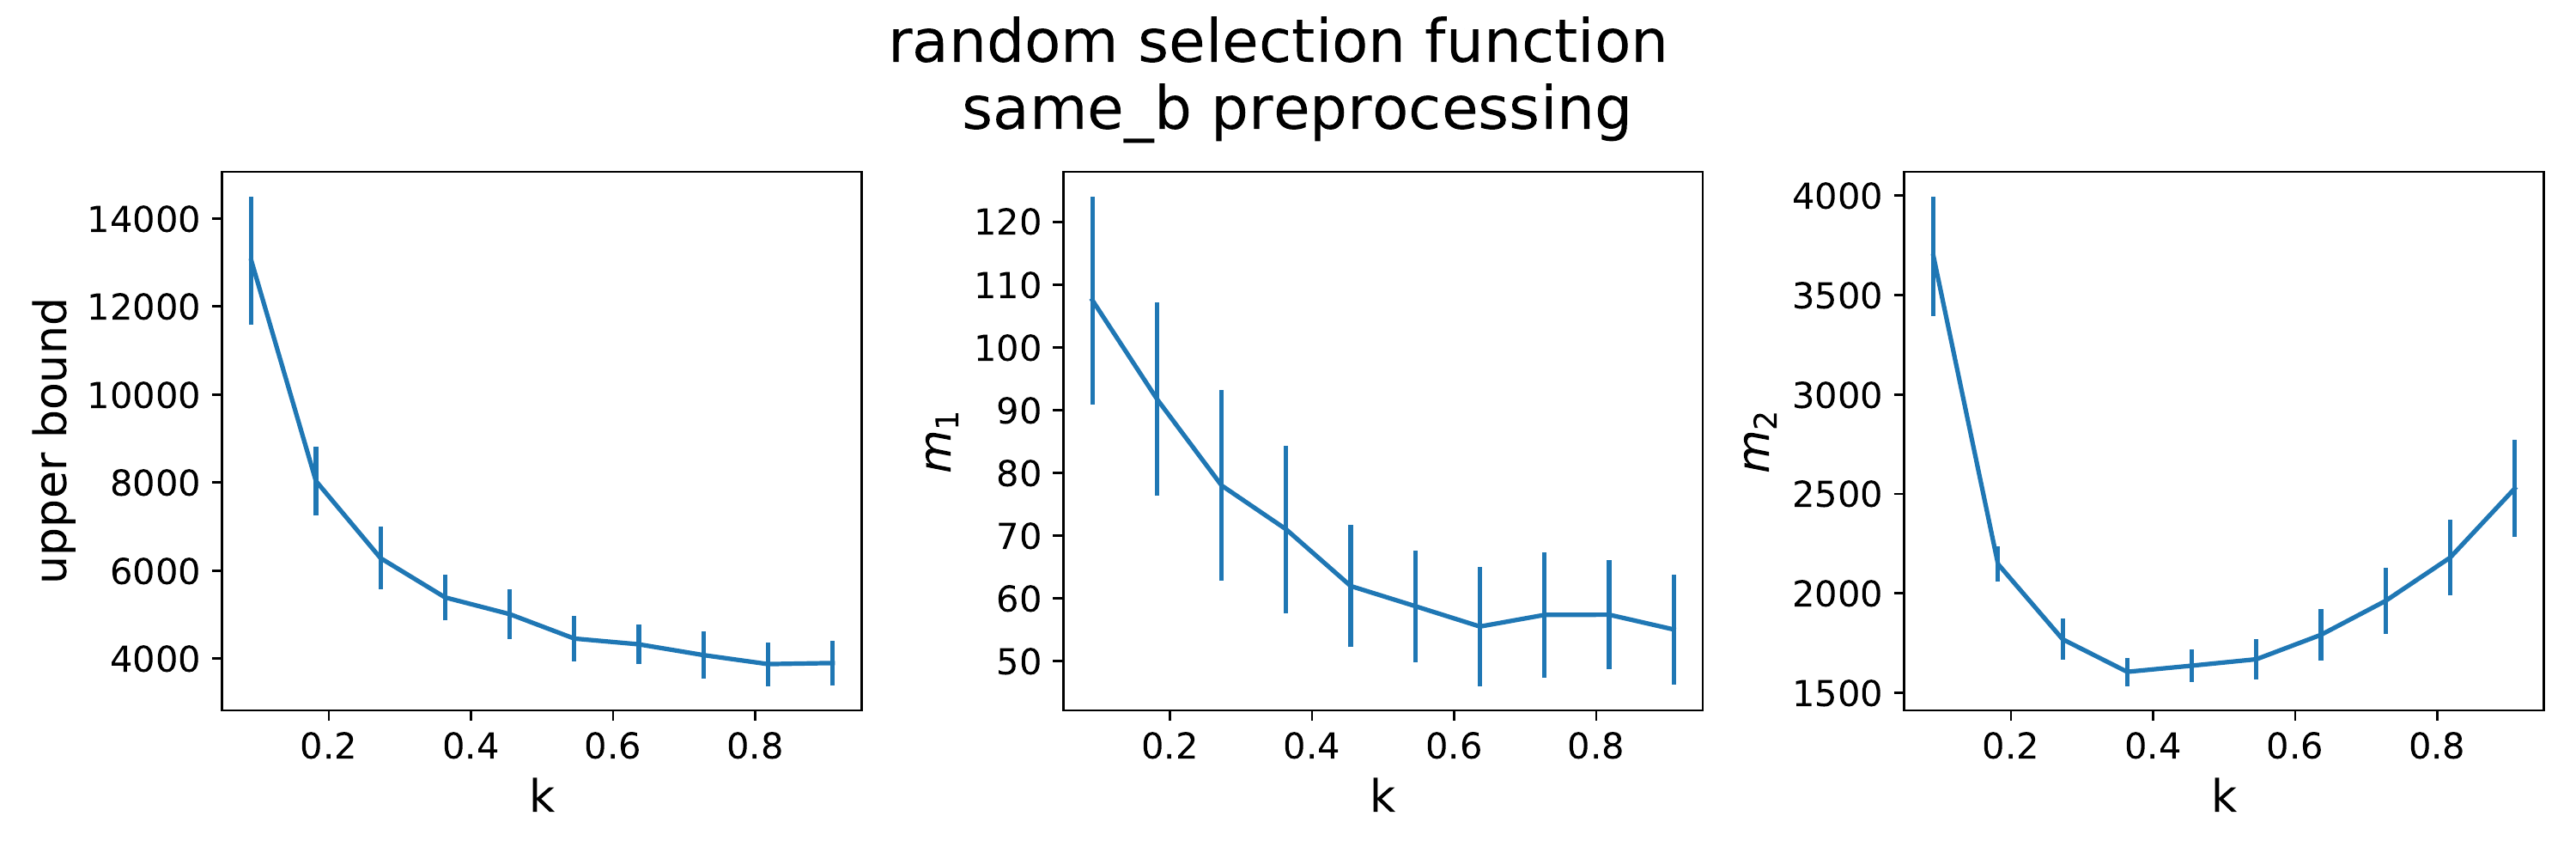}
   
 \includegraphics[width=1\linewidth]{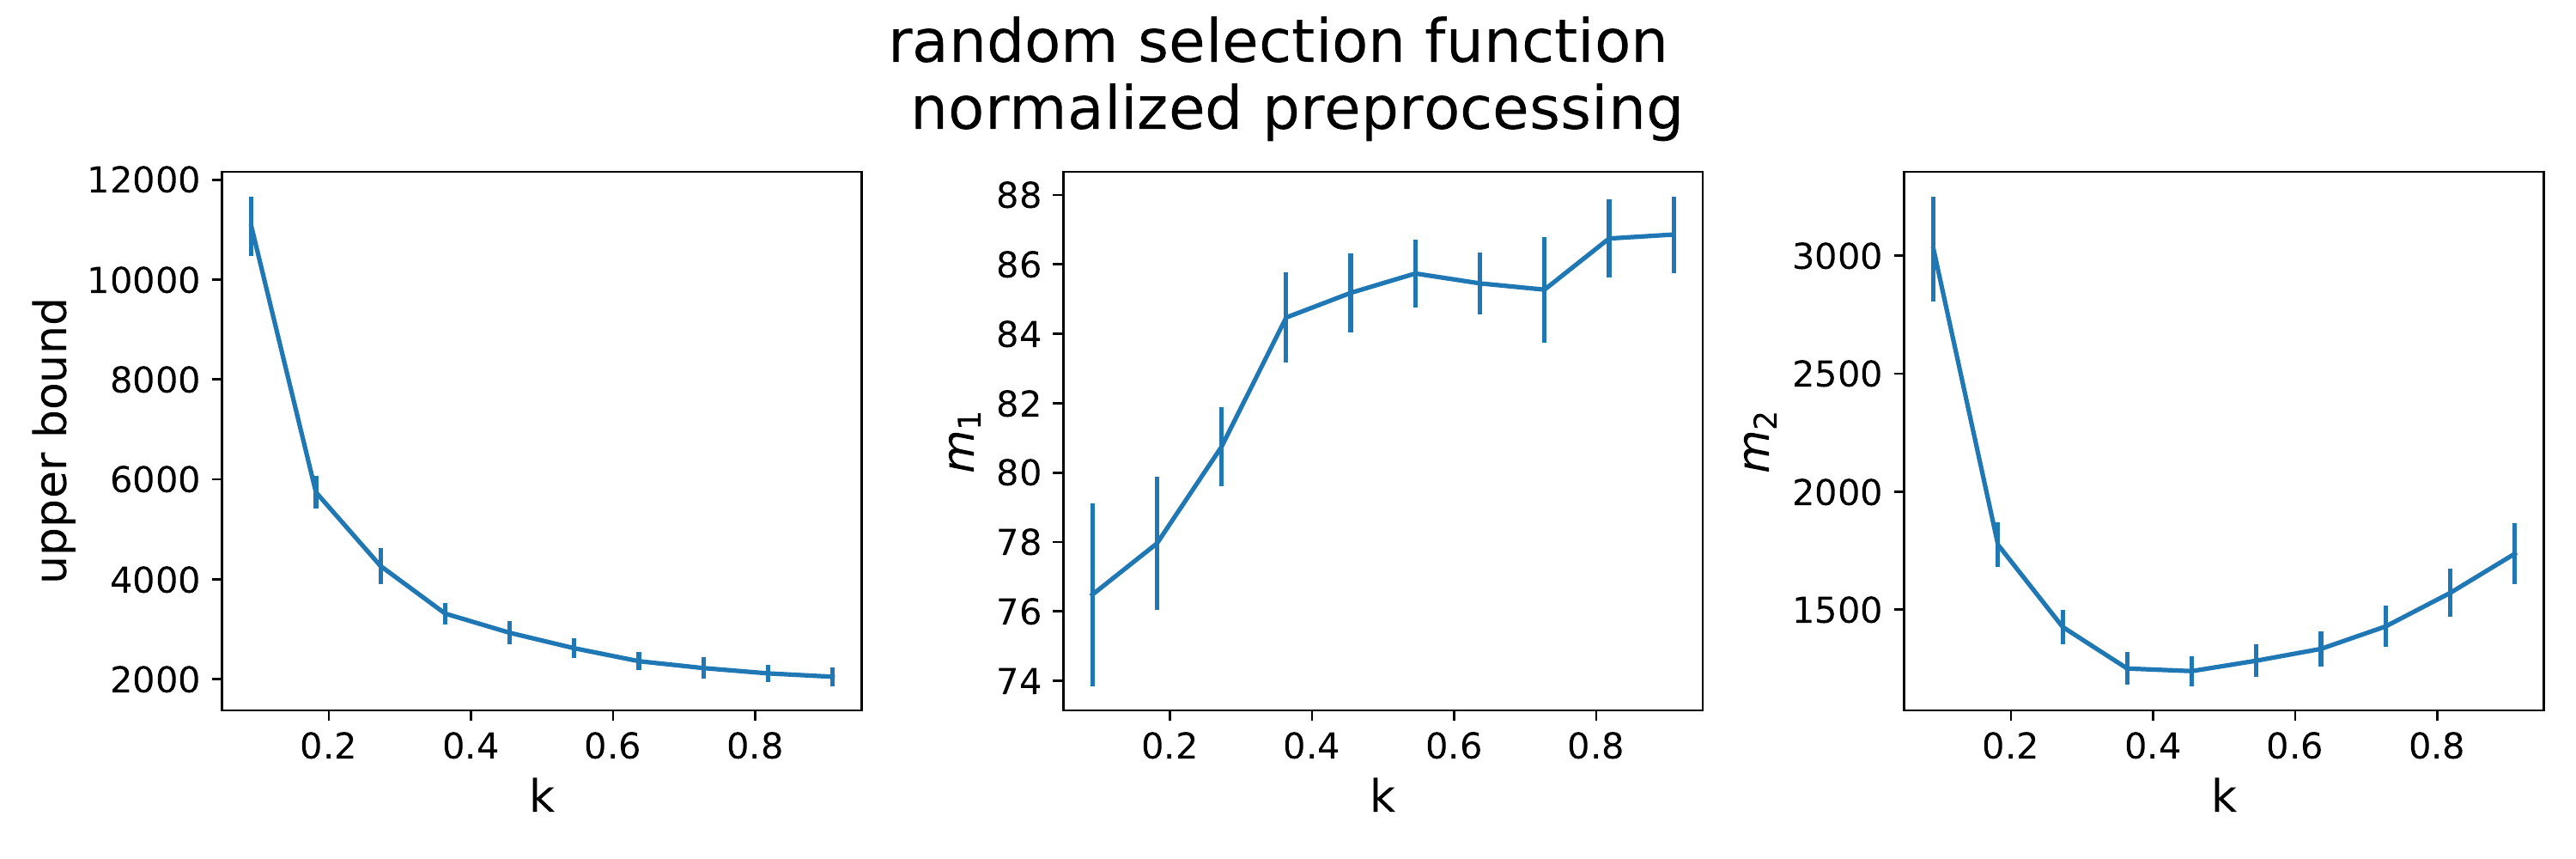}
 \caption{Number of samples and bound for ``random"}
\label{fig:samp,random}
\end{figure}

\begin{figure}
\centering

   \includegraphics[width=1\linewidth]{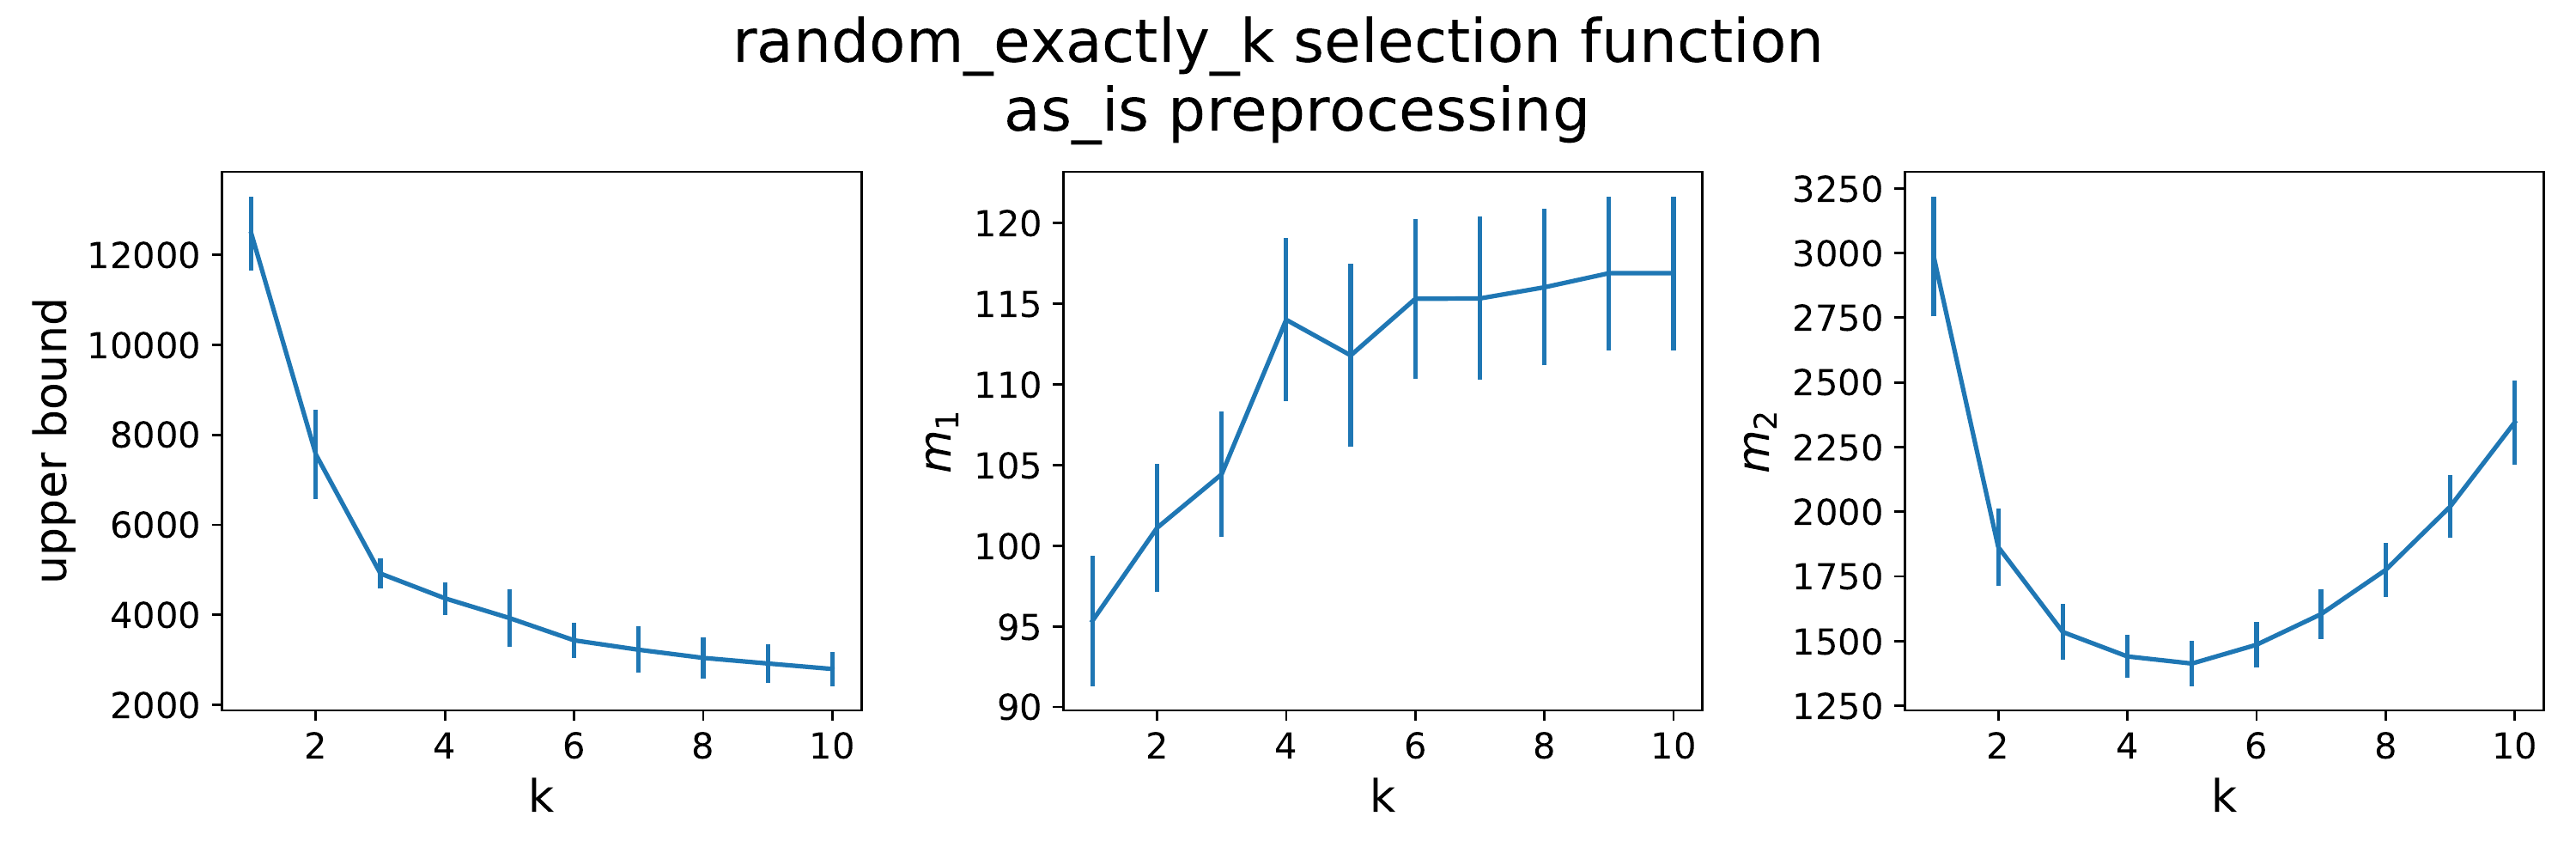}

 \includegraphics[width=1\linewidth]{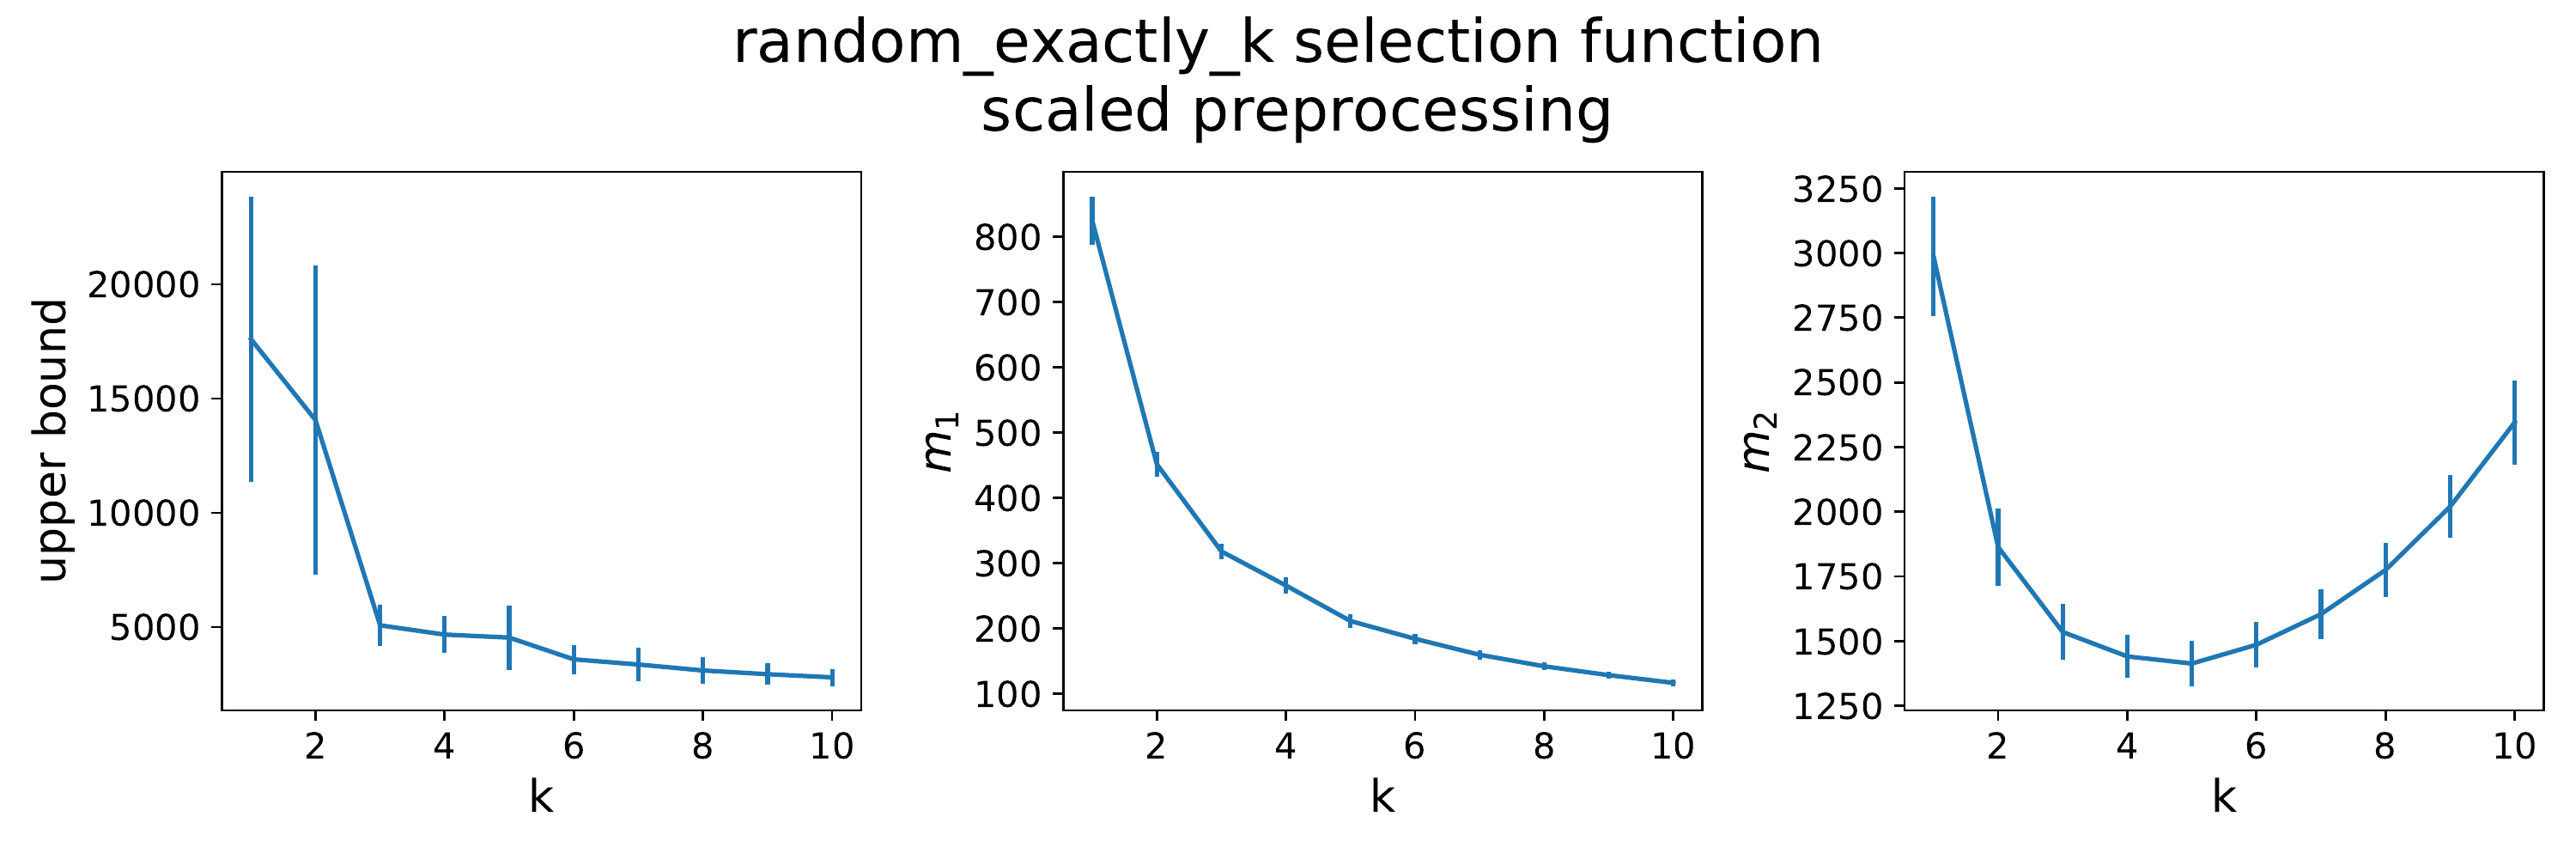}

    \includegraphics[width=1\linewidth]{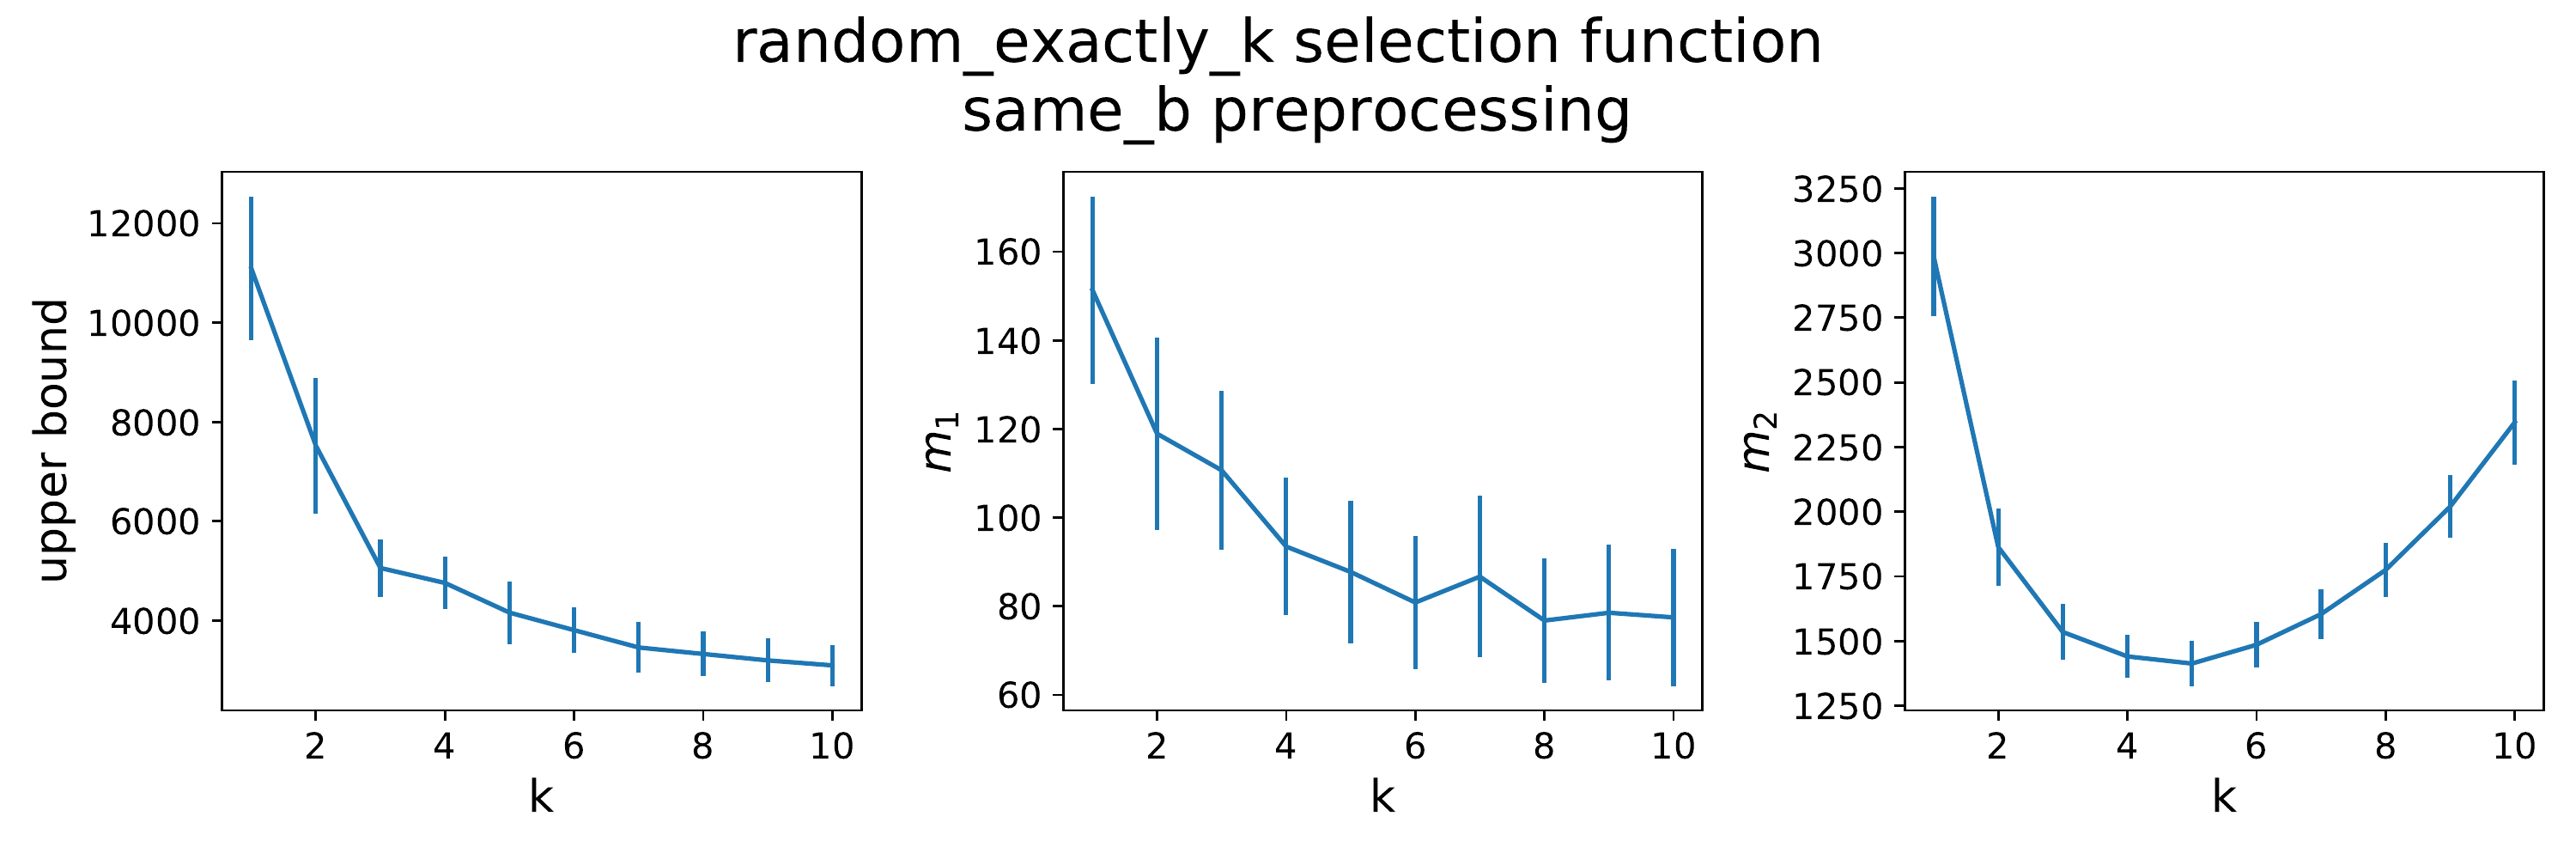}
   
 \includegraphics[width=1\linewidth]{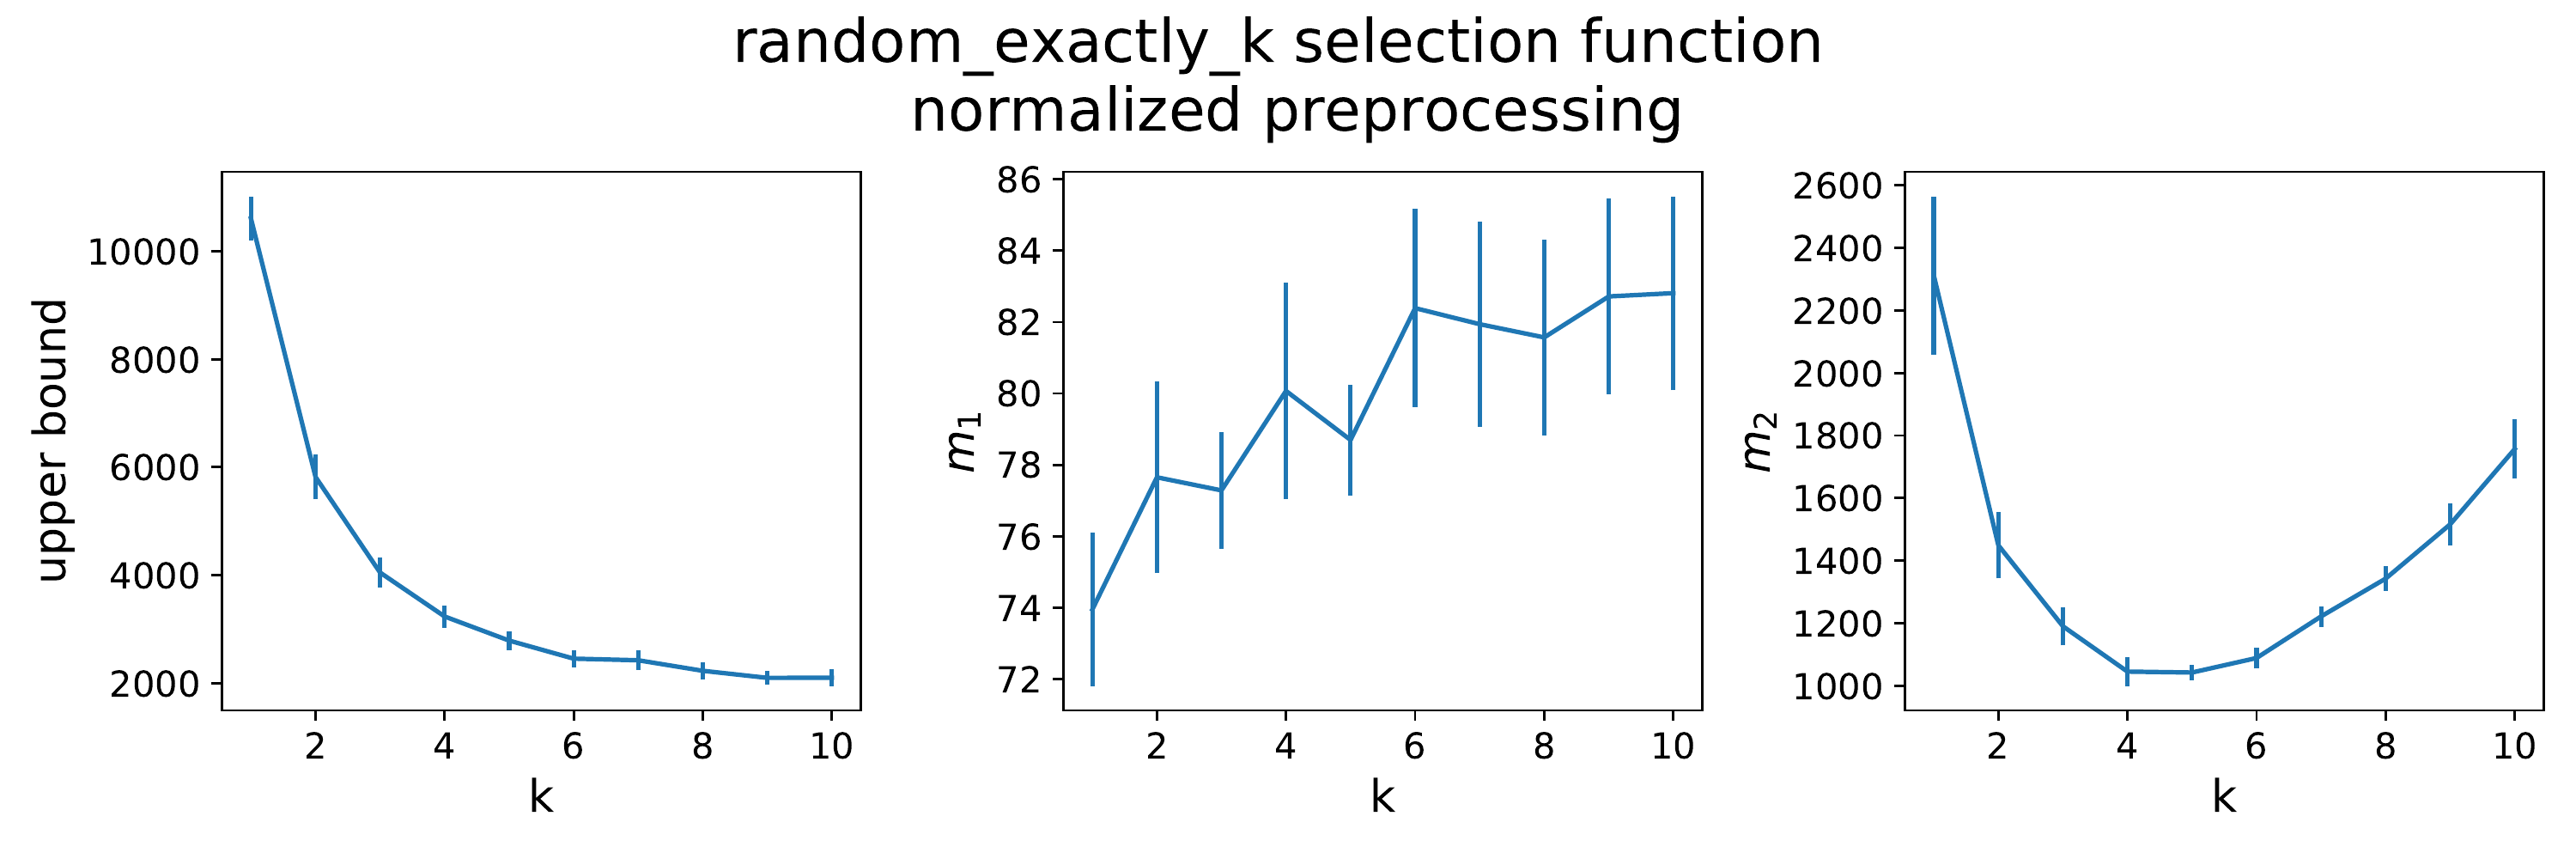}
  \caption{Number of samples and bound for ``random exactly $k$"}
\label{fig:samp,random exaclty k}
\end{figure}

\begin{figure}
\centering

   \includegraphics[width=1\linewidth]{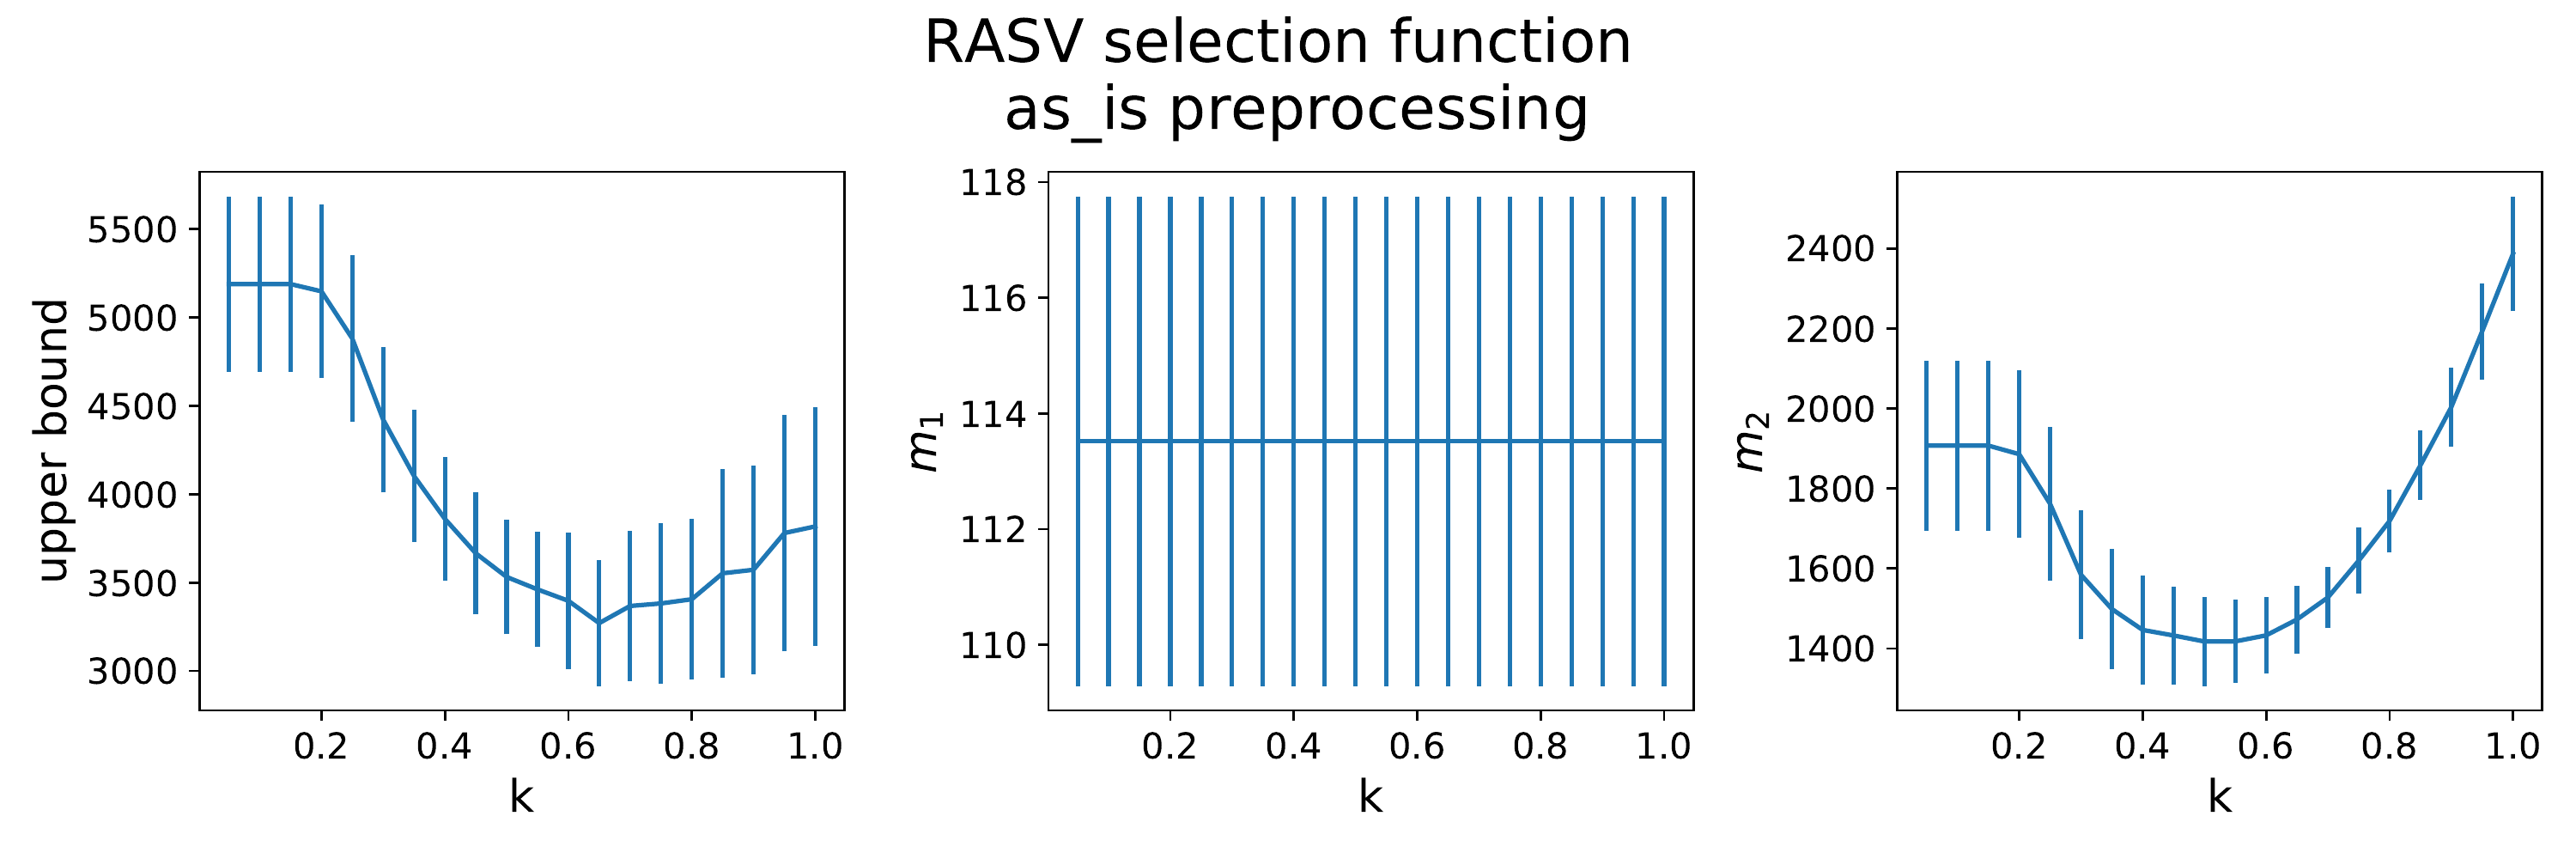}

    \includegraphics[width=1\linewidth]{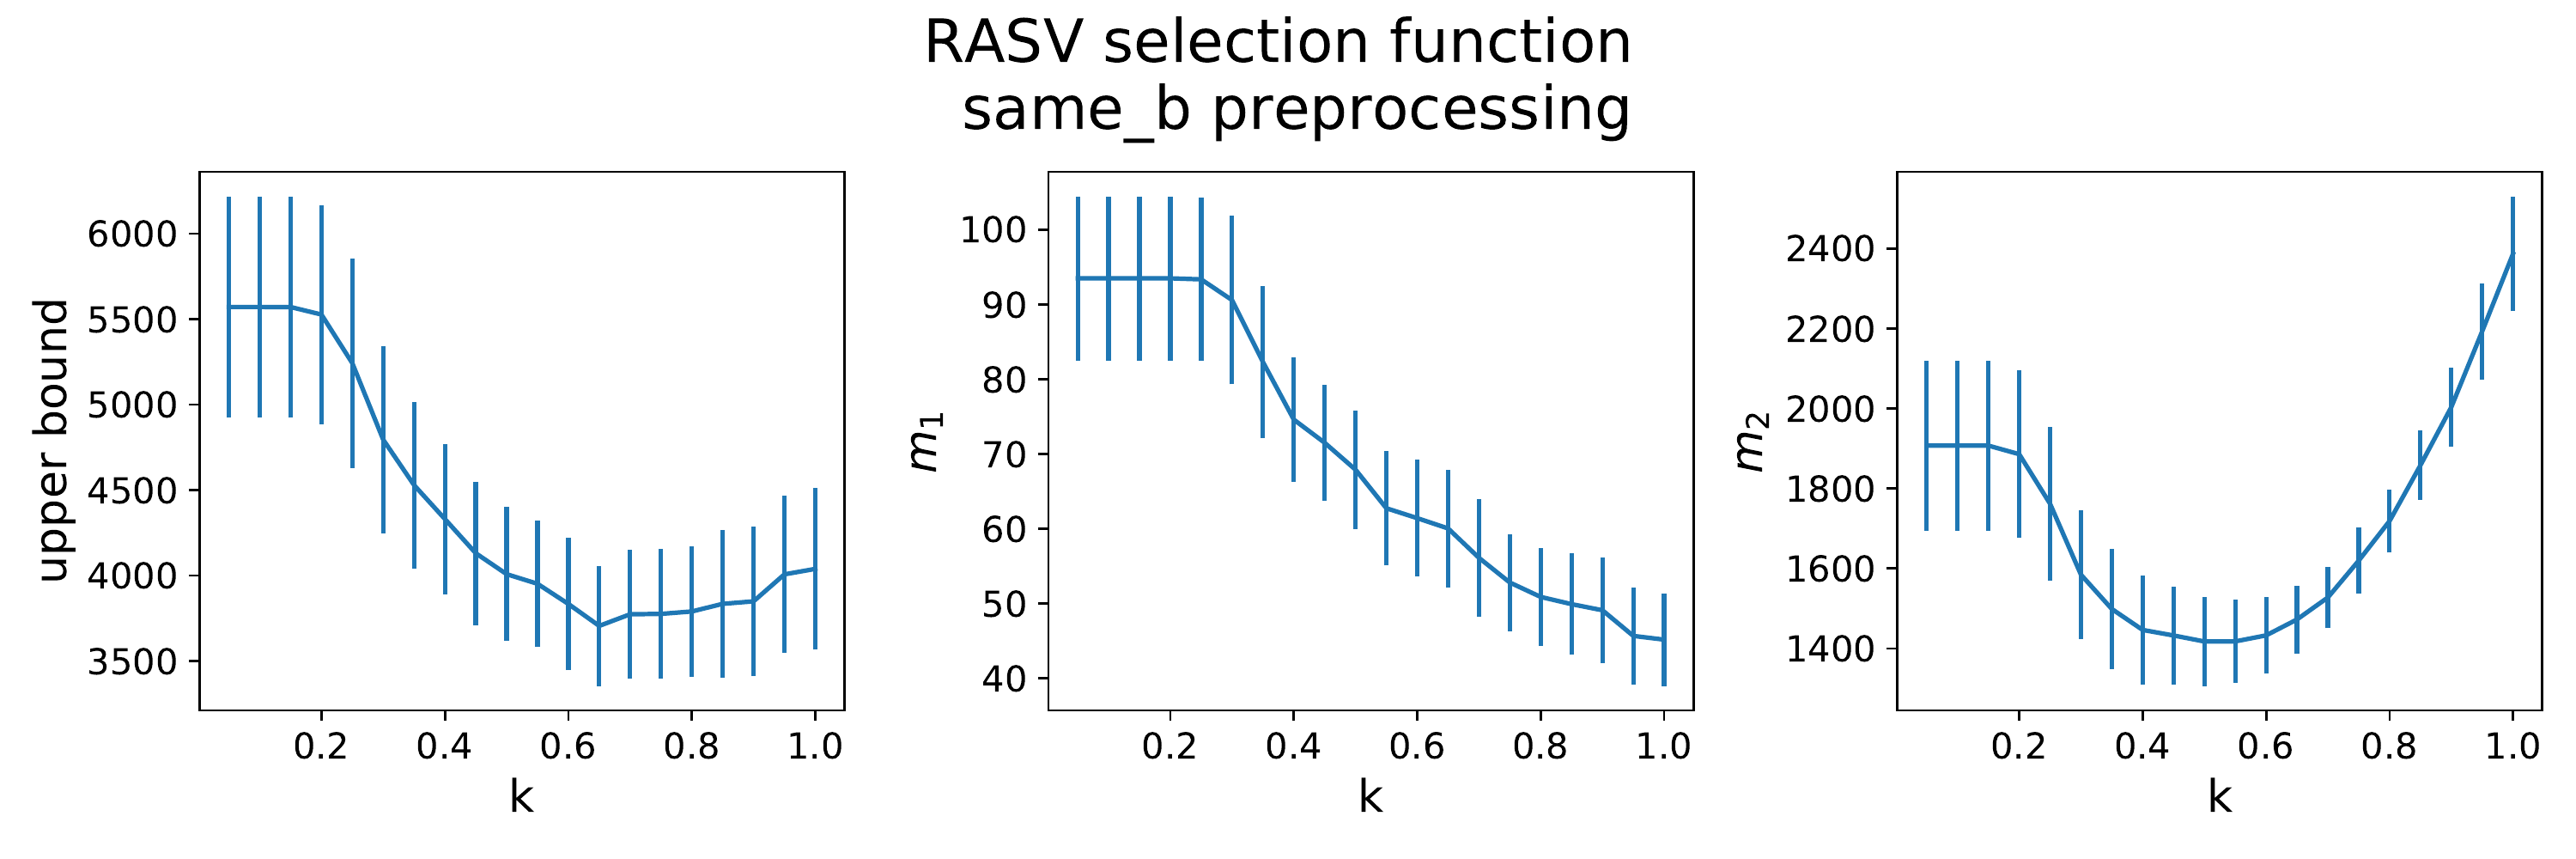}
   
 \includegraphics[width=1\linewidth]{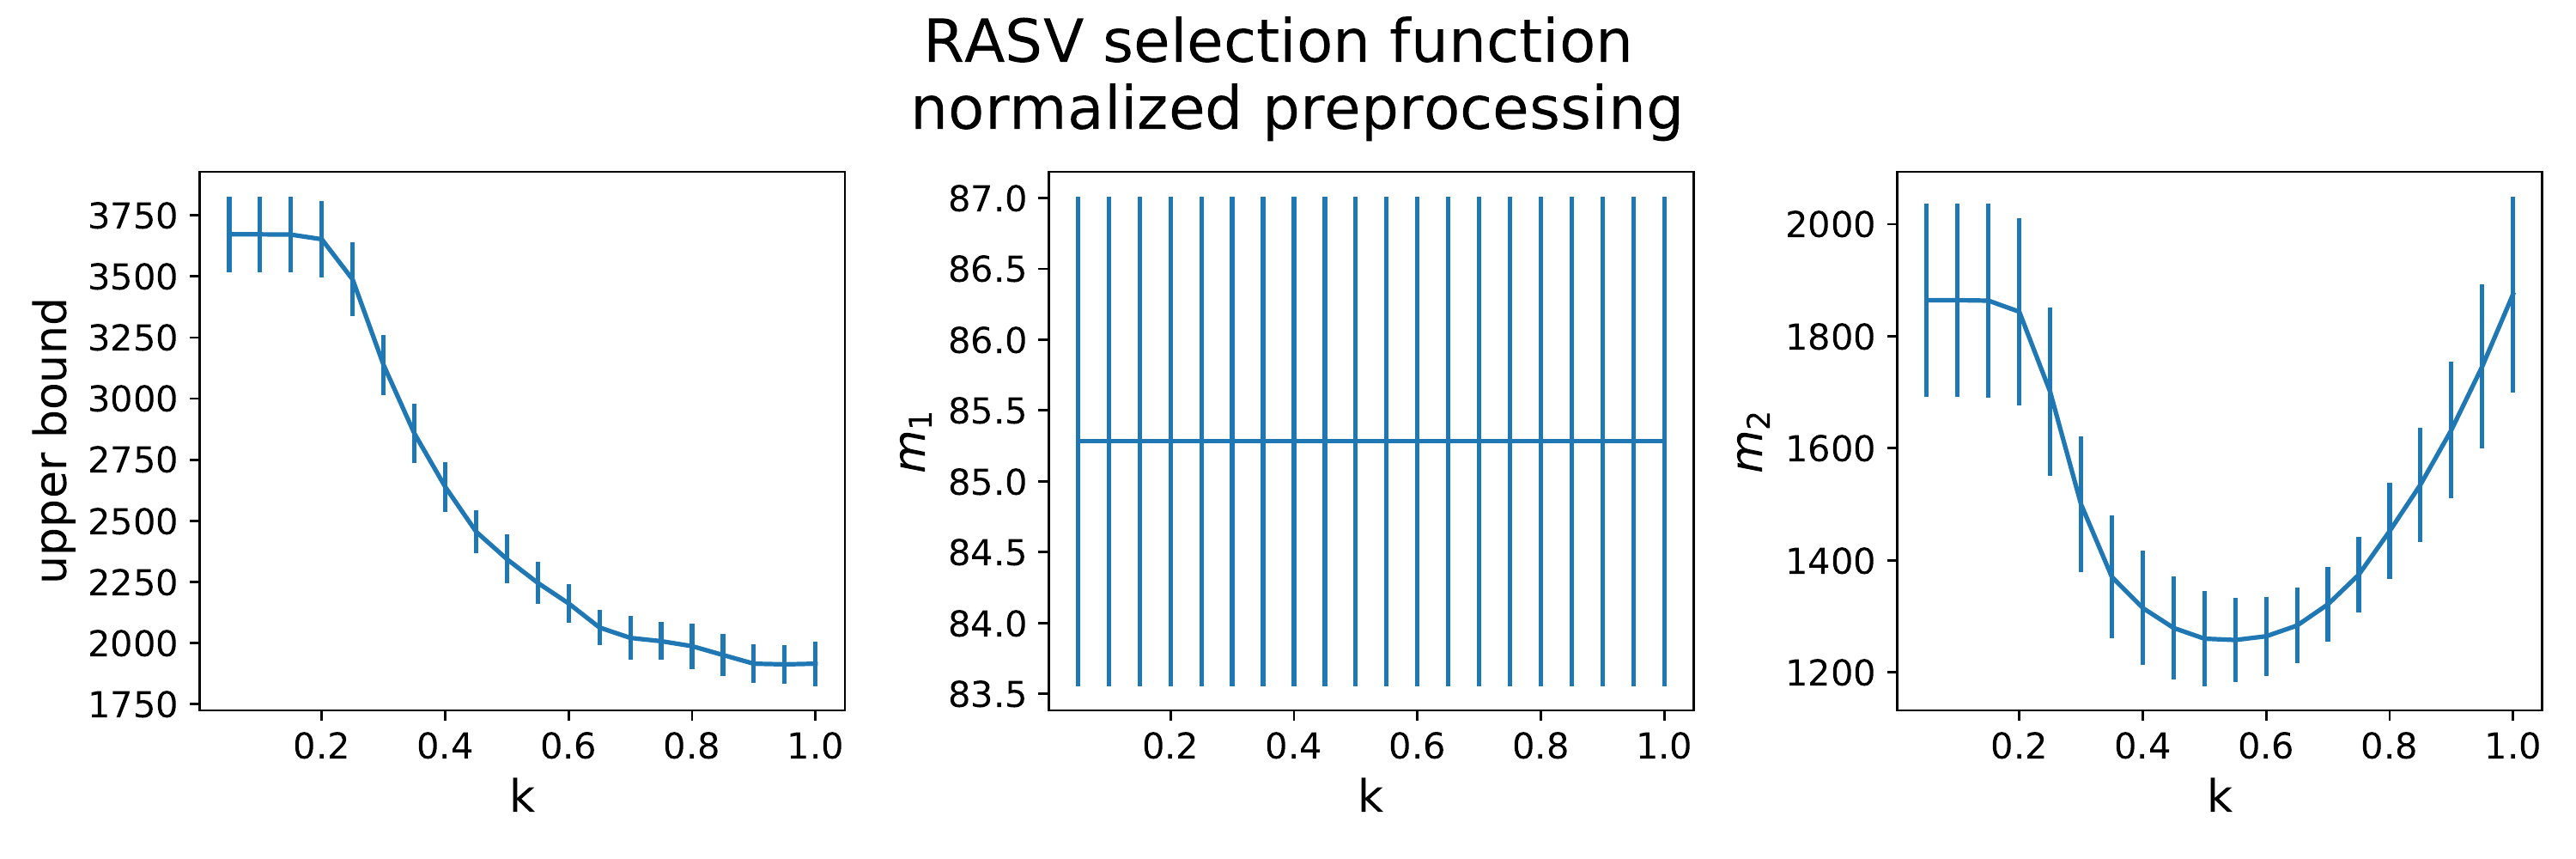}
   \caption{Number of samples and bound for RASV}
\label{fig:samp,rasv}
\end{figure}

\begin{figure}
\centering

   \includegraphics[width=1\linewidth]{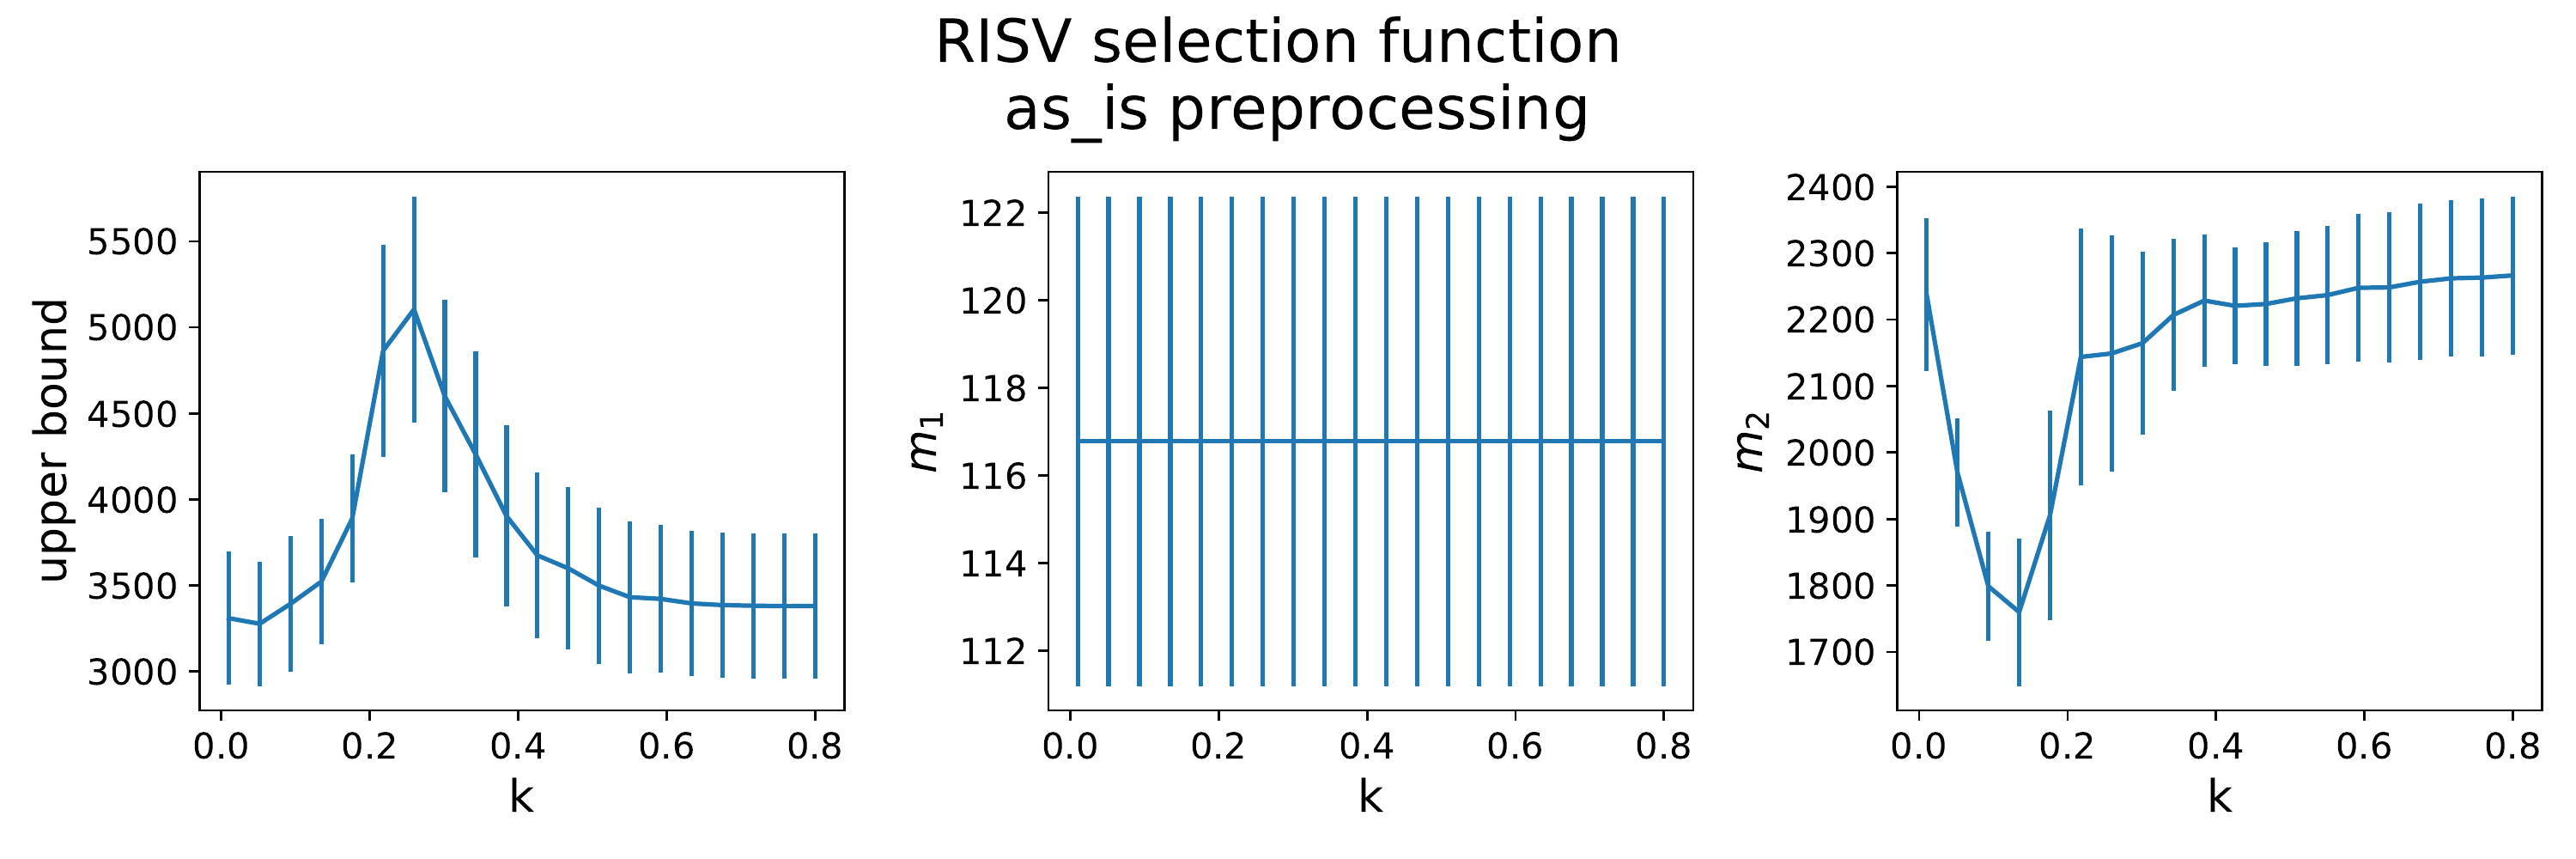}

    \includegraphics[width=1\linewidth]{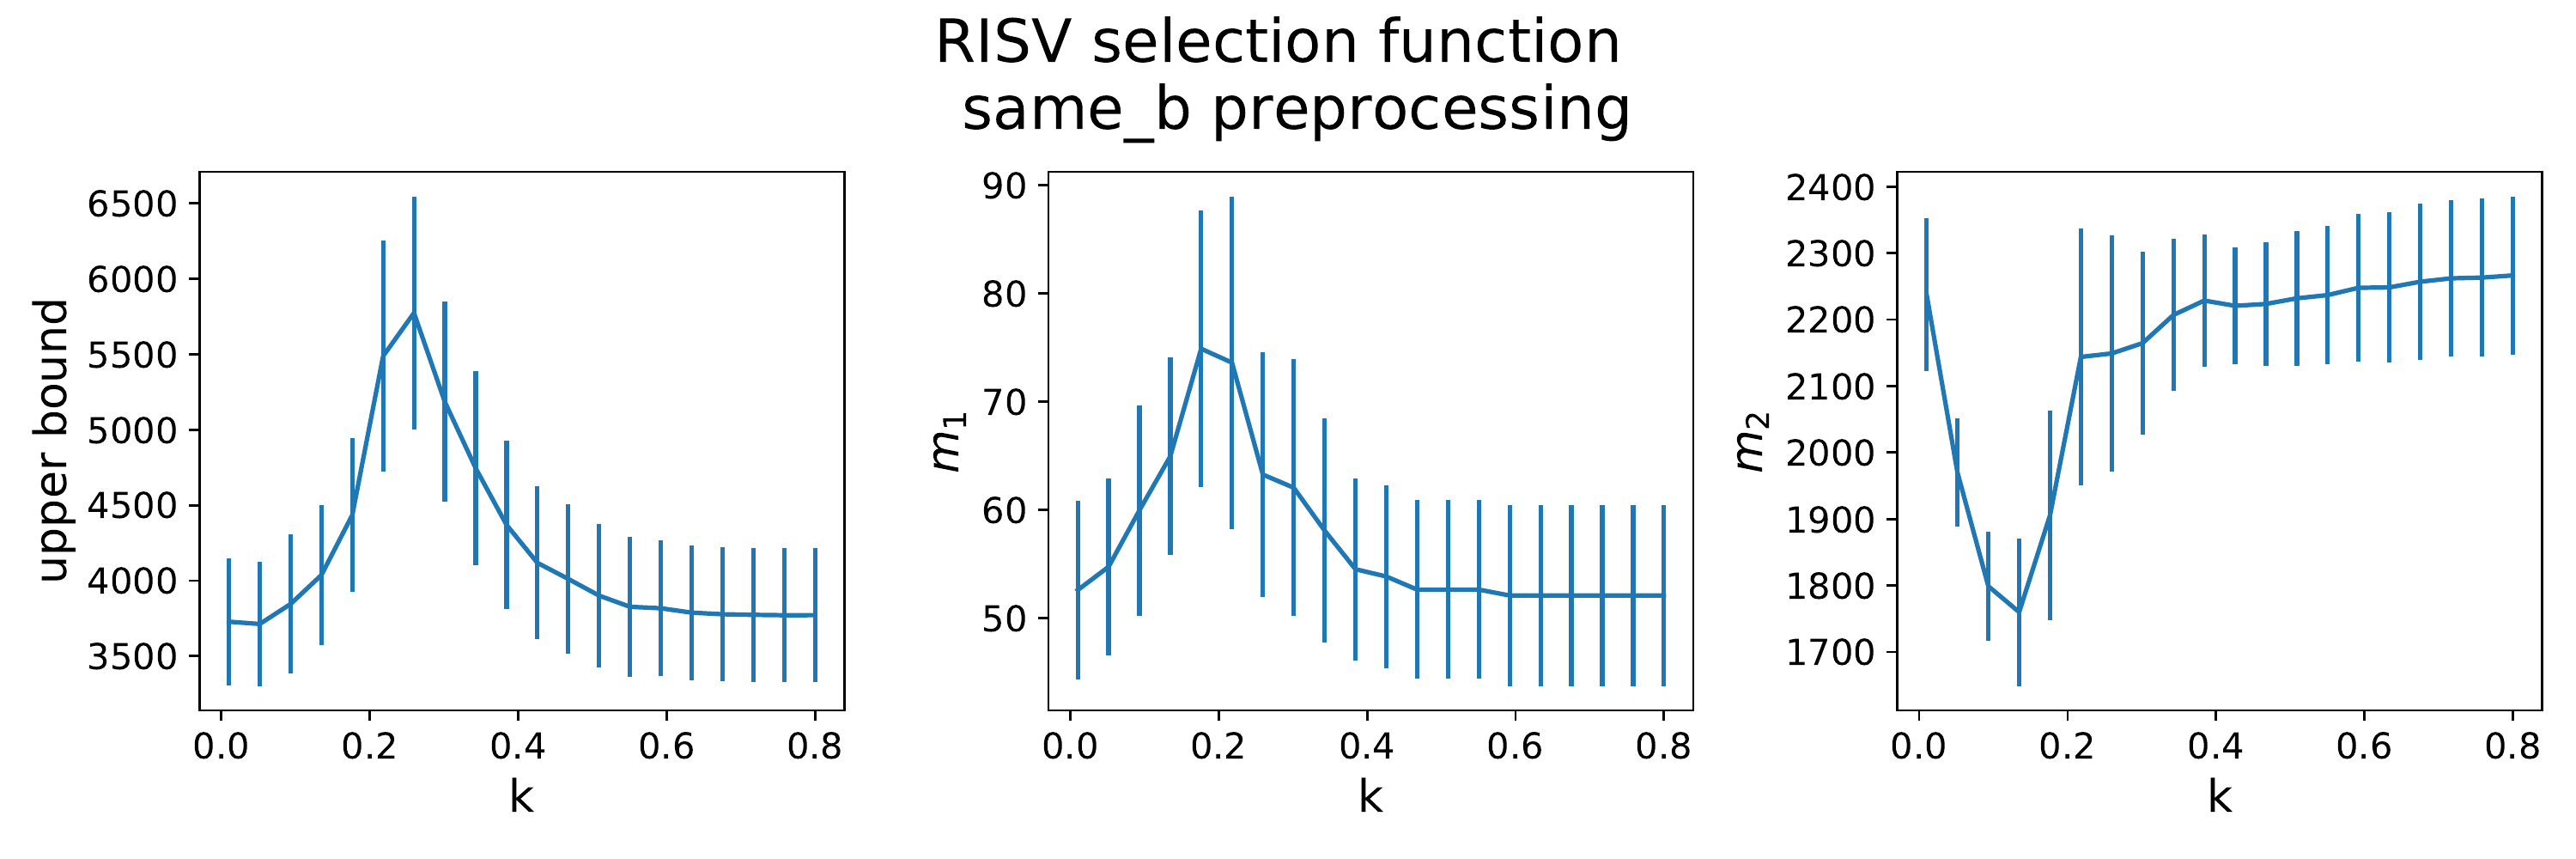}
   
 \includegraphics[width=1\linewidth]{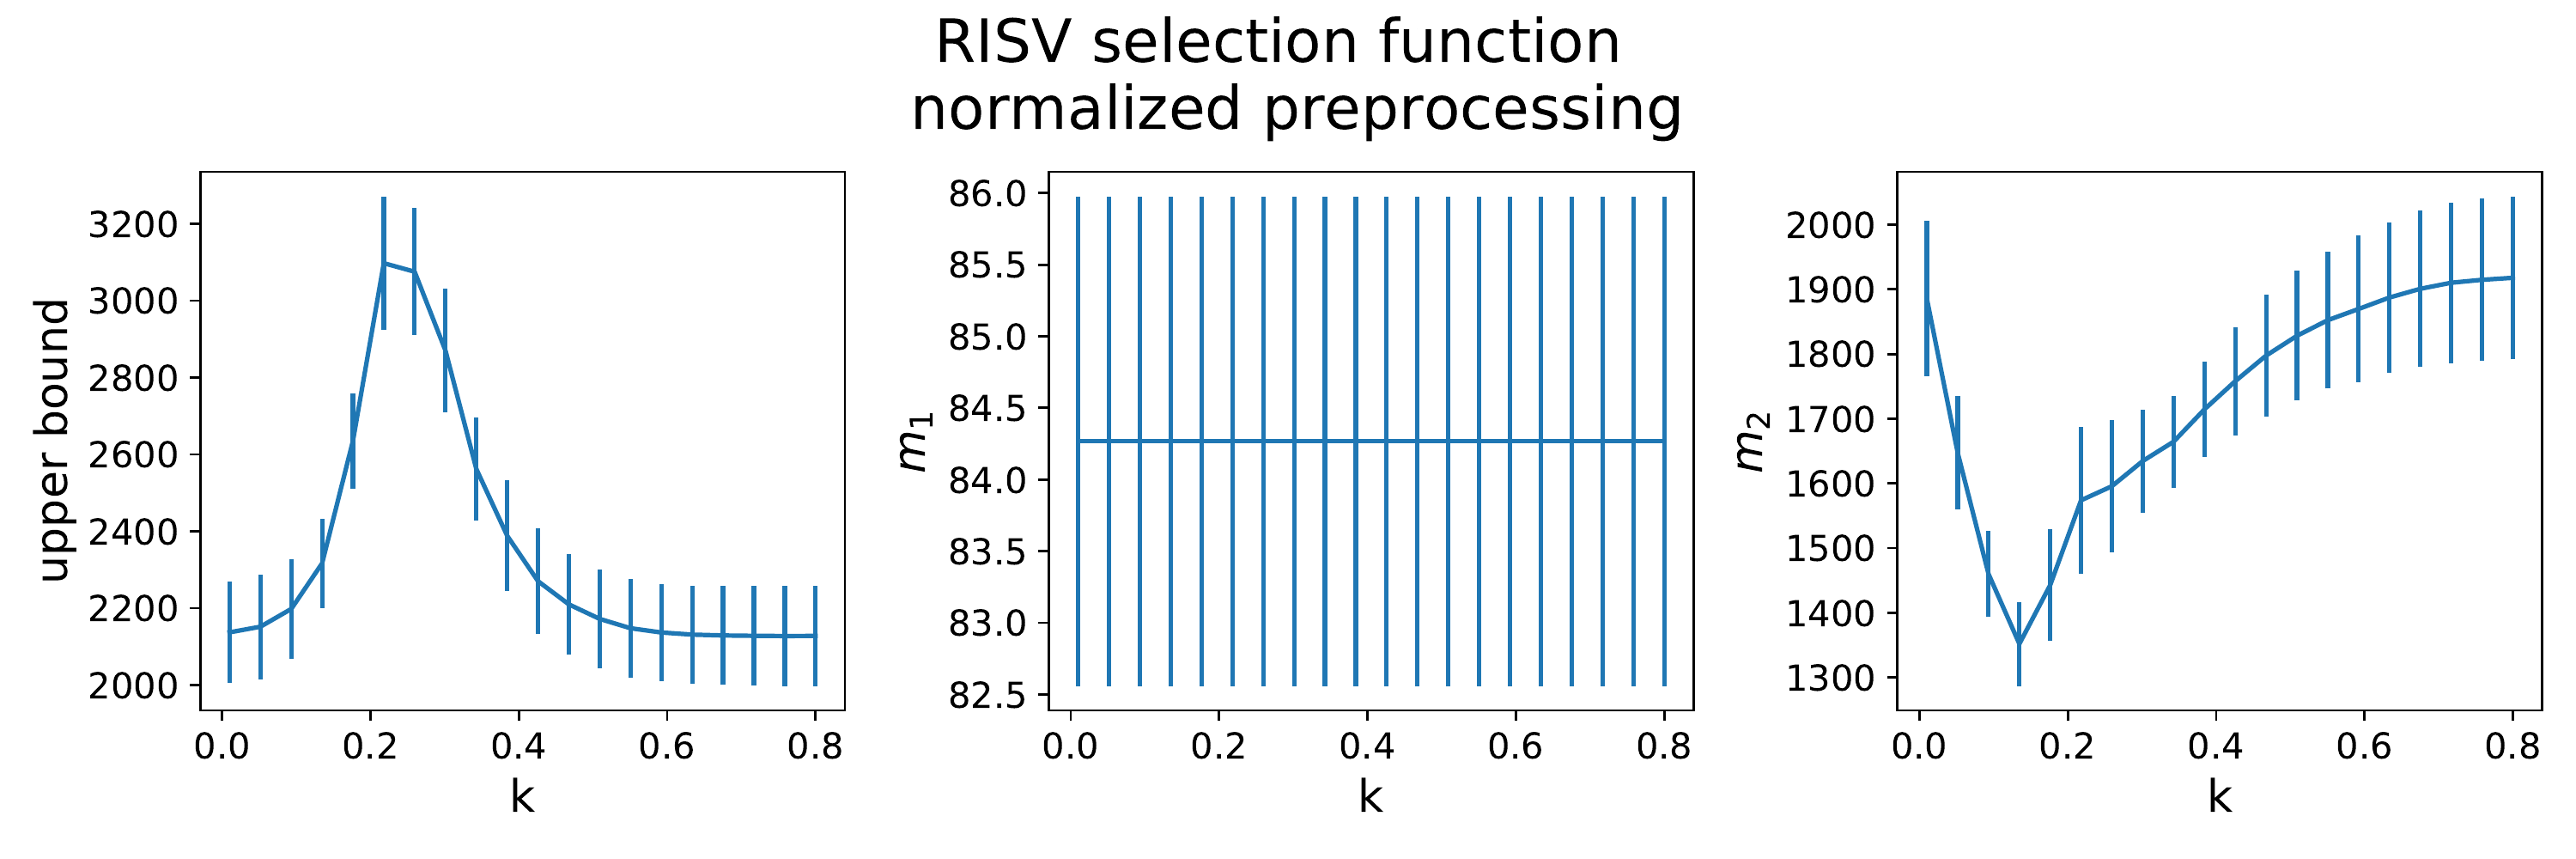}
    \caption{Number of samples and bound for RISV}
\label{fig:samp,risv}
\end{figure}

\subsection{Intransitivties and pairwise inconsistencies}
\begin{figure}
\centering

   \includegraphics[width=8cm]{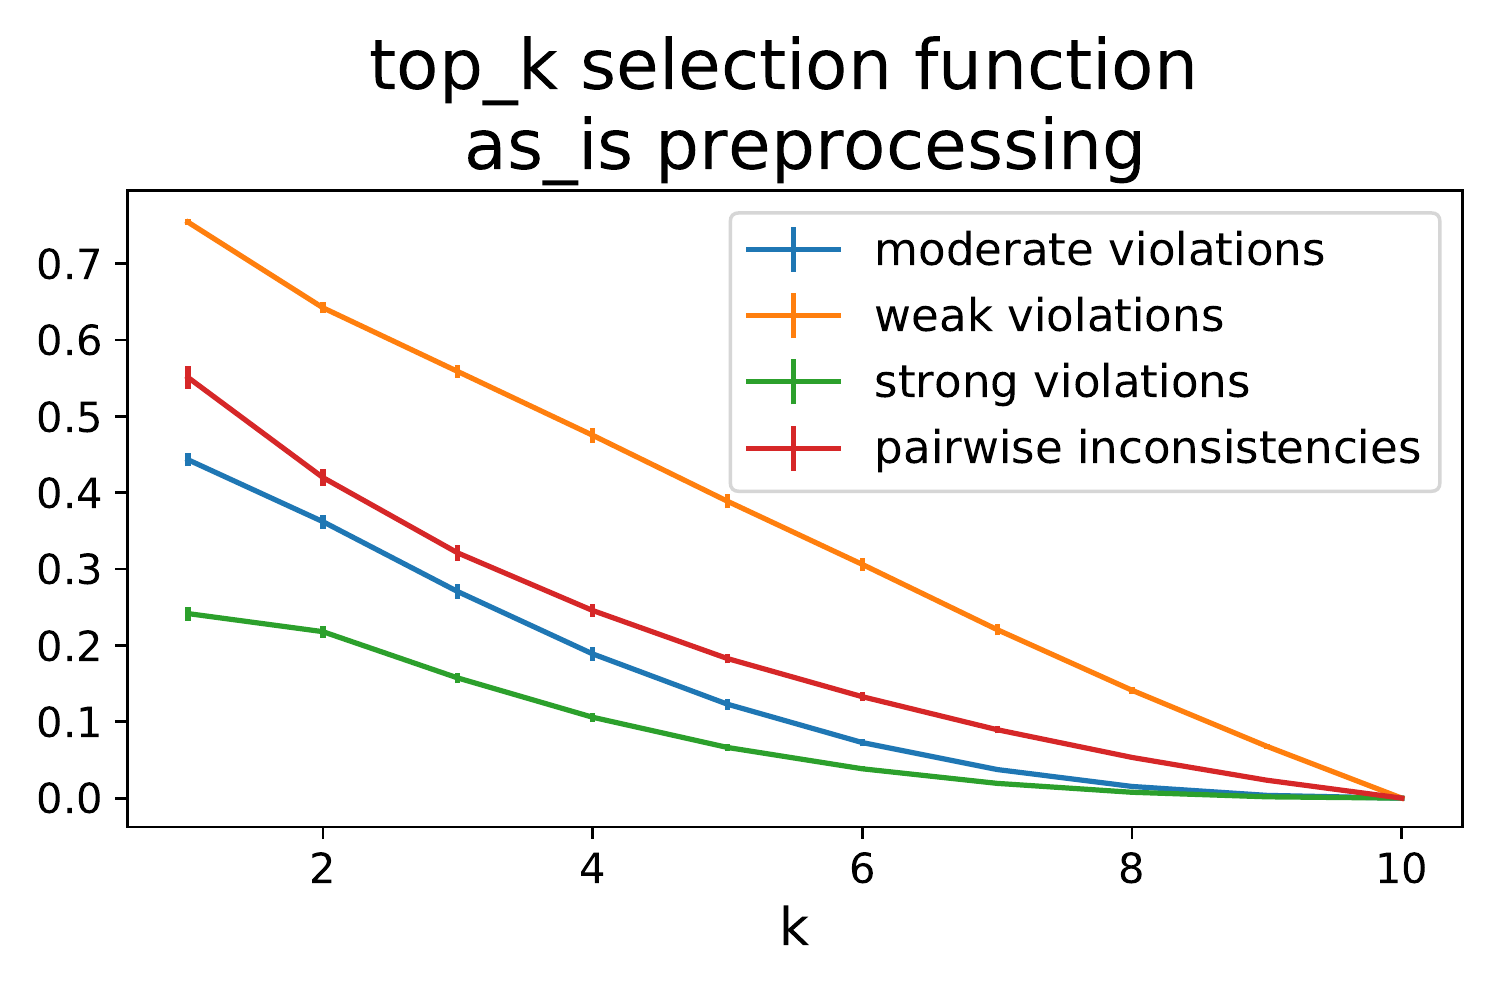}

 \includegraphics[width=8cm]{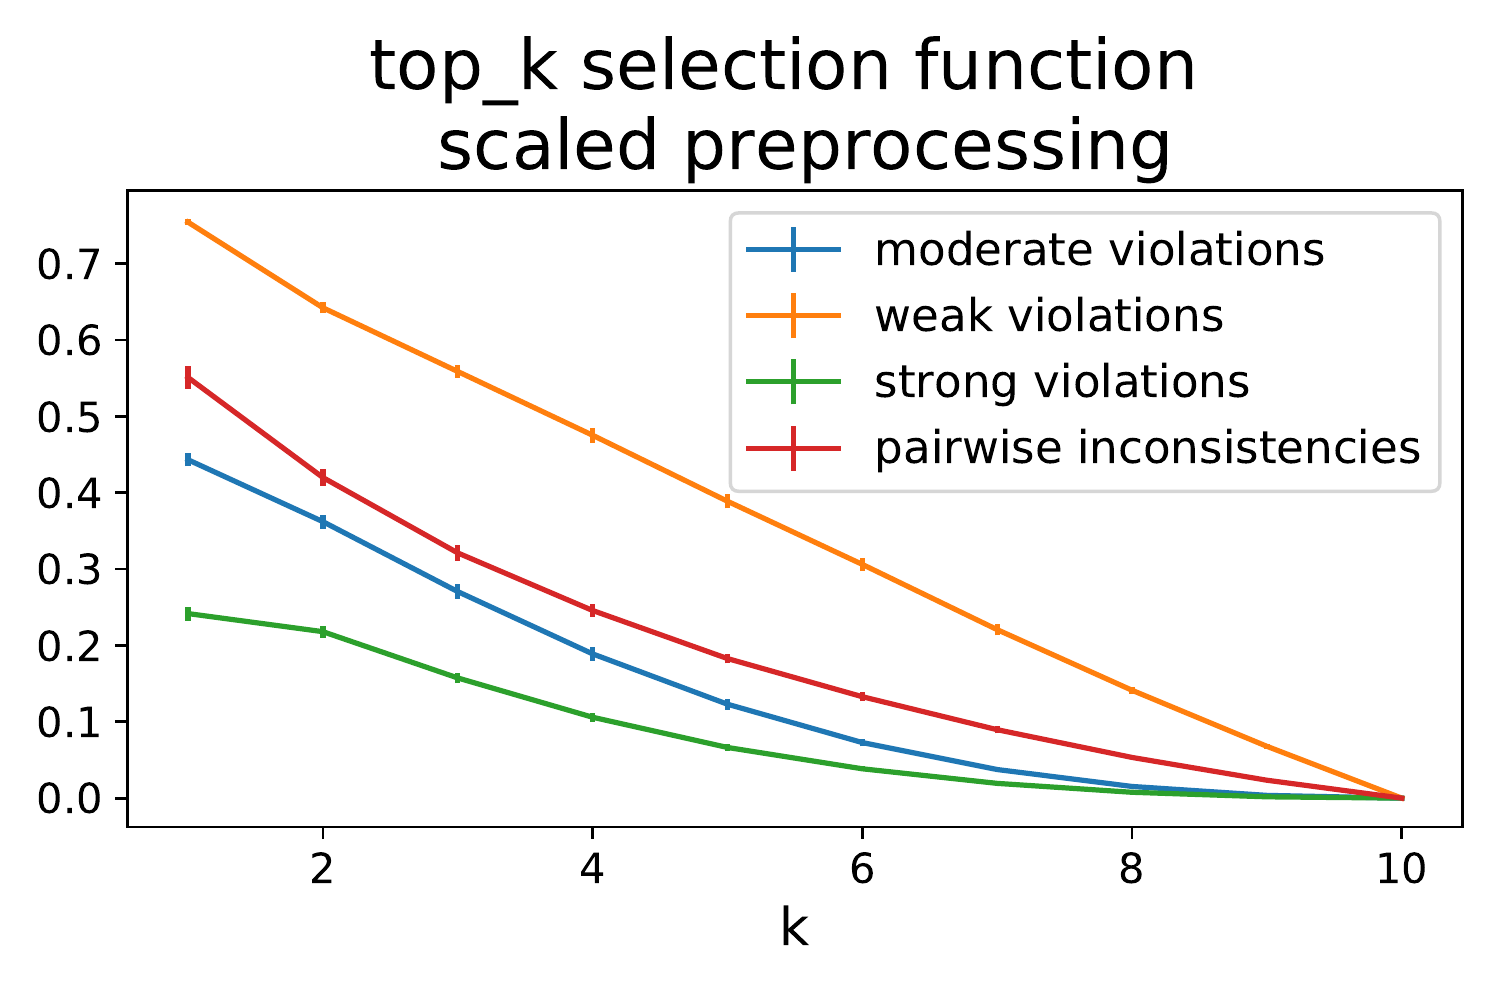}

    \includegraphics[width=8cm]{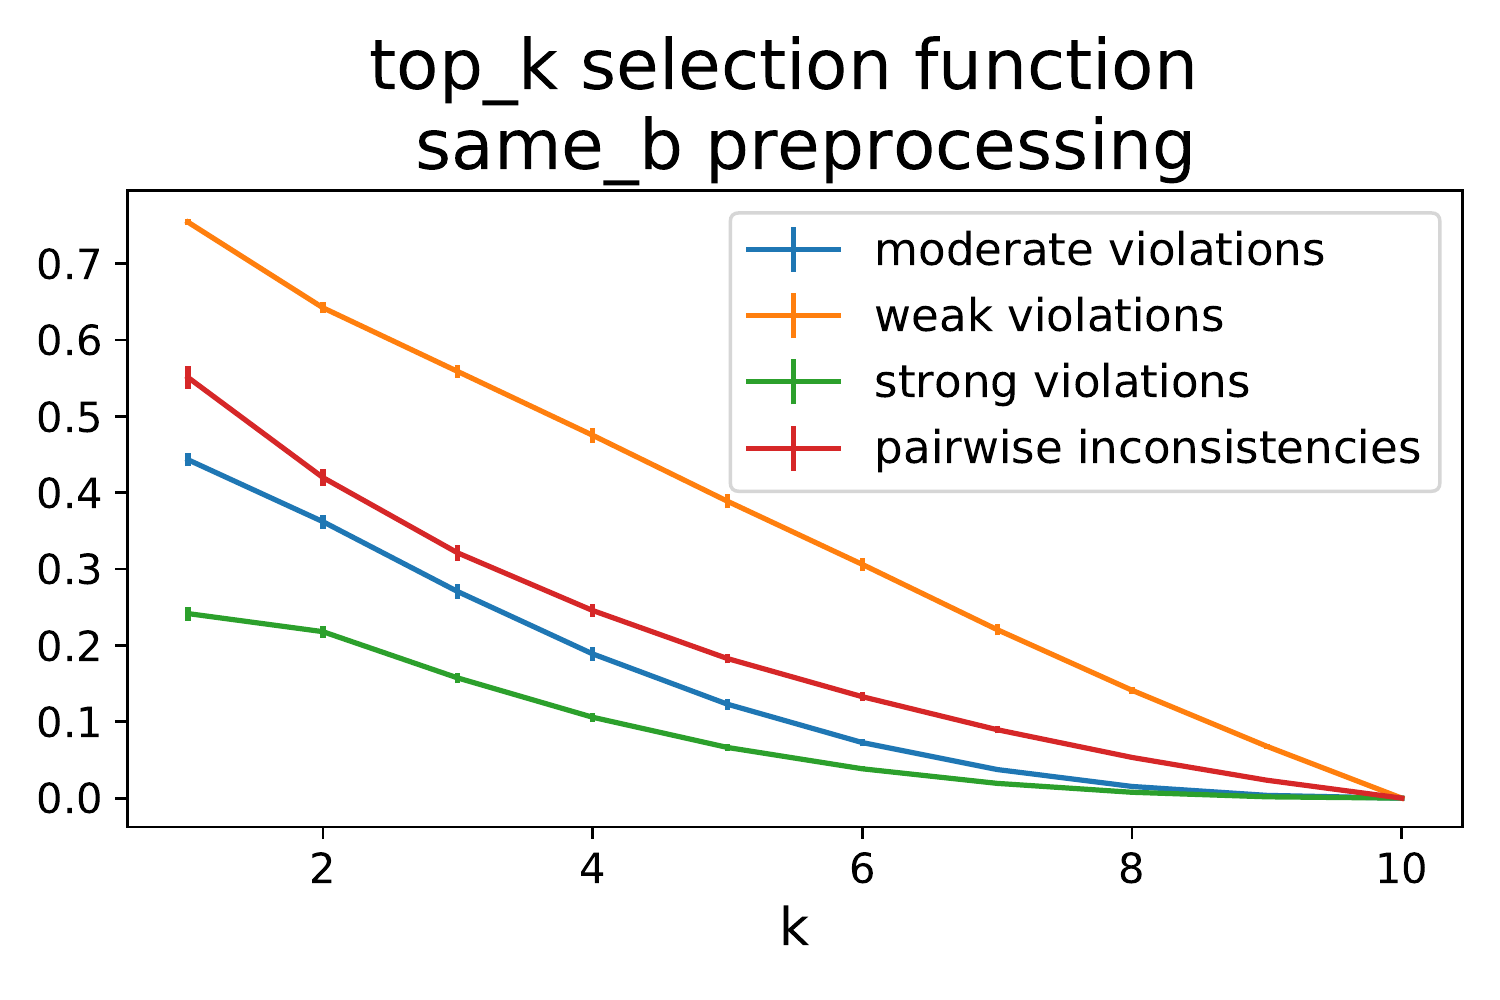}
   
 \includegraphics[width=8cm]{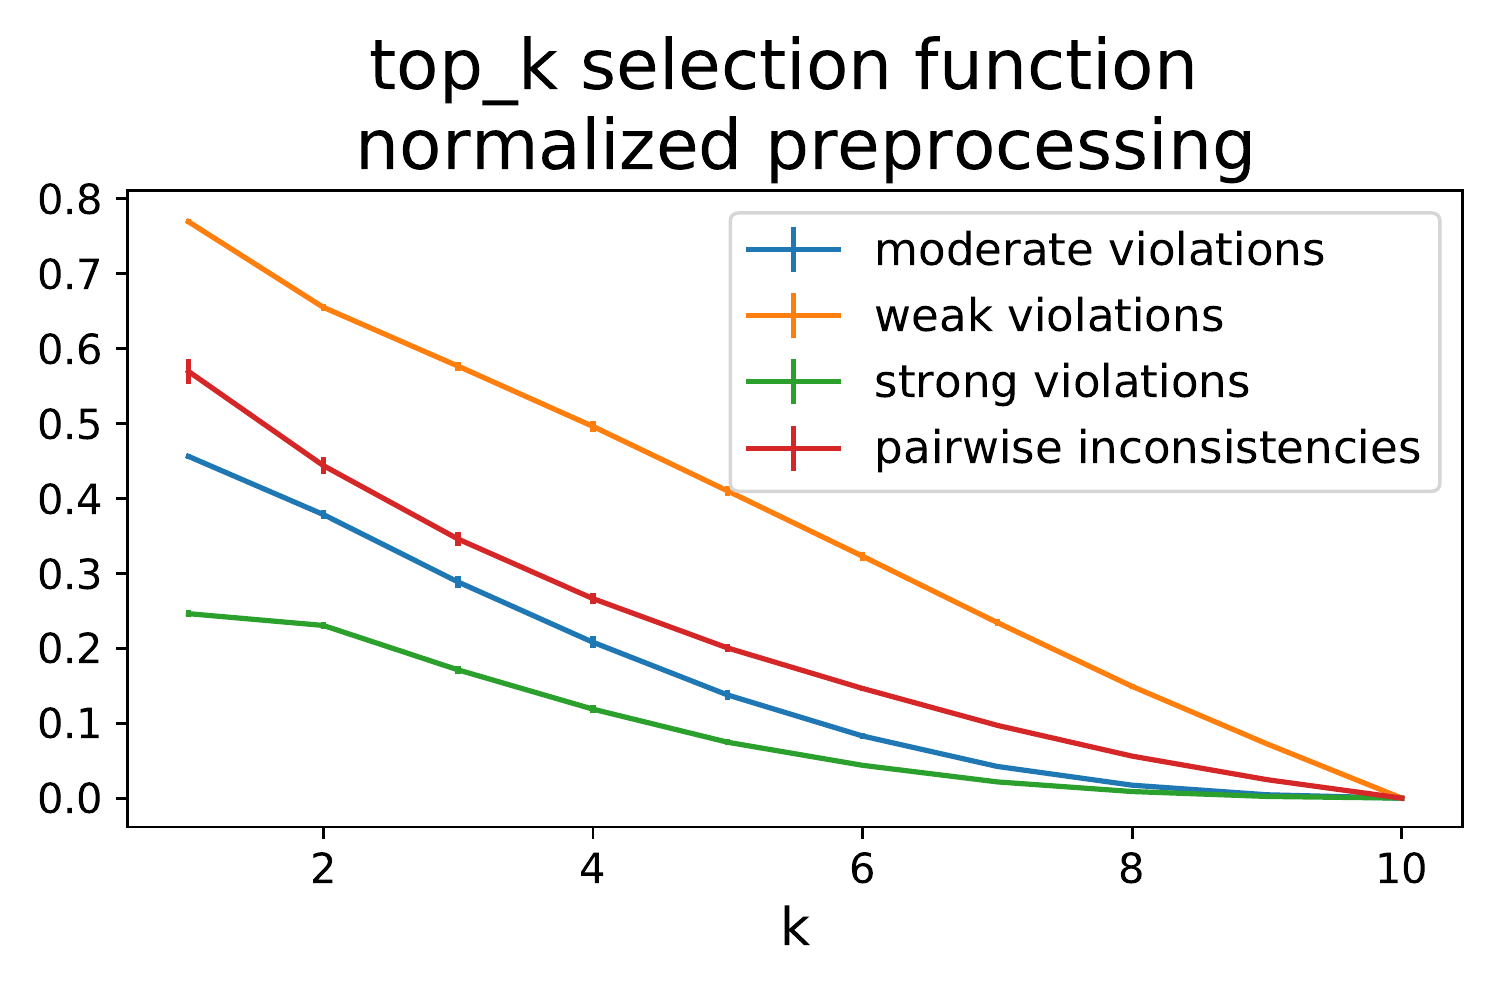}

    \caption{Number of samples and bound for ``top $k$"}
\label{fig:sst, top k}
\end{figure}

\begin{figure}
\centering

   \includegraphics[width=8cm]{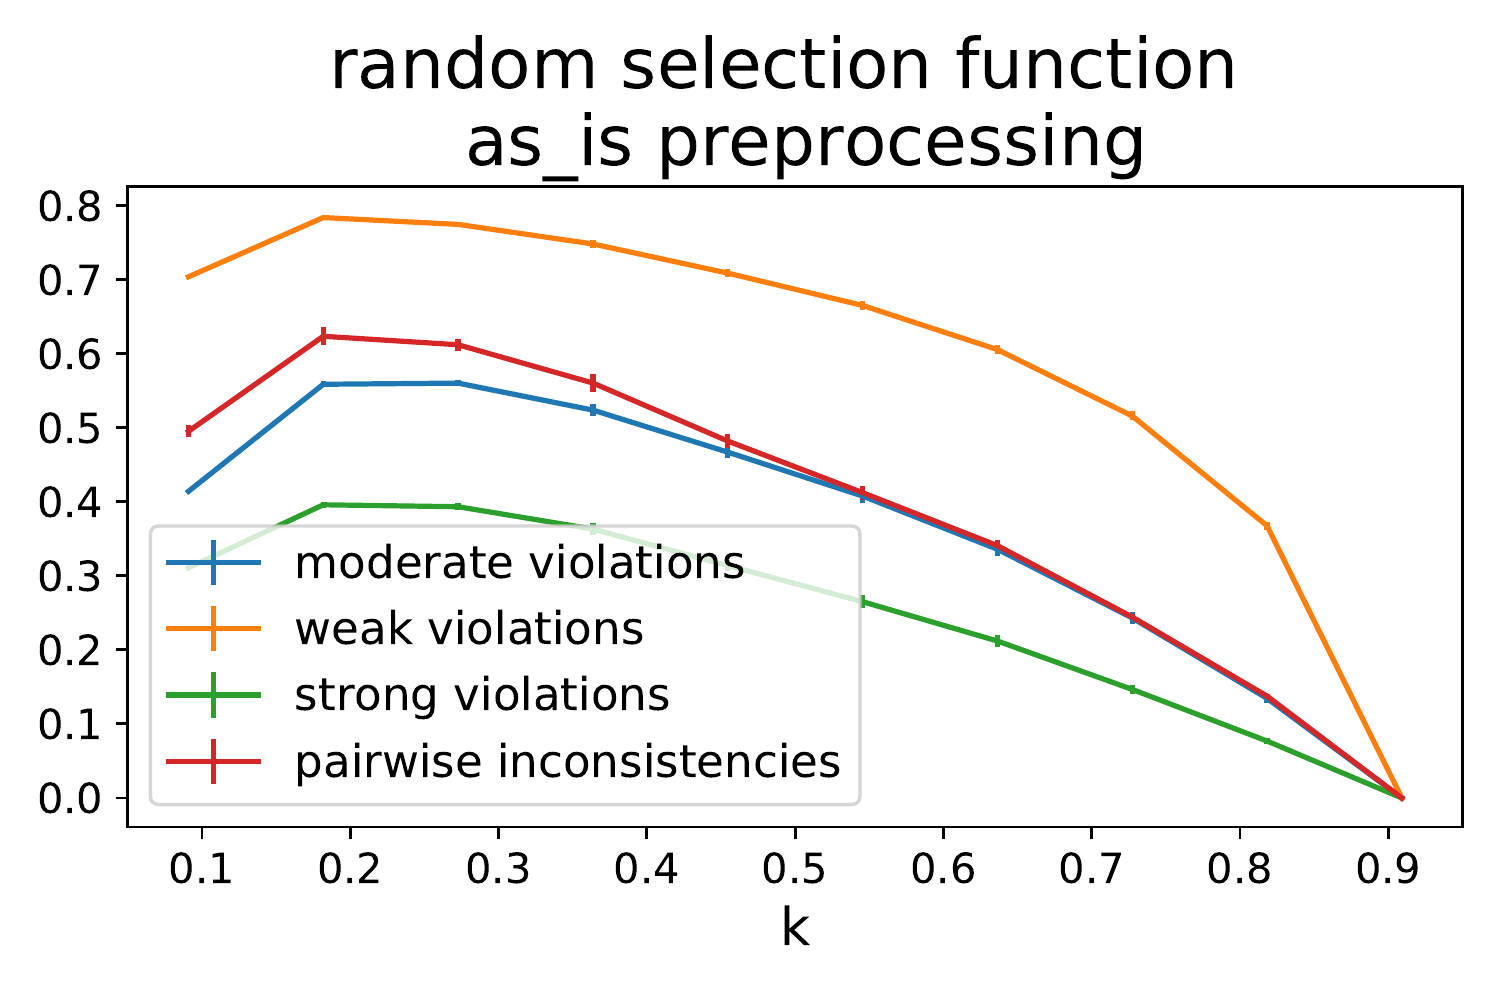}

 \includegraphics[width=8cm]{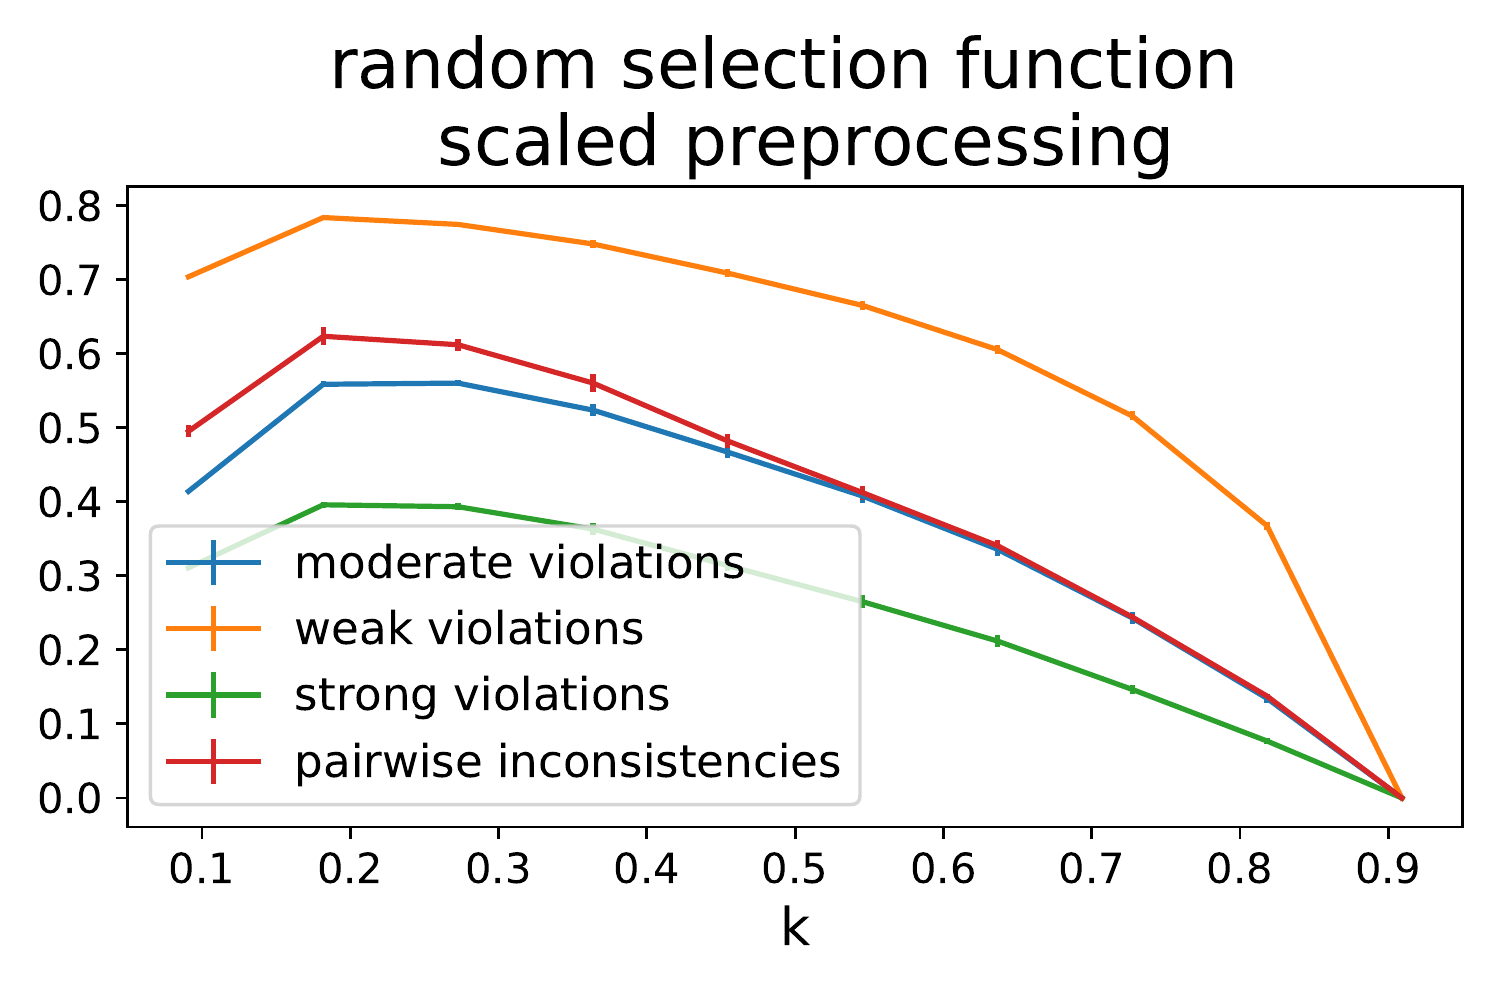}

    \includegraphics[width=8cm]{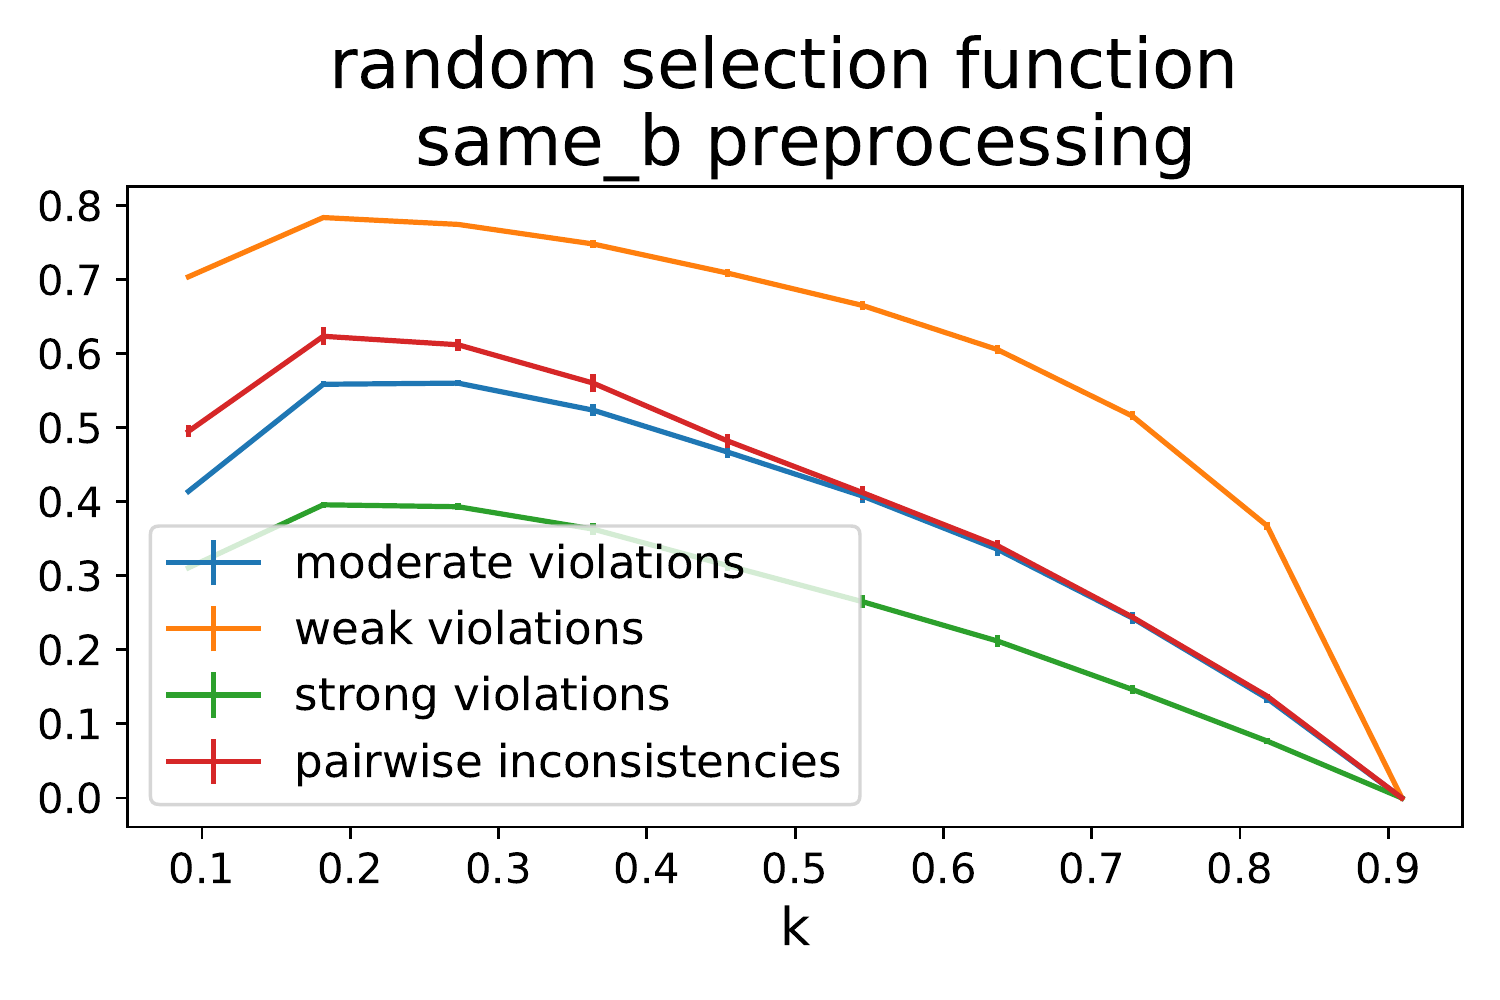}
   
 \includegraphics[width=8cm]{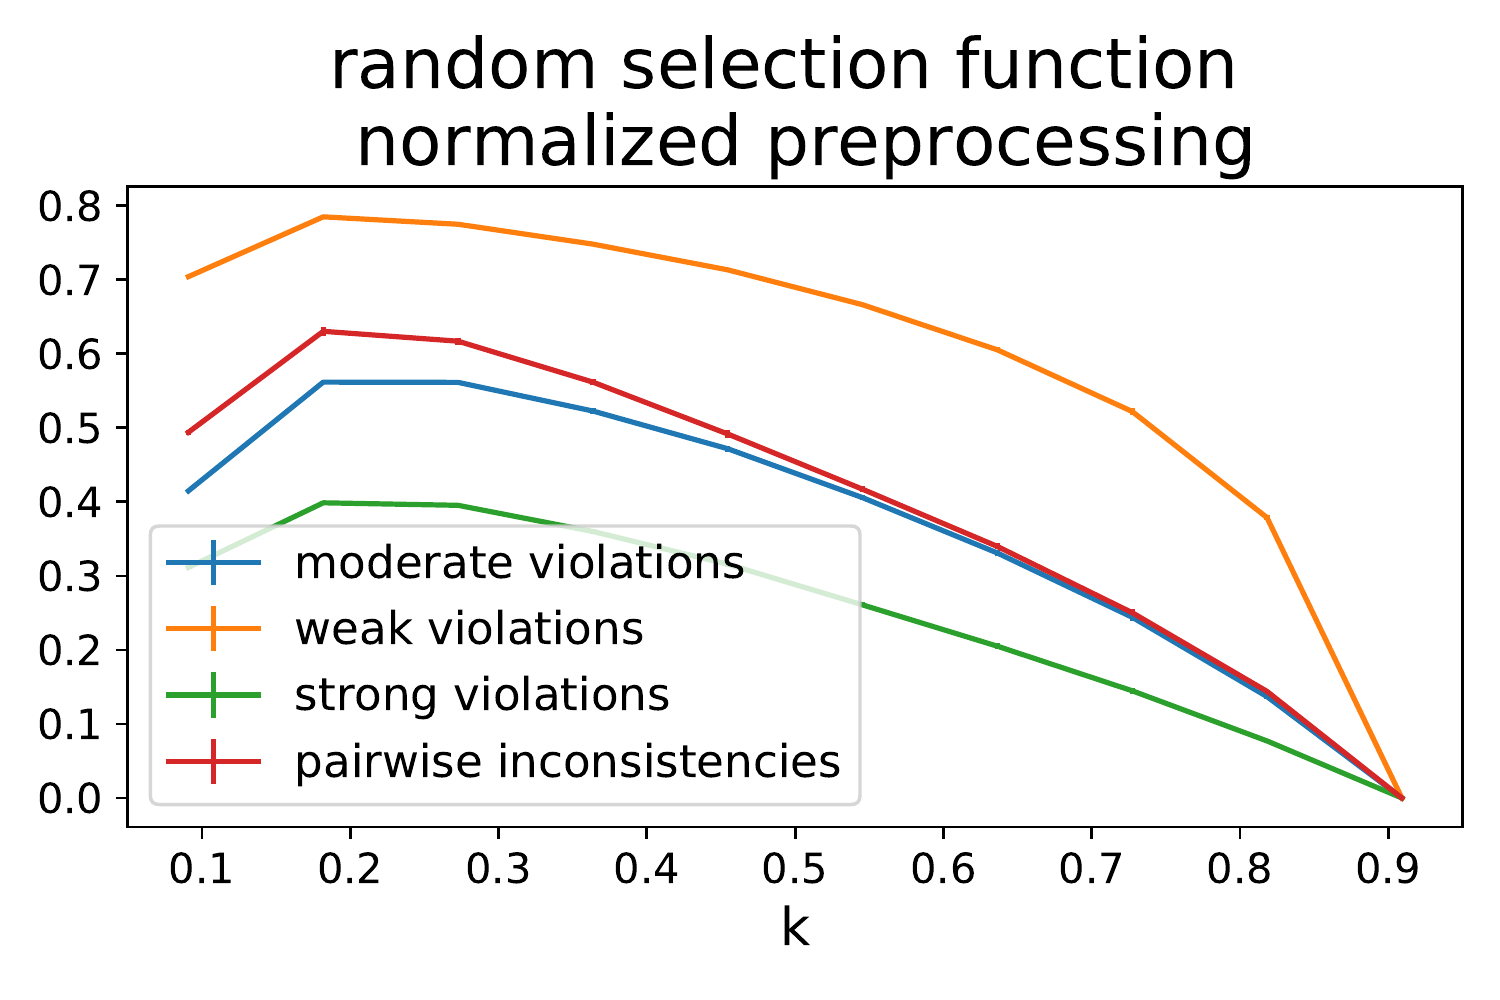}
     \caption{Number of samples and bound for ``random"}
\label{fig:sst, random}
\end{figure}

\begin{figure}
\centering

   \includegraphics[width=8cm]{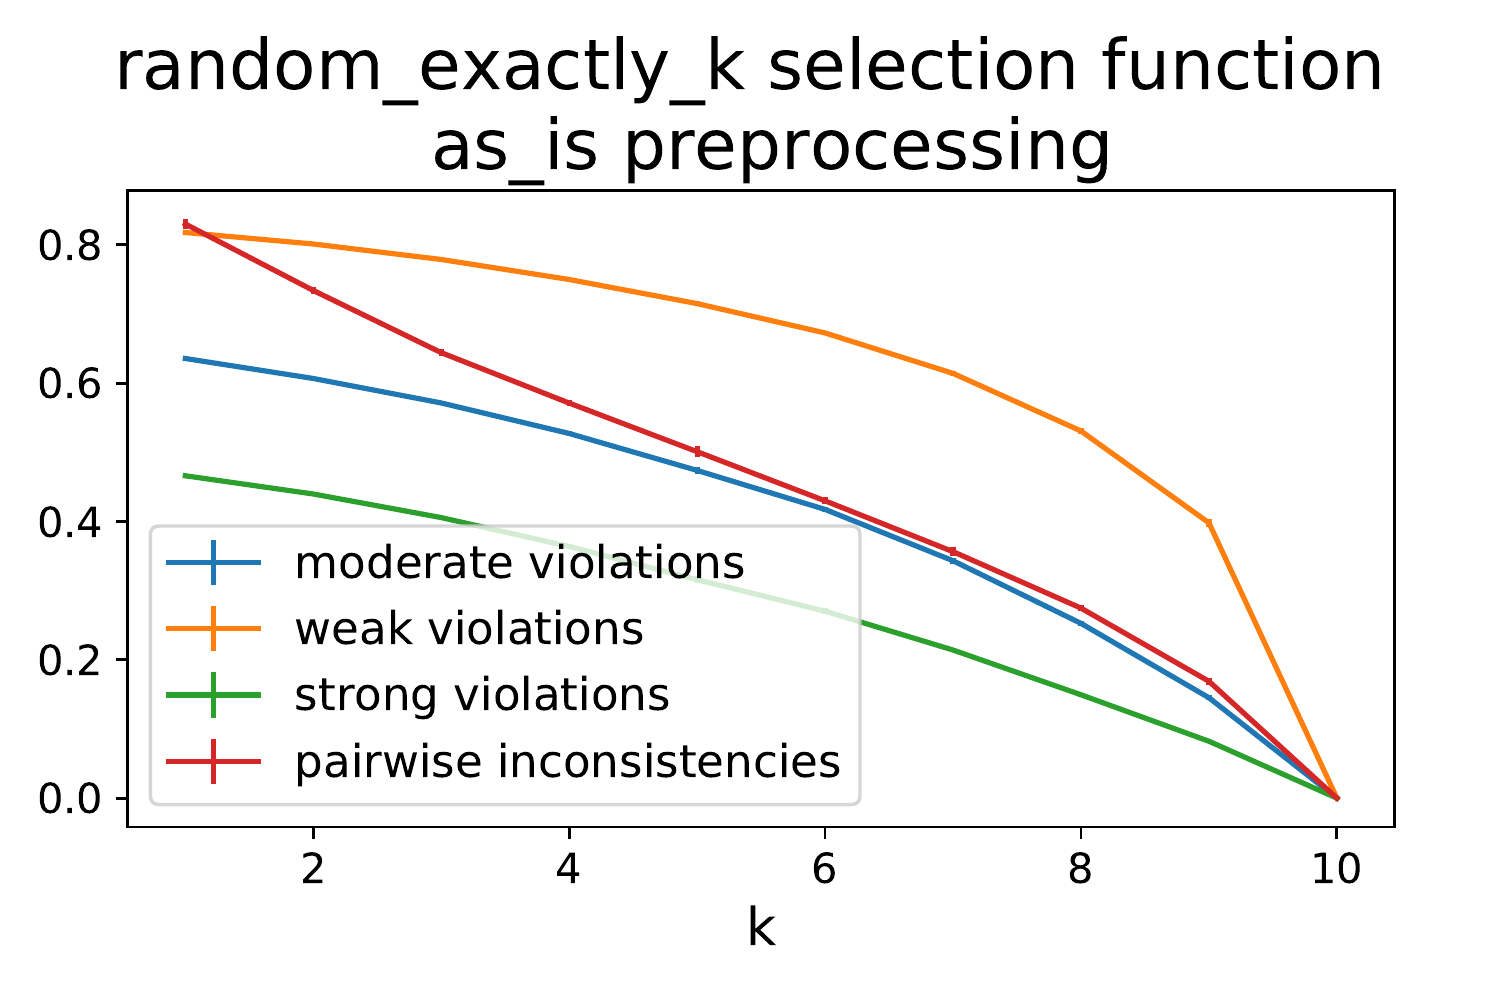}

 \includegraphics[width=8cm]{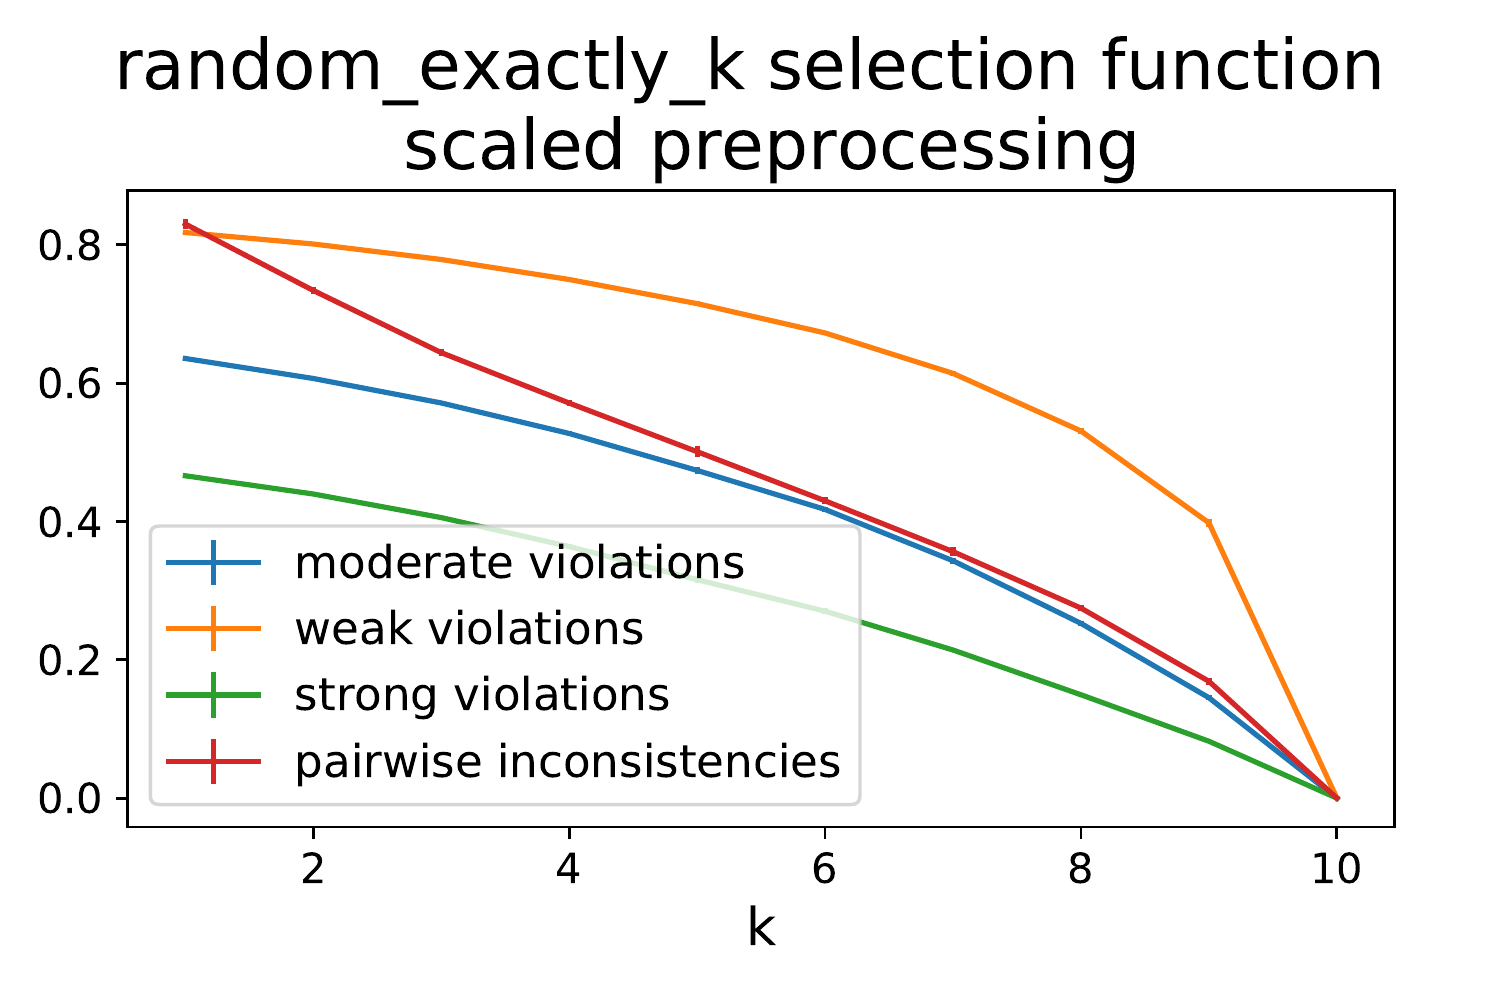}

    \includegraphics[width=8cm]{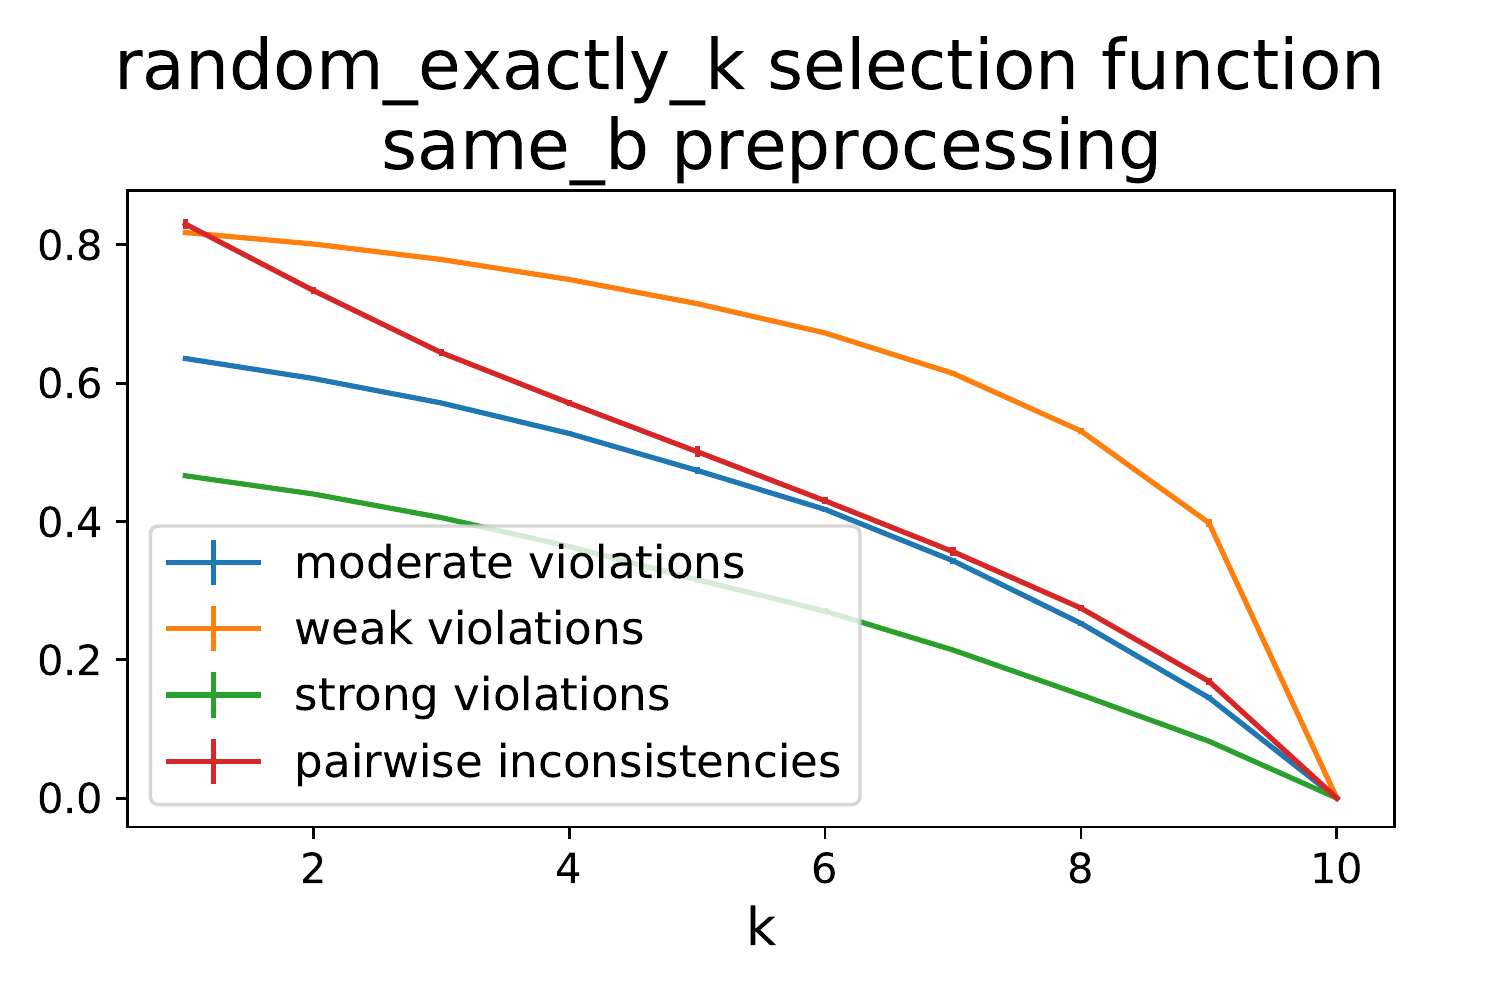}
   
 \includegraphics[width=8cm]{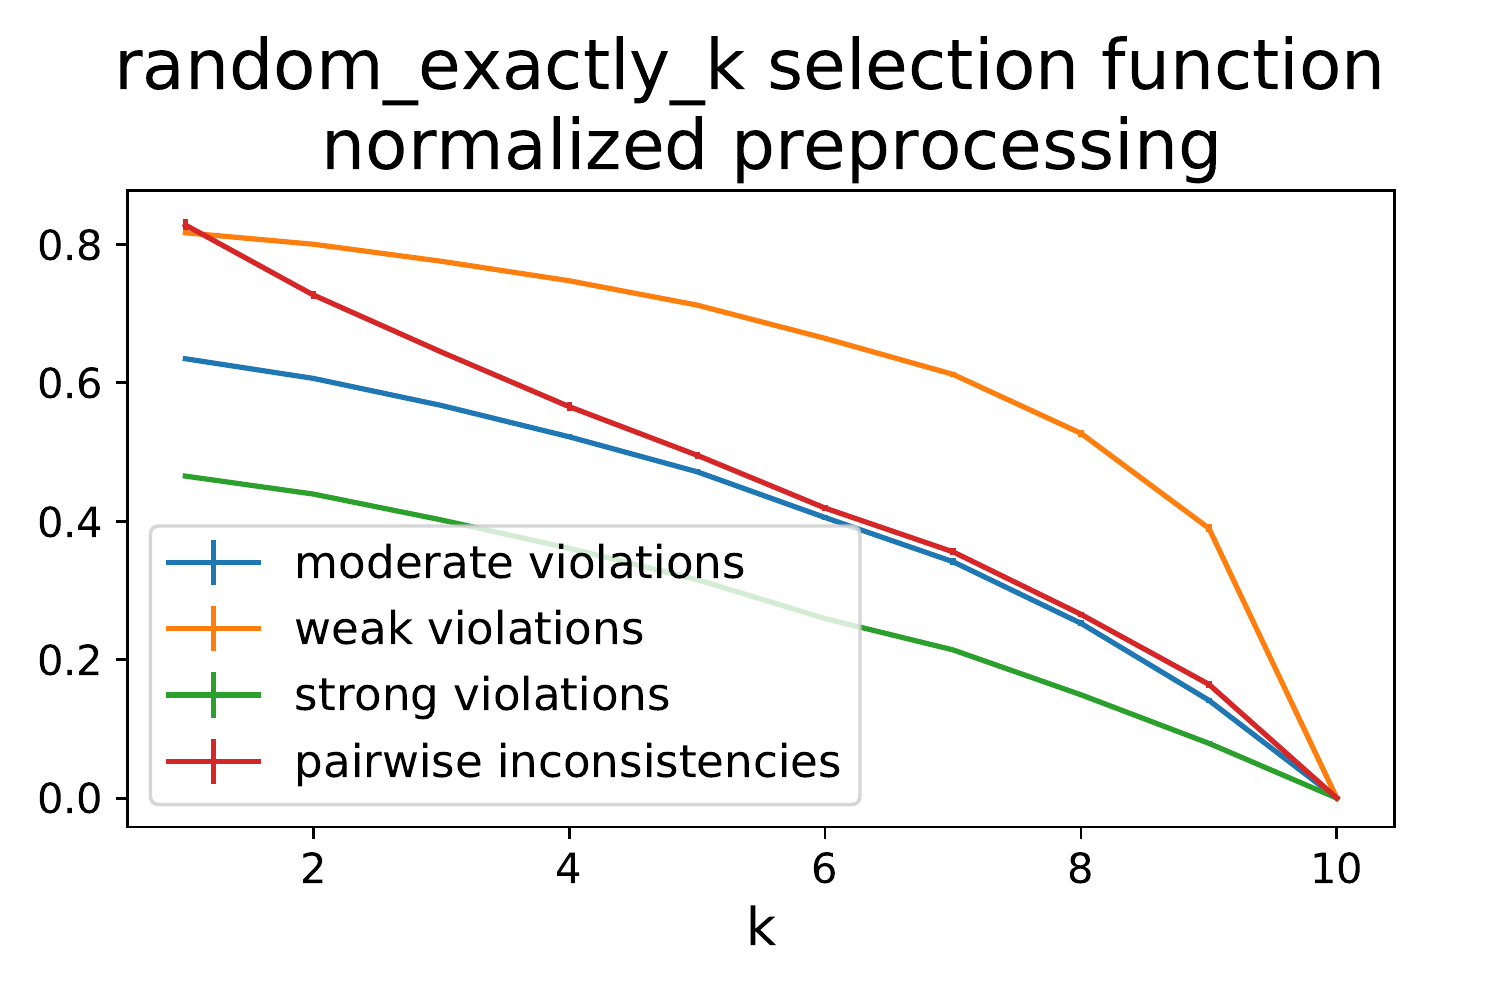}
\caption{Number of samples and bound for ``random exactly $k$"}
\label{fig:sst, random exaclty k}
\end{figure}

\begin{figure}
\centering

   \includegraphics[width=8cm]{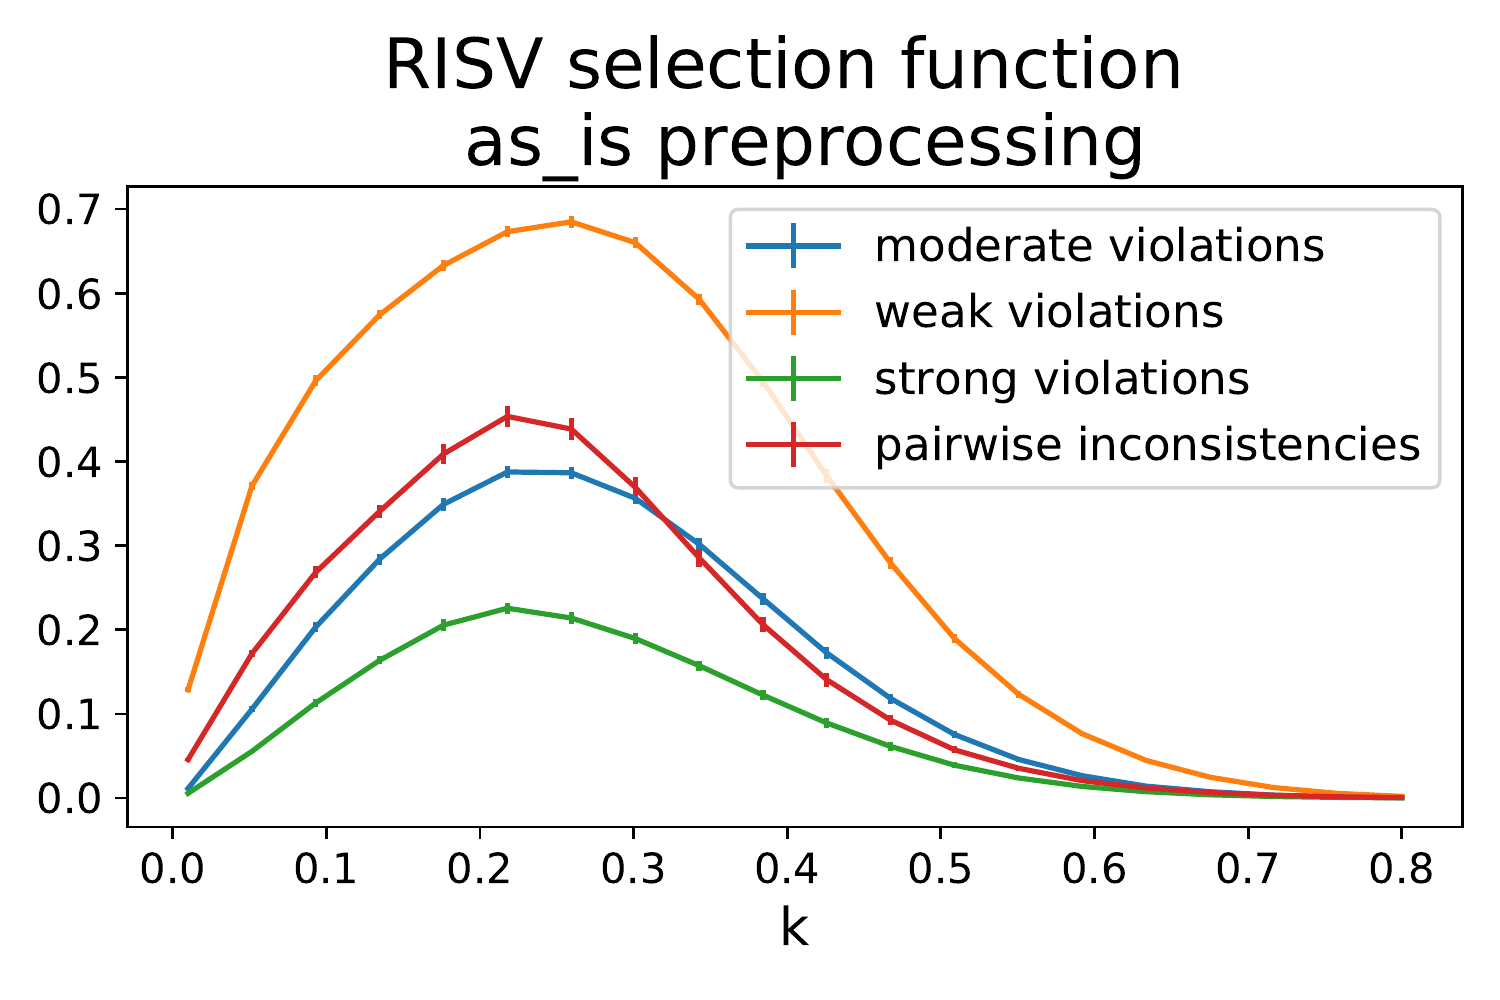}

    \includegraphics[width=8cm]{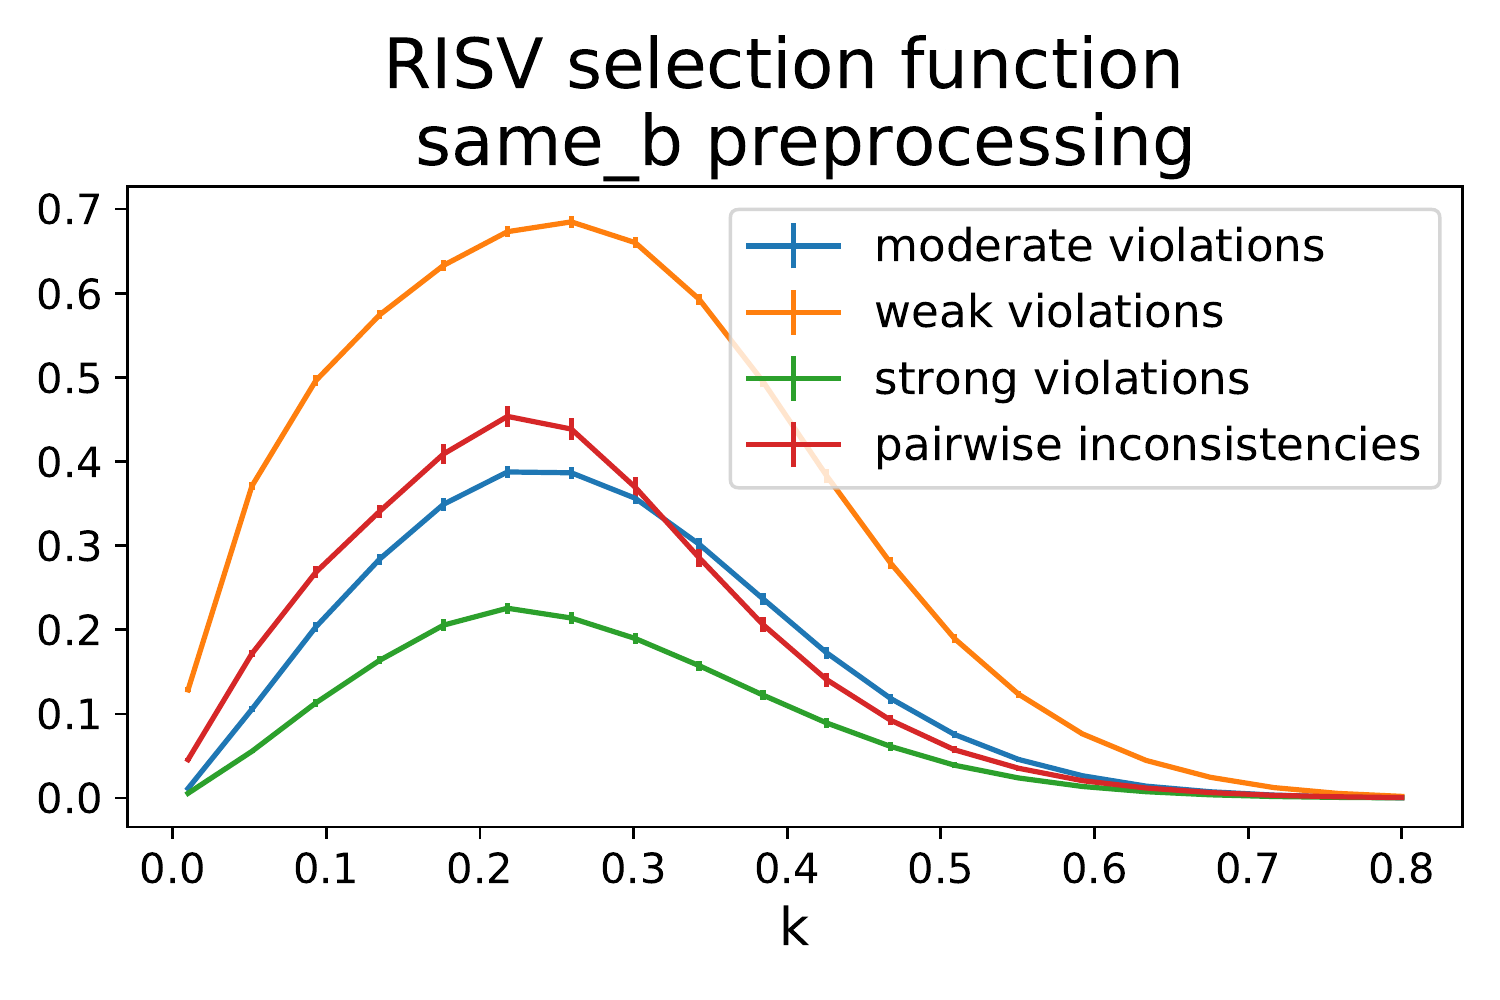}
   
 \includegraphics[width=8cm]{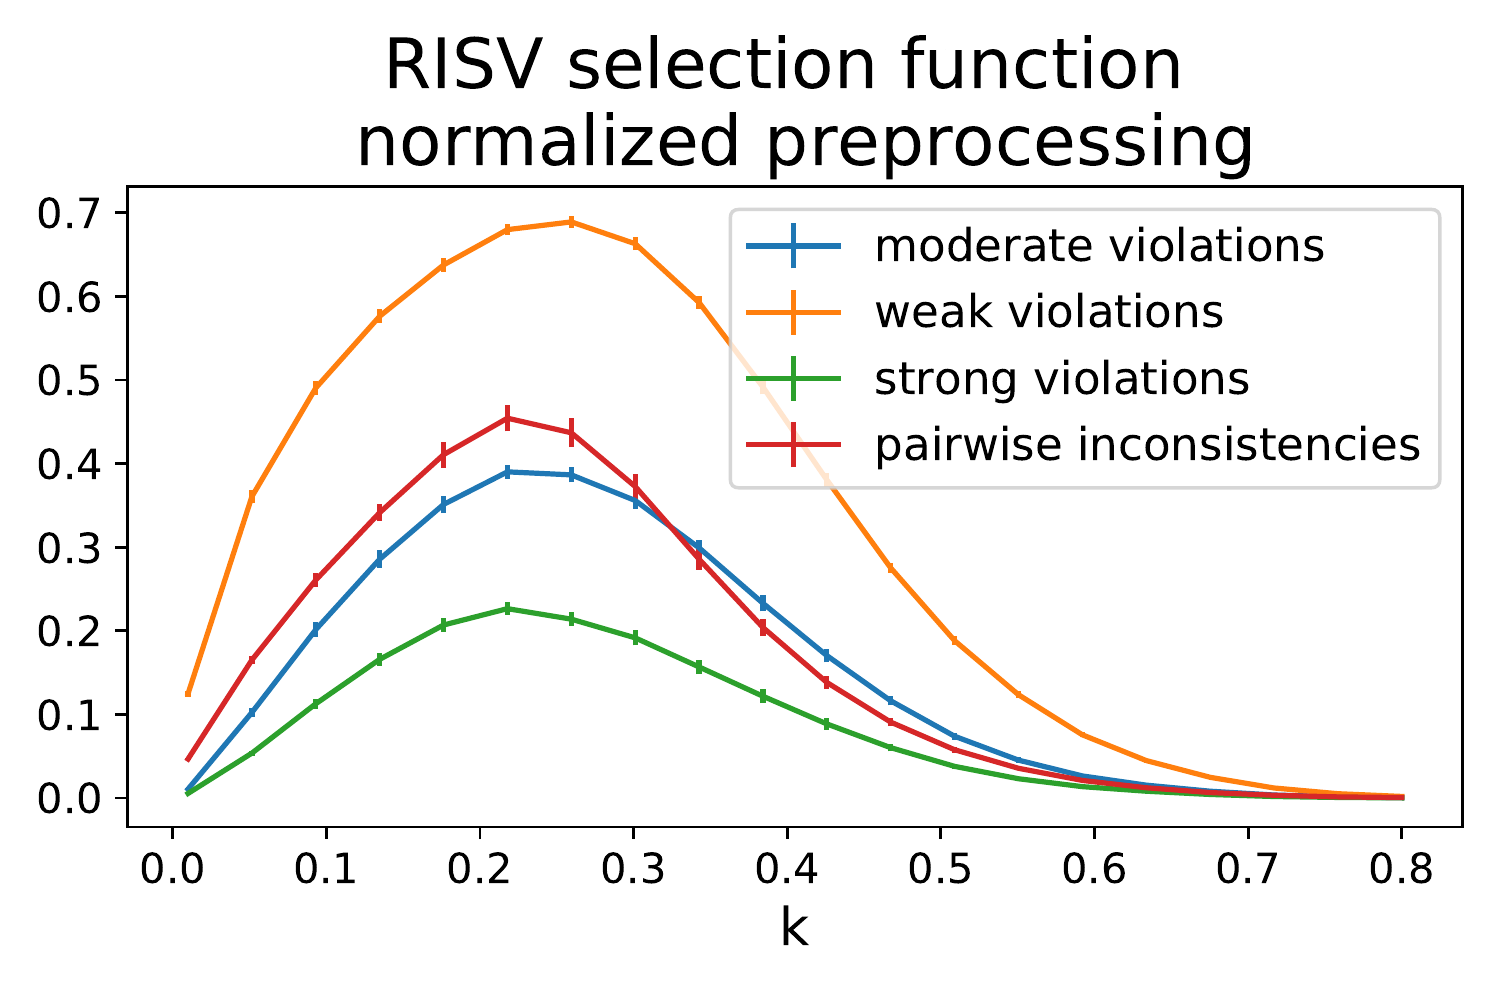}
 \caption{Number of samples and bound for RISV}
\label{fig:sst, risv}
\end{figure}

\begin{figure}
\centering

   \includegraphics[width=8cm]{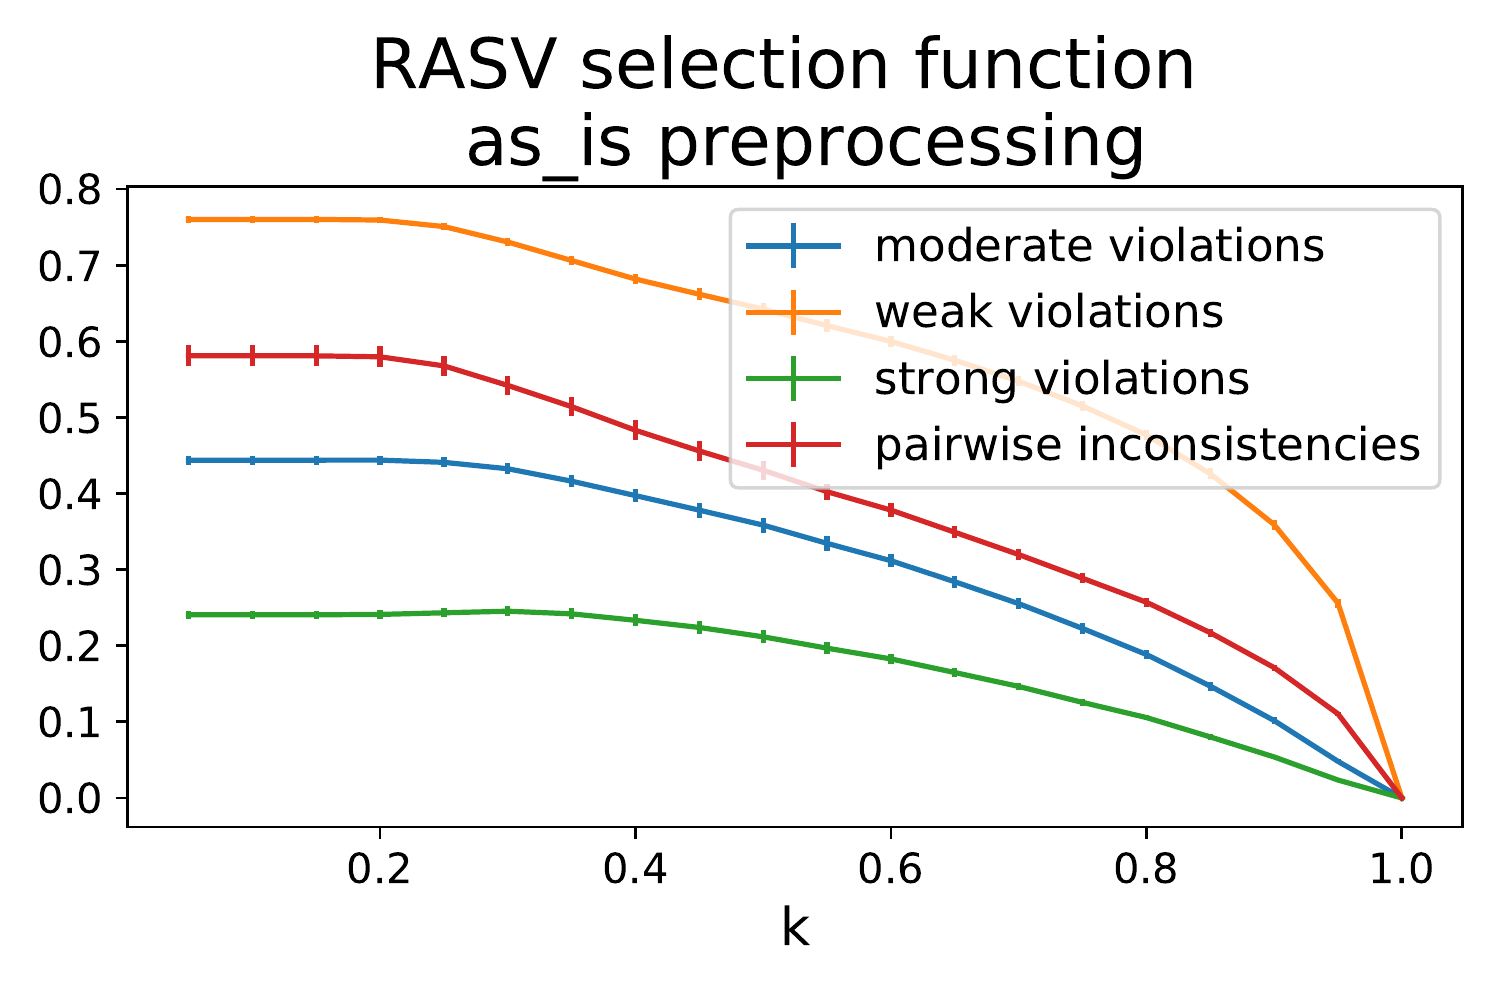}

    \includegraphics[width=8cm]{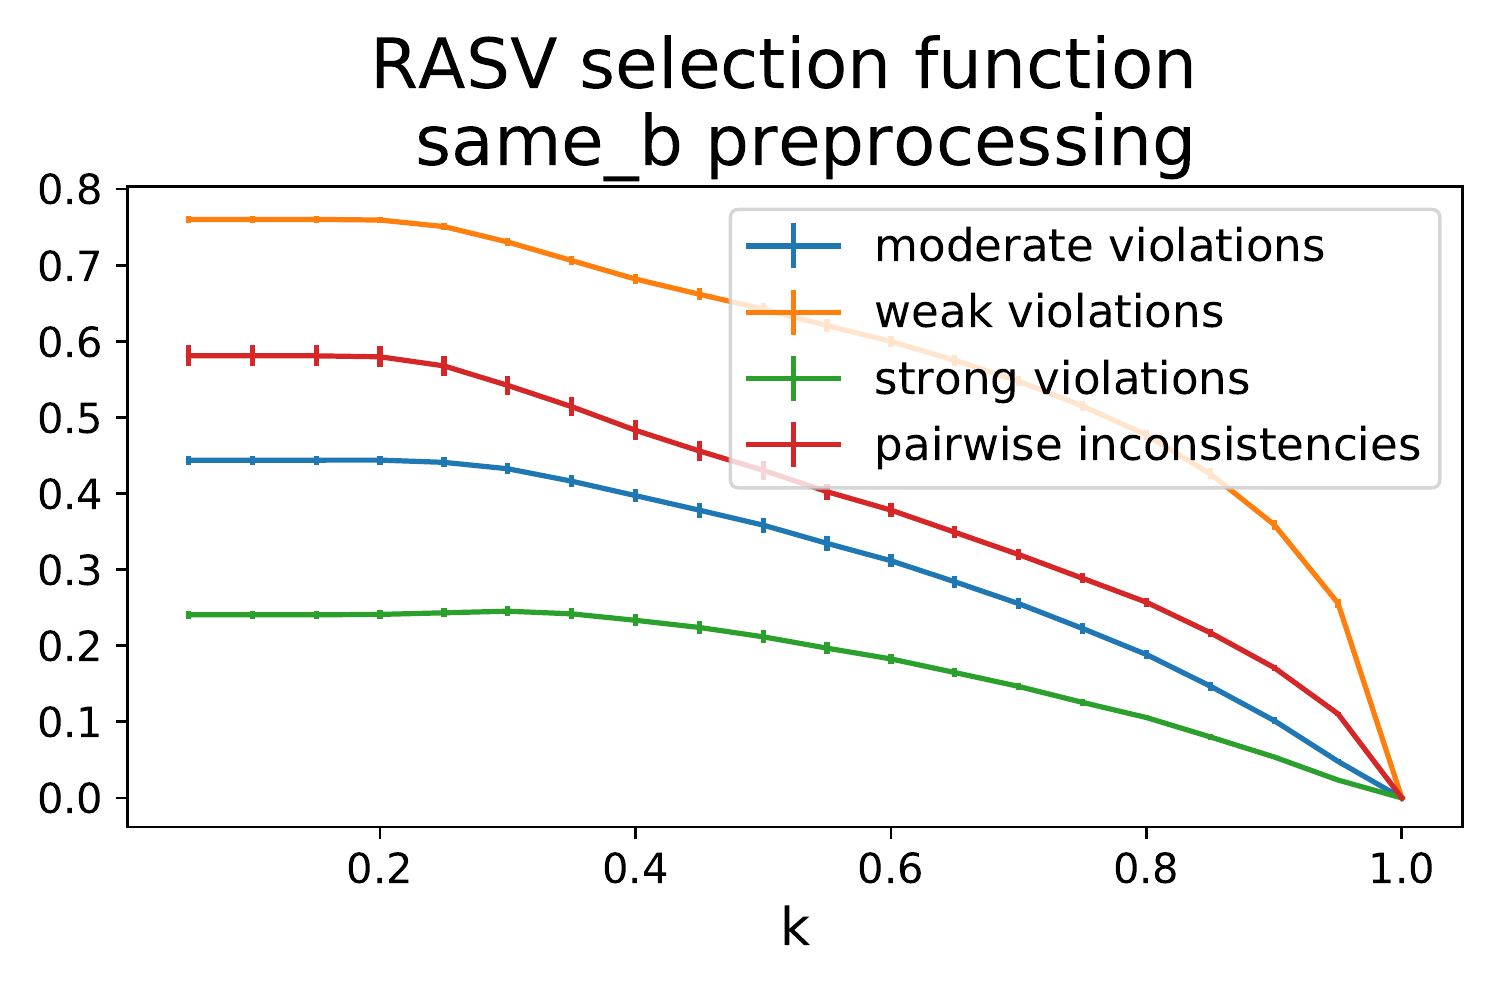}
   
 \includegraphics[width=8cm]{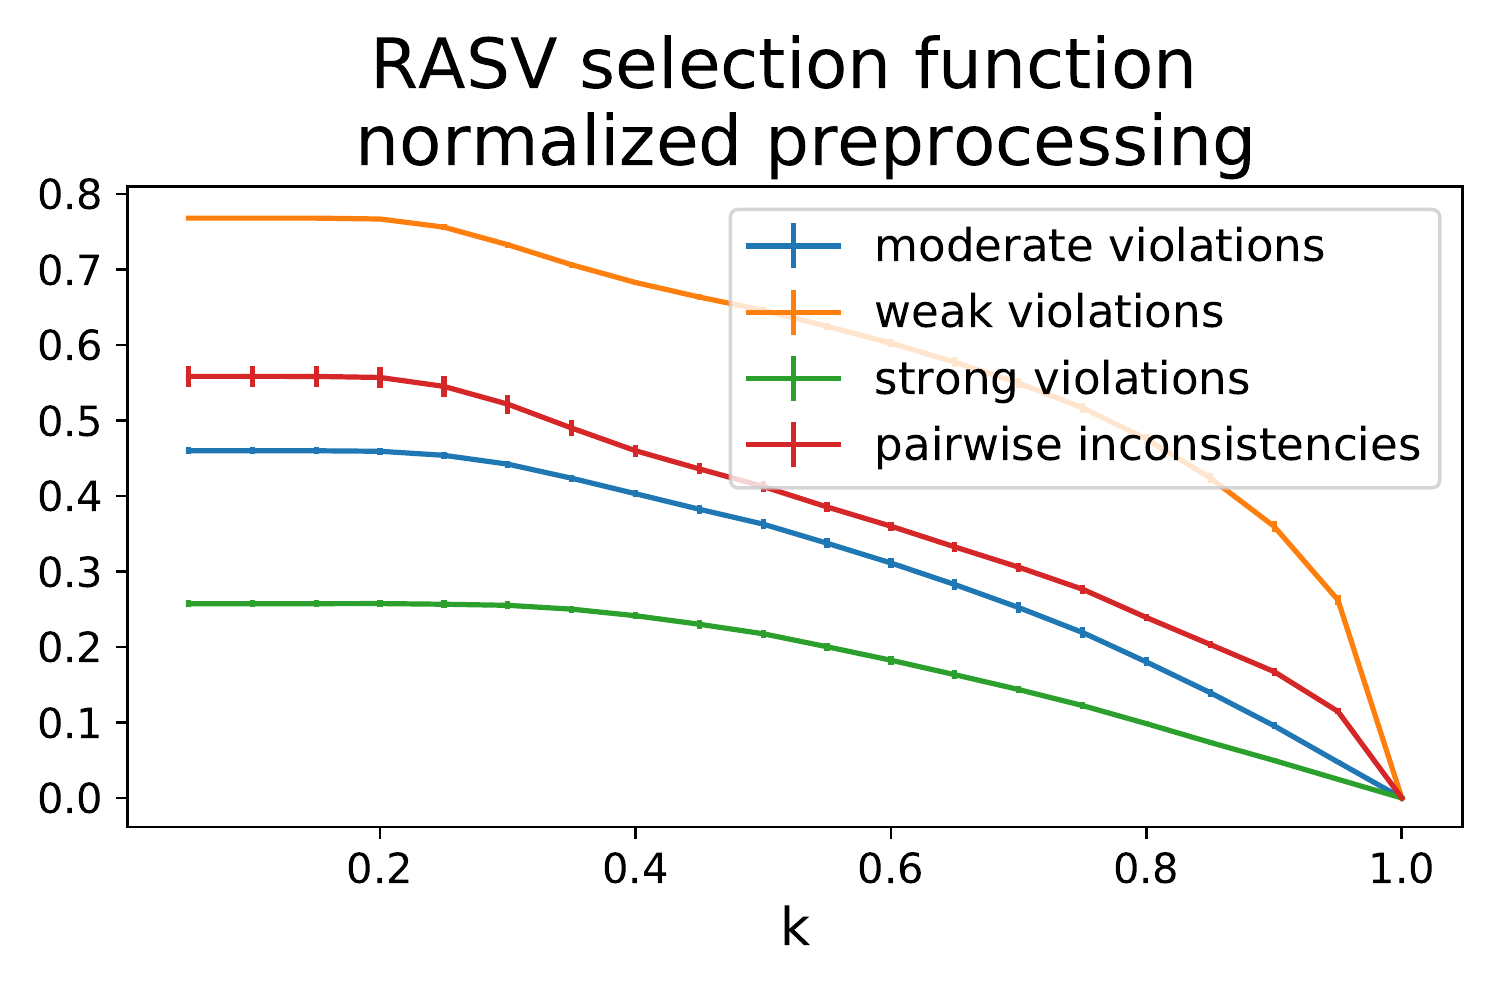}
 \caption{Number of samples and bound for RASV}
\label{fig:sst, rasv}
\end{figure}

Remarks on each pre-processing idea:
\begin{enumerate}
    \item As is: We already discussed why leaving $U$ as is might not be a fair comparison while varying $k$ since the norm of $U_i^{\tau(i,j)}$ changes.
    \item Same b: We are trying to remove the effect of $b^*$. But as shown, the other parameters still change, so maybe this does not really make sense. 
    \item Scaled: It turns out that $b^*$ has a larger range in this case than in the ``as is" case, which is not really what I expected. Perhaps this is because $b^*$ is a sum, and the number of terms in the sum is larger for larger $k$, so maybe a concentration result kicks in where $b^*$ is more controlled for larger $k$. When $k=1$, we are scaling $U$ by $\sqrt{10}$, so we are also scaling $b^*$ by $\sqrt{10}$, so it makes sense that we are making the range of $b^*$ larger. Also, it is not straight forward on how to use this for RASV and RISV.
    \item Normalized: Doesn't really behave differently than ``as is." The same problem as in ``as is" remain, i.e. the norms of $U_i^{\tau(i,j)}$ change. We also cannot normalize $U_i^{\tau(i,j)}$, since any pre-processing operation should be done on the entire matrix $U$, not on the masked versions of $U_i$ given by $\tau$.
\end{enumerate}

All selections functions produce intransitivities and pairwise inconsistencies.

The shape of $m_1$ changes for different pre-processing choices, i.e. it could be increasing, decreasing, or constant. With the dimension $d$ fixed, $m_1$ is just a function of $\beta$. Multiplying $U$ by $\alpha$ also scales $\beta$ by $\alpha$. Therefore, for ``scaled" pre-processing $m_1$ is significantly bigger than the ``as is" case since for any $k$, we are scaling $U$ by $\frac{\sqrt{d}}{\sqrt{k}} > 1$. However, $m_1 << m_2$ so $m_1$ is almost insignificant.

The shape of $m_2$ remains the same after pre-processing. In the case where $U$ is multiplied by a scalar, like in ``same $b$" and ``scaled", this makes sense since if we scale $U$ by $\alpha$, we scale $\eta$ by $\alpha^4$, $\lambda$ by $\alpha^2$, and $R$ by $\alpha^2$. Therefore $m_2$ is invariant to scaling $U$ by $\alpha$ since $m_2 = \frac{8\log(d)(6\eta + \lambda R)}{3\lambda^2} = \frac{8\log (d)(6\alpha^4\eta + (\alpha^2\lambda) (\alpha^2 R))}{3(\alpha^2\lambda)^2}$. 

For ``scaled" pre-processing, the upper bound is significantly larger compared to ``as is" because of the increase in $b^*$. The upper bound is \[ \frac{4(1 + \exp(b^*))^2}{\exp(b^*)\lambda}  \sqrt{\frac{3\beta^2\log{(2d^2)}d + 4\sqrt{d}\beta \log{(2d^2)}}{6}},\] so when $U$ is scaled by $\alpha$, the upper bound becomes 
\begin{align} 
\frac{4(1 + \exp(\alpha b^*))^2}{\exp(\alpha b^*)(\alpha^2 \lambda)}  \sqrt{\frac{3(\alpha \beta)^2\log{(2d^2)}d + 4\sqrt{d}(\alpha) \beta \log{(2d^2)}}{6}} \leq \frac{4(1 + \exp(\alpha b^*))^2}{\exp(\alpha b^*)\alpha \lambda}  \sqrt{\frac{6 \beta\log{(2d^2)}d \log{(2d^2)}}{6}},
\end{align}
so the upper bound changes because of the $\frac{4(1 + \exp(\alpha b^*))^2}{\exp(\alpha b^*)\alpha}$ term. Furthermore, this shows why in the ``same $b$" preprocessing, the bound does not change much since $b^* =1$, so the only difference in the upper bound versus the ``as is" case is $\frac{1}{\alpha}$.

% The general upper bound typically remain the same after preprocessing and under the different selection functions except for RASV with normalized preprocessing and ``top $k$" where the upper bound for ``as is" and ``same b" tend to remain constant after $k=2$ compared to scaled and normalized preprocessing. 

% The overall number of samples and bound tend to increase for scaled preprocessing. One reason is because the maximum and range of $\beta$ significantly increases which suggests

Originally, we wanted to say something about $\lambda$. However, it does not make sense to isolate just $\lambda$ without considering the other terms. Furthermore, $m_1$, $m_2$, and the bound is what we ultimately care about. These plots suggest that the smallest number of samples we need to use Theorem \ref{thm:sampleComplexity} is not when $k=1$ or $k=10$, but somewhere in between. However, the smallest upper bound occurs when $k=10$.

After running these experiments and thinking about preprocessing, I'm also inclined to ditch RASV/RISV for ``top k" and ``random" since (1) thinking about ``top k" is easier and simpler, (2) Proposition \ref{prop:MaxCoordProp} could be about ``top k" when $k=1$, and (3) we might end up putting in a theoretical result about ``random." However, I do not know yet which selection functions work better on real data. ``Random" definitely cannot be used on real data, but I still think conceptually it's interesting for theoretical analysis.
