# Supplementary material for: Preference Modeling with Context-Dependent Salient Features
Source: arXiv:2002.09615 source file (2020-06-27)
Supplement: Supplementary file 2 [file synthetic_exp.tex]

\subsection{Additional plot for the salient feature preference model under RASV}

Since the salient feature preference model only uses some features for each pairwise comparison, Figure \ref{fig:avg_h_RASV} shows how many features on average are used by each pairwise comparison under the same experiment from Section \ref{sec:experiments}. Other than when the threshold is 1, no sampled pairwise comparison utilizes all the features in the resulting utilities, i.e. $\tau(i,j) \neq [d].$ As one might expect, contrasting Figure \ref{fig:avg_h_RASV} with Figures \ref{fig:syntheticExperiments} and \ref{fig:propsRASV}, shows that in the regime where only a few features are used is where the most intransitives and inconsistencies with the underlying ranking arise and where more samples are required for learning $w^*$.

\begin{figure}
    \centering
    \includegraphics[width=8cm]{synthetic_experiment_figs/avg_h_threshold_sweep_RASV.pdf}
    \caption{Under the salient feature preference model with the RASV selection function, we plot how many features on average are used in a pairwise comparison given the threshold. As one might expect, less features used on average translates to higher intransitivity rates and pairwise inconsistency rates.}%
    \label{fig:avg_h_RASV}%
\end{figure}

% First, our salient feature preference model can result in pairwise comparisons that are inconsistent with the underlying true ranking. Consider items $\{i,j\}$ such that $\langle U_{i} - U_{j}, w^* \rangle < 0$, meaning item $i$ is lower than item $j$ in a full ranking using all features. This pair may be such that $\langle U_{i}^{\tau(\{i,j\})} - U_{j}^{\tau(\{i,j\})}, w^* \rangle >0$ meaning item $i$ beats item $j$ on average when compared in isolation from the other items. See the first plot in Figure \ref{fig:syntheticExperiments}, which shows what percentage of pairwise comparisons of all pairwise comparisons disagree with the underlying true ranking. Preferences arising from the standard BTL model cannot be inconsistent with the underlying ranking. Therefore, the pairwise inconsistency rate affects the quality of the learned ranking under the BTL MLE.

% Second, Figure \ref{fig:syntheticExperiments} also shows the low noise violation rate which is the fraction of pairs for which the low noise condition does not hold. The low noise condition is a property of the underlying pairwise probabilities and is defined as the following implication: if for any pair of items $(i,j)$ $P_{ij} > .5$, then $\sum_{k} P_{ki} > \sum_{k} P_{kj}$. The low noise condition is a sufficient condition for the MLE of the BTL without features model to produce a ranking that minimizes the number of pairs that disagree with the underlying ranking \cite{rajkumar2016can}.

\subsection{Synthetic experiments for the salient feature preference model under RISV}
We repeat the same experiments but for the salient feature preference feature model with the RISV selection function. We only increase the threshold until $t = .6$ because around this threshold, the salient feature preference model and the BTL model are identical. See Figure \ref{fig:w_KT_threshold_sweep_individual} which again illustrates the gap between the estimation error for $w*$ and learning a ranking for the MLE of the BTL model and the MLE of the salient feature preference model.

\begin{figure}
    \centering
    \includegraphics[width=12cm]{synthetic_experiment_figs/w_KT_indv.pdf}
    \caption{The estimation error of $w^*$ and the Kendall tau correlation between the estimated ranking the true ranking for both the BTL and threshold preference model with the RISV selection function.}%
    \label{fig:w_KT_threshold_sweep_individual}%
\end{figure}

See Figure \ref{fig:prop_individual} for plots about the behavior of the resulting pairwise comparisons. This model also produces pairwise comparisons that are intransitive and that are inconsistent with the underlying ranking, both of which must be satisfied by pairwise comparisons generated by the BTL model. Unlike the plot for the RASV selection function, the average number of features used in a pairwise comparison is reported for pairs that do not use all the features. Because for some pairs the RISV selection function returns all the features, we also show the percentage of the 10,000 pairwise comparison samples that utilize all the features.

\begin{figure}
    \centering
    \includegraphics[width=13
    cm]{synthetic_experiment_figs/props_indv.pdf}
    \caption{The affect of varying the threshold on properties of the pairwise comparisons with the RISV selection function.}%
    \label{fig:prop_individual}%
\end{figure}

We also illustrate Theorem \ref{thm:sampleComplexity} for the RISV selection function under the same set-up as the corresponding experiments for the RASV selection function in Section \ref{sec:experiments} except we fix the threshold at $t=.15$. See Figure \ref{fig:thmIllustrationIndiv}.

\begin{figure}%
    \centering
    \includegraphics[width=9cm]{synthetic_experiment_figs/w_error_threshold_individual.pdf} 
  \caption{Illustration of Theorem \ref{thm:sampleComplexity} under the RISV selection function.}%
    \label{fig:thmIllustrationIndiv}%
\end{figure}
