# Supplementary material for: Preference Modeling with Context-Dependent Salient Features
Source: arXiv:2002.09615 source file (2020-06-27)
Supplement: Supplementary file 3 [file ideas.tex]

what about when orthogonal matrices so min eigenvalue is 1
what about non-overlapping selection function
is this minimax optimal?

write down:
-btl model not identifiable and why. and where in the proof things change, but that the bounds match.

pros:
-emphasize that you can get intransitivities out of this model
-compared to other models, we are using features and we have a ranking
-in contrast to that work, we provide a convex intransitivity model.
-dealing with intransitivties is harder.
-what's interesting is how do you deal with intransitivties. something like rank centrality won't work. or will it work so long as the intransitivties are not too bad?
-how does sample complexity compared to just using pairwise comparisons with no features? i guess in the f-btl paper they say they can do better than n log n

experiments:
-show intransitivity makes lambda worse and conclude that intransitivties makes learning harder
- how many samples do you need to attain a certain error and say its harder for intransitive data

-----------
Minimax lower bounds
Max coord with gaussian (what does a thm statement even look like)
