# Supplementary material for: Preference Modeling with Context-Dependent Salient Features
Source: arXiv:2002.09615 source file (2020-06-27)
Supplement: Supplementary file 4 [file intransitivity.tex]

\begin{table*}
  \centering

  \begin{tabular}{lllllllll}
    \toprule
    \cmidrule(r){1-2}
Data Set &  Items & Match-ups  & Unique Pairs & Valid Triplets & Strong Violations & Moderate Violations & Weak Violations \\
    \midrule

NBA 2014 & 30 & 481 & 339 & 1853 & 778 & 776 & 522 \\
NBA 2015 & 30 & 1238 & 430 & 3198 & 1983 & 1729 & 816  \\
NBA 2016 & 30 & 1247 & 421 & 2877 & 1733 & 1474 & 654   \\
NBA 2017 & 30 & 1268 & 423 & 2967 & 2016 & 1678 & 762  \\
NBA 2018 & 30 & 686 & 372 & 1998 & 968 & 926 & 414 \\
District & 122 & 5150 & 94 & 48 & 18 & 3 & 0 \\
Car & 10  & 45 & 2973 & 120 & 46 & 7 & 0 \\
    \bottomrule
  \end{tabular}
\end{table*}

%https://www.kaggle.com/ionaskel/nba-games-stats-from-2014-to-2018
% car: http://users.cecs.anu.edu.au/~u4940058/CarPreferences.html
