# Supplementary material for: Preference Modeling with Context-Dependent Salient Features
Source: arXiv:2002.09615 source file (2020-06-27)
Supplement: Supplementary file 5 [file latexmkrc.tex]

add_cus_dep( 'tex', 'aux', 0, 'makeexternaldocument' );
 
sub makeexternaldocument {
    if (!($root_filename eq $_[0]))
    {
        system( "latexmk -pdf \"$_[0]\"" );
    }
}
